# Supplementary material for: Estimating sex and age for forensic applications using machine learning based on facial measurements from frontal cephalometric landmarks
Source: arXiv:1908.02353 source file (2019-08-06)

# Distributions of PAI\_0 by Sex and Age

ages from 5 years to 22 years old

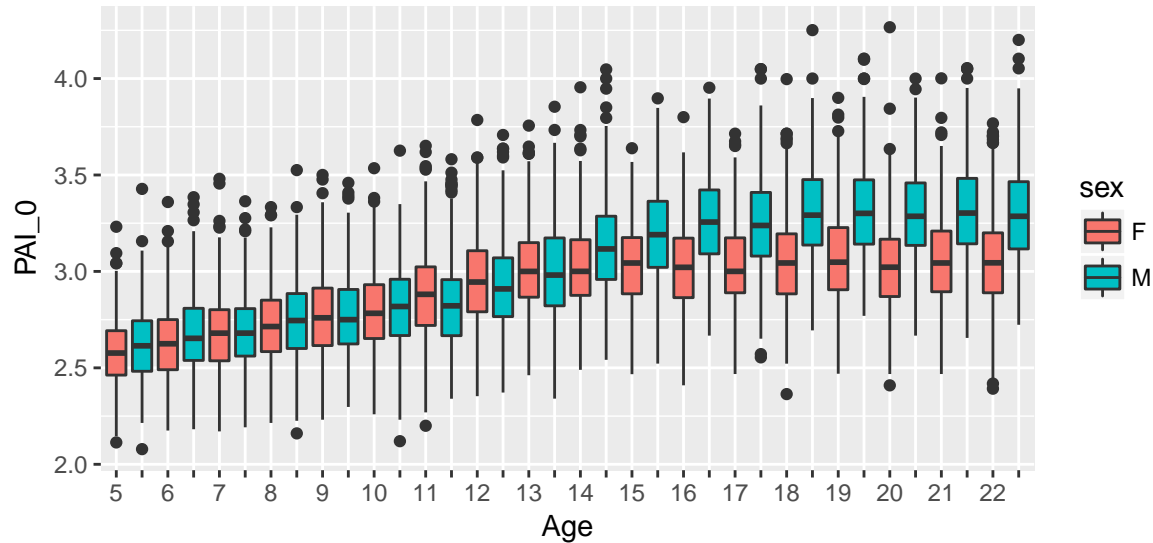

# Distributions of PAI\_100 by Sex and Age

ages from 5 years to 22 years old

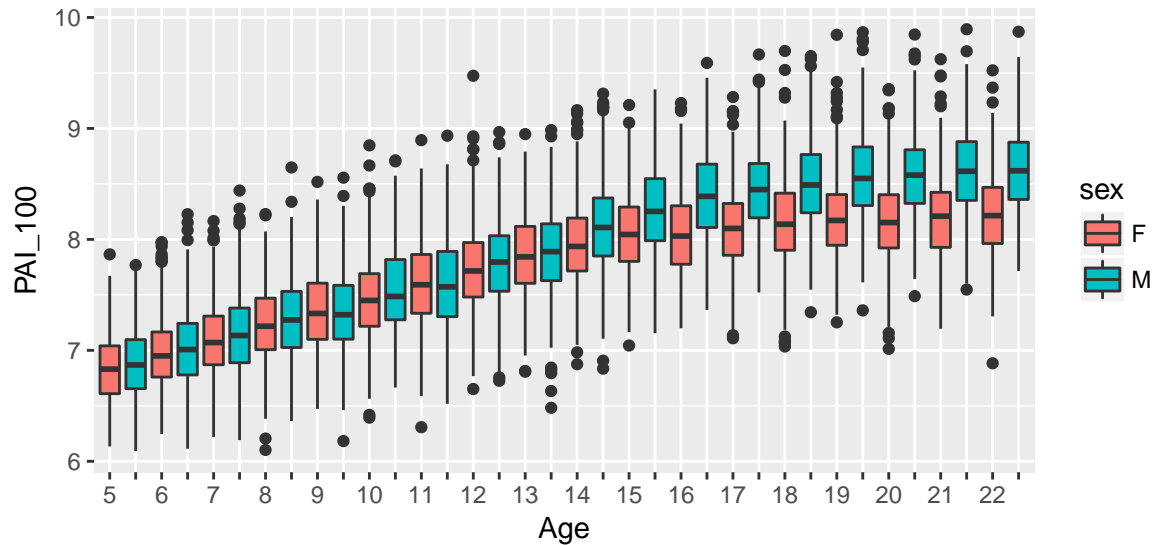

# Distributions of PAI\_101 by Sex and Age

ages from 5 years to 22 years old

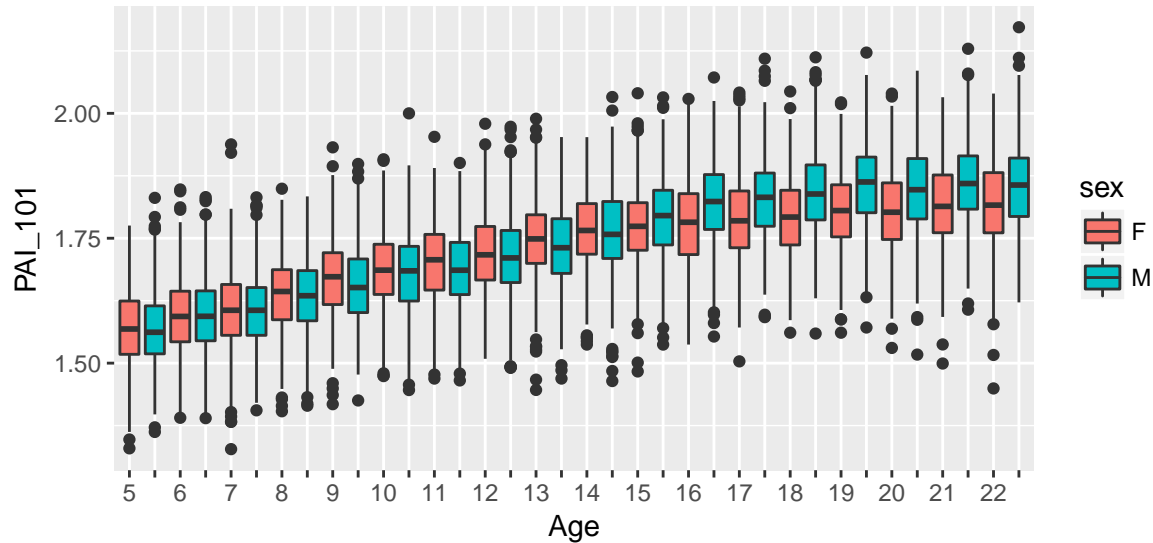

# Distributions of PAI\_102 by Sex and Age

ages from 5 years to 22 years old

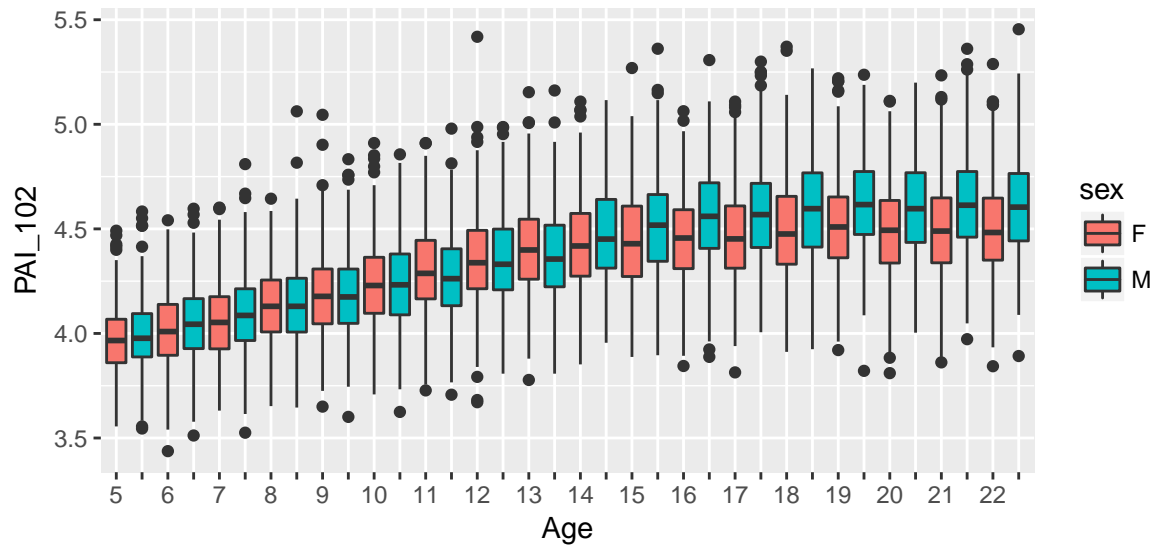

# Distributions of PAI\_103 by Sex and Age

ages from 5 years to 22 years old

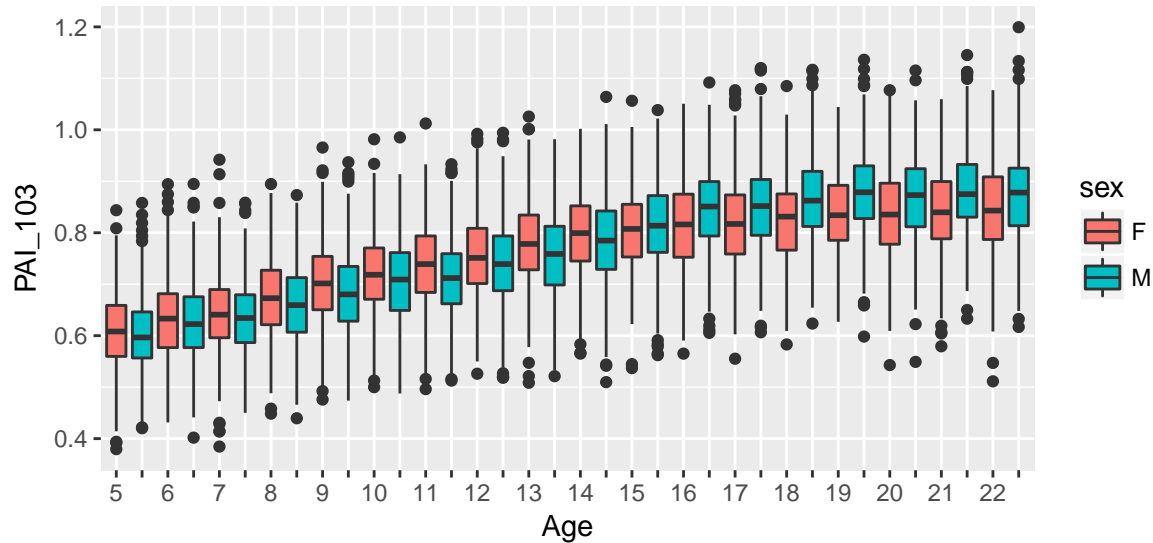

# Distributions of PAI\_104 by Sex and Age

ages from 5 years to 22 years old

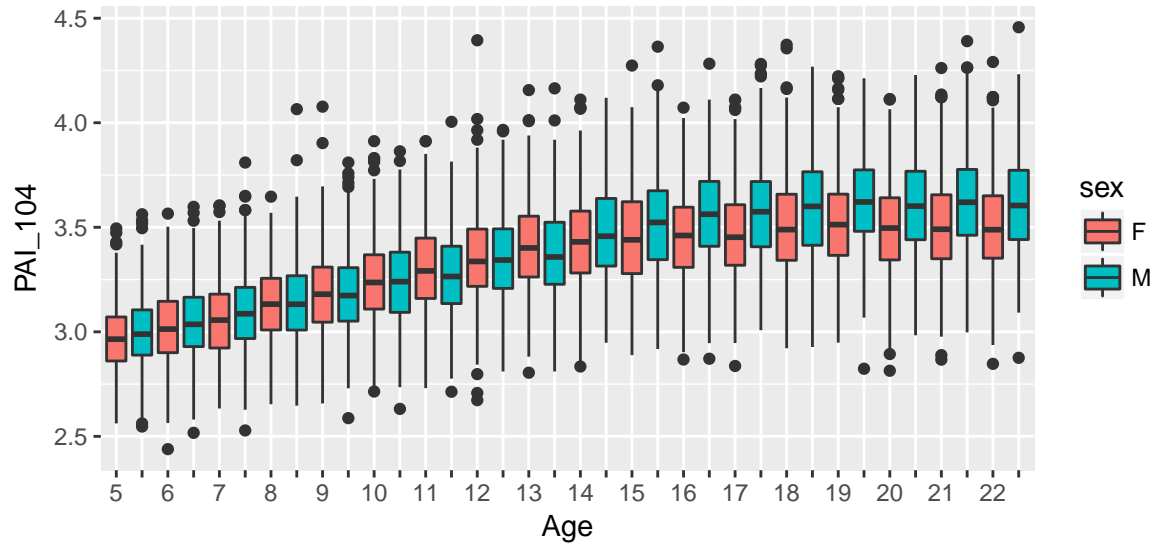

# Distributions of PAI\_105 by Sex and Age

ages from 5 years to 22 years old

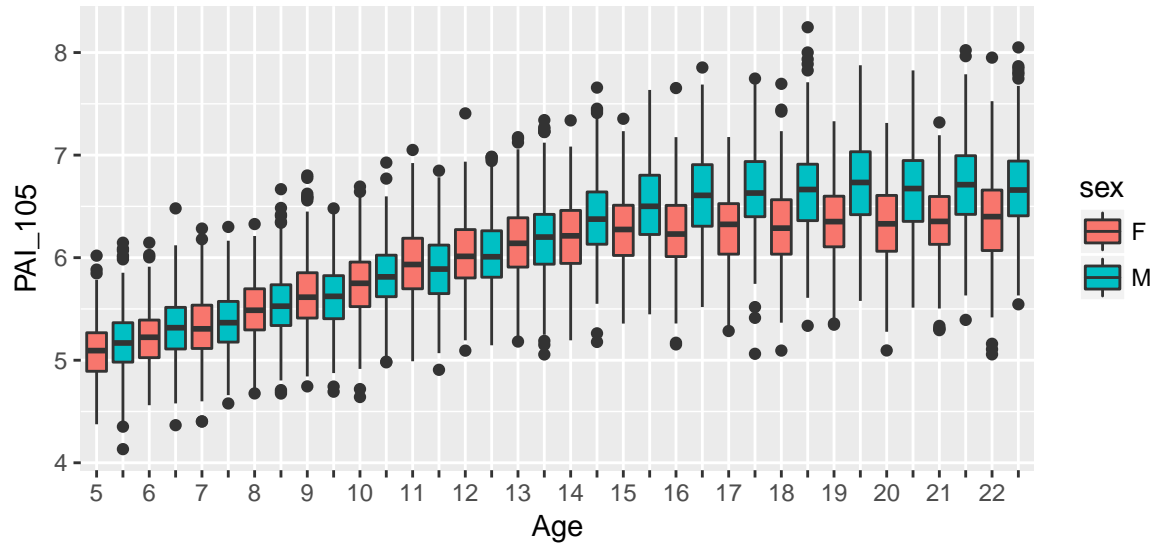

# Distributions of PAI\_106 by Sex and Age

ages from 5 years to 22 years old

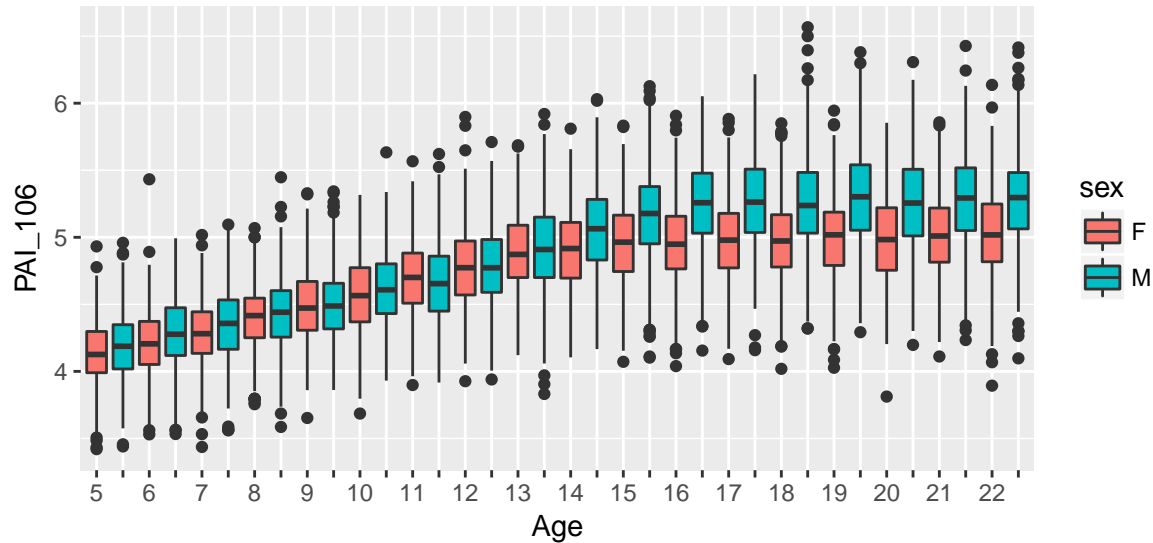

# Distributions of PAI\_107 by Sex and Age

ages from 5 years to 22 years old

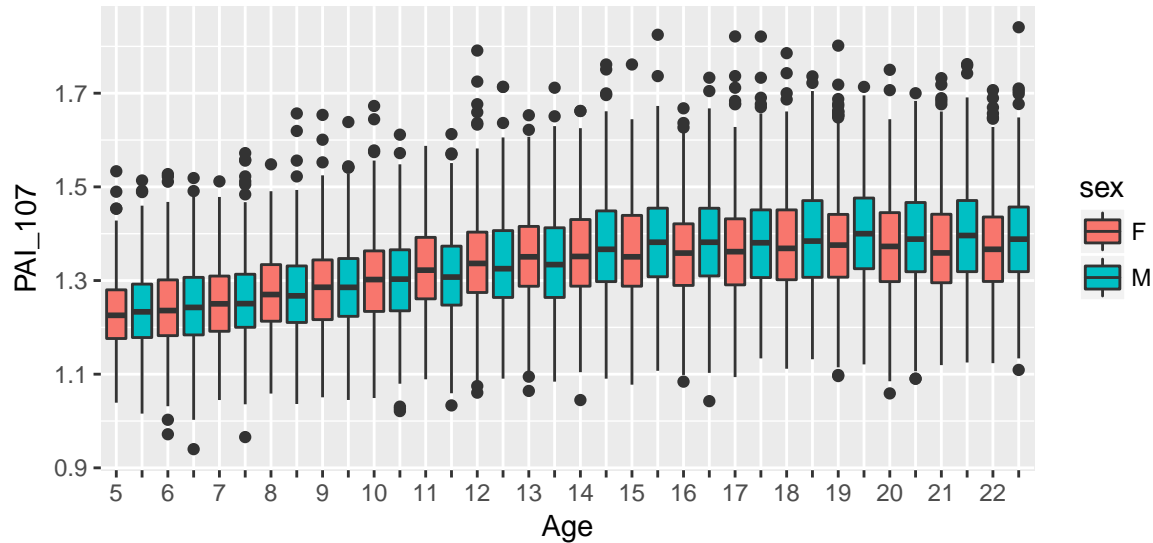

# Distributions of PAI\_108 by Sex and Age

ages from 5 years to 22 years old

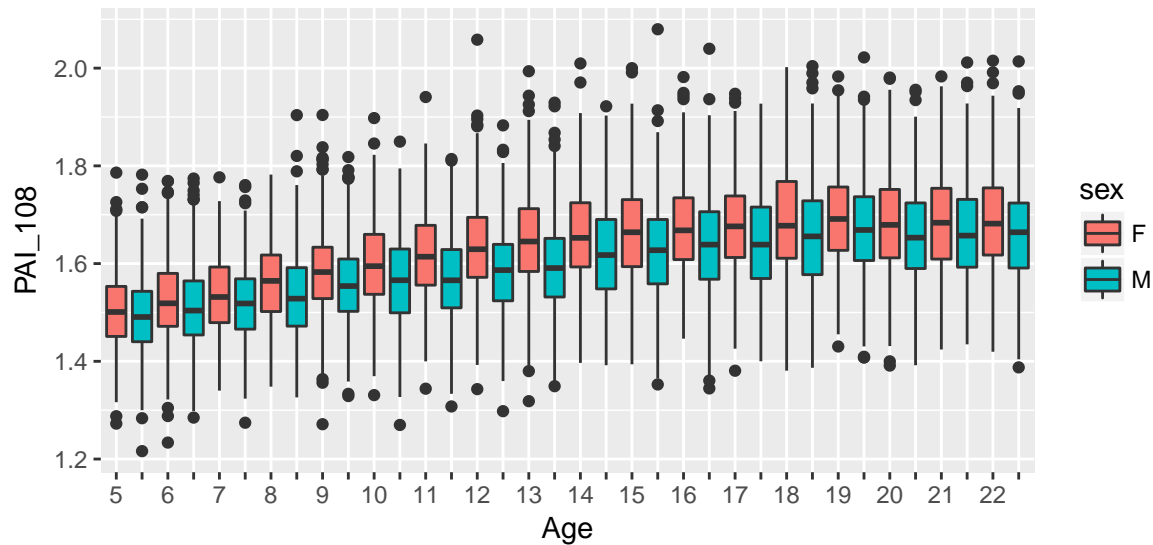

# Distributions of PAI\_109 by Sex and Age

ages from 5 years to 22 years old

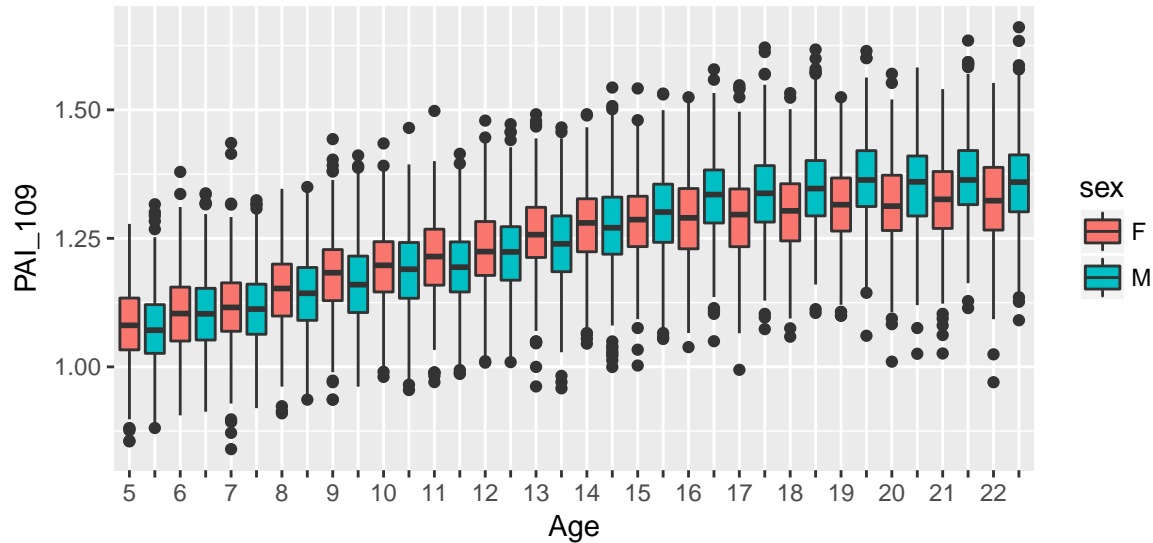

# Distributions of PAI\_10 by Sex and Age

ages from 5 years to 22 years old

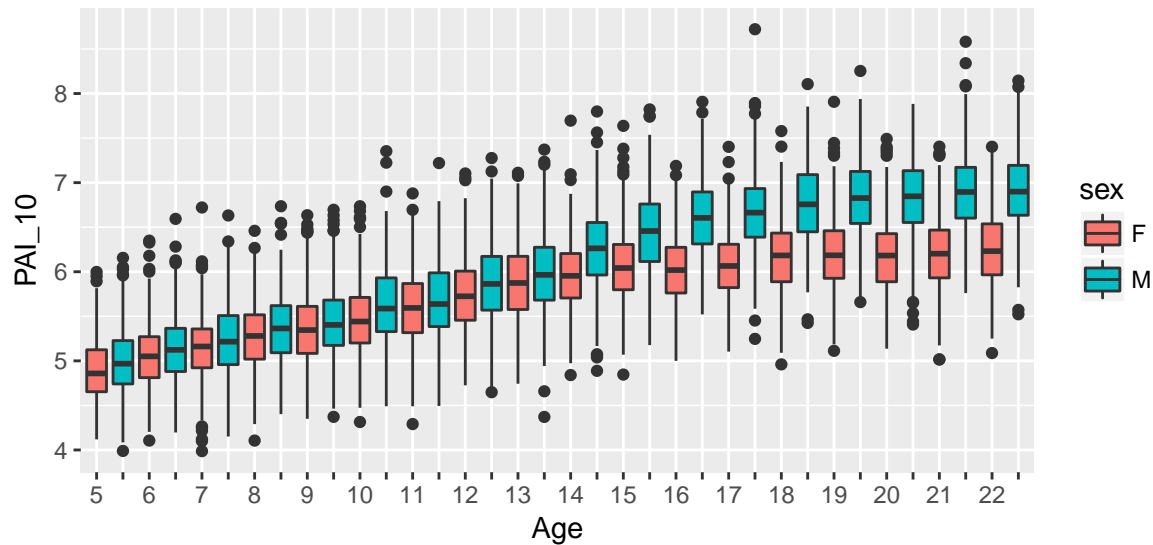

# Distributions of PAI\_110 by Sex and Age

ages from 5 years to 22 years old

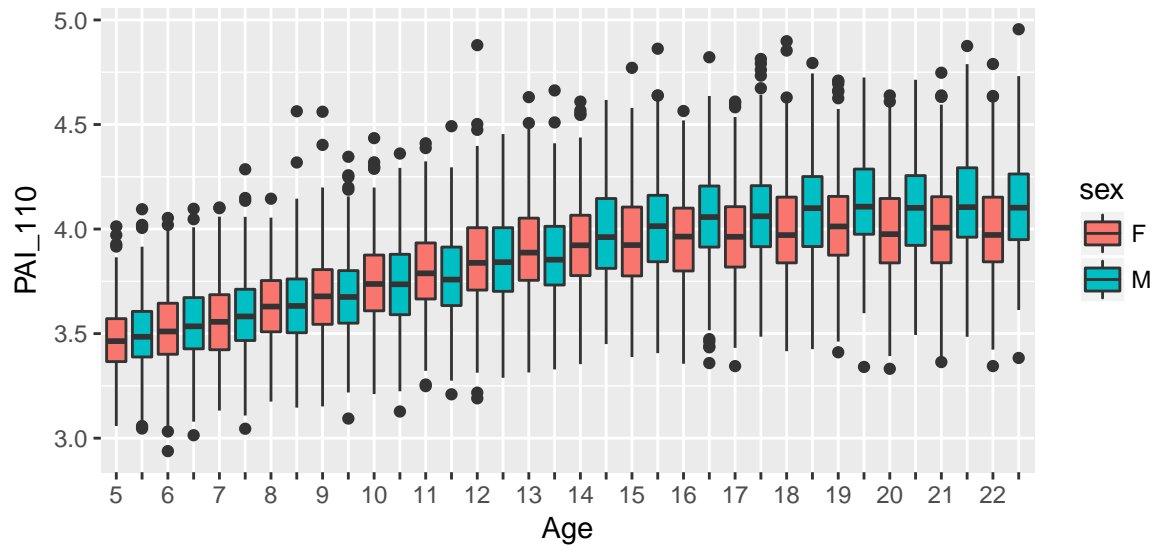

# Distributions of PAI\_111 by Sex and Age

ages from 5 years to 22 years old

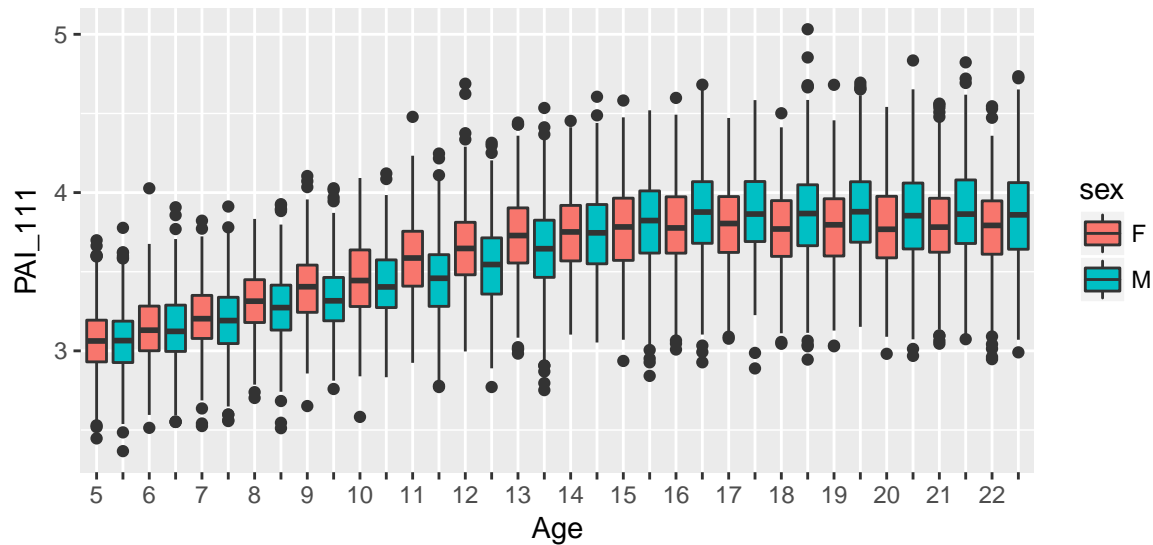

# Distributions of PAI\_112 by Sex and Age

ages from 5 years to 22 years old

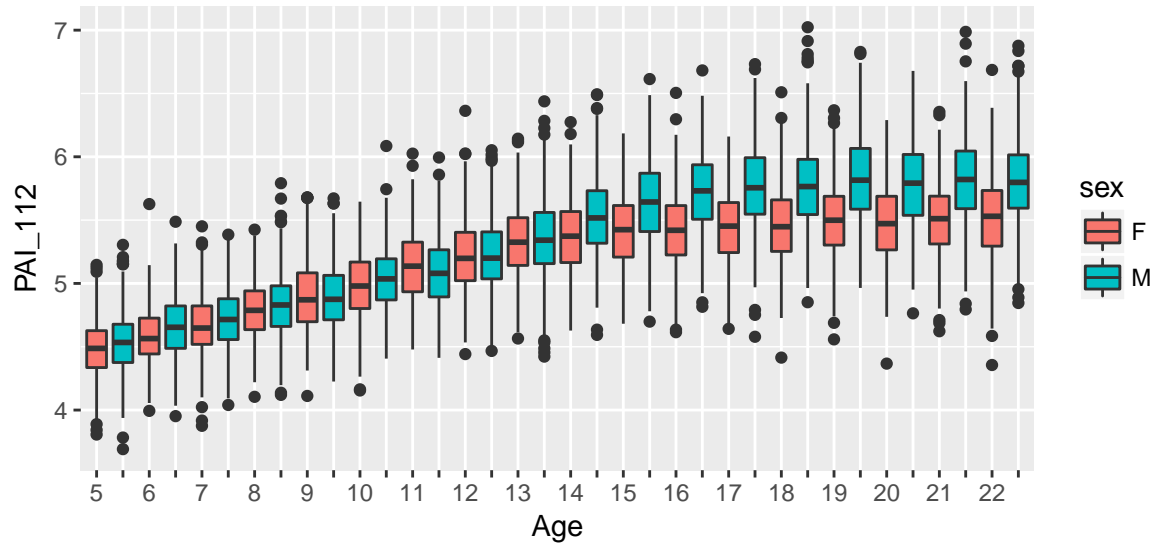

# Distributions of PAI\_113 by Sex and Age

ages from 5 years to 22 years old

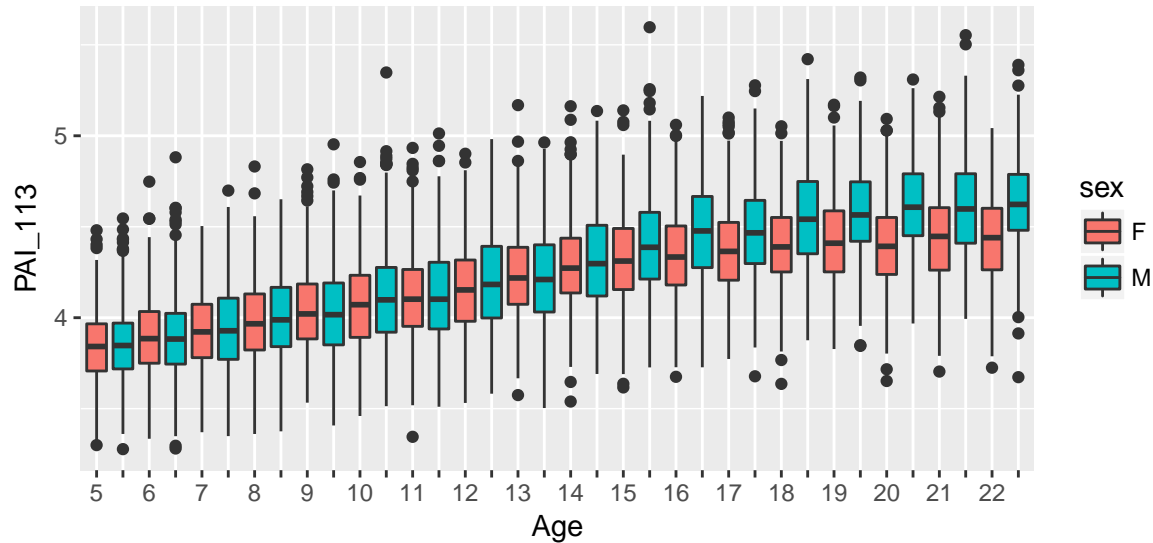

# Distributions of PAI\_114 by Sex and Age

ages from 5 years to 22 years old

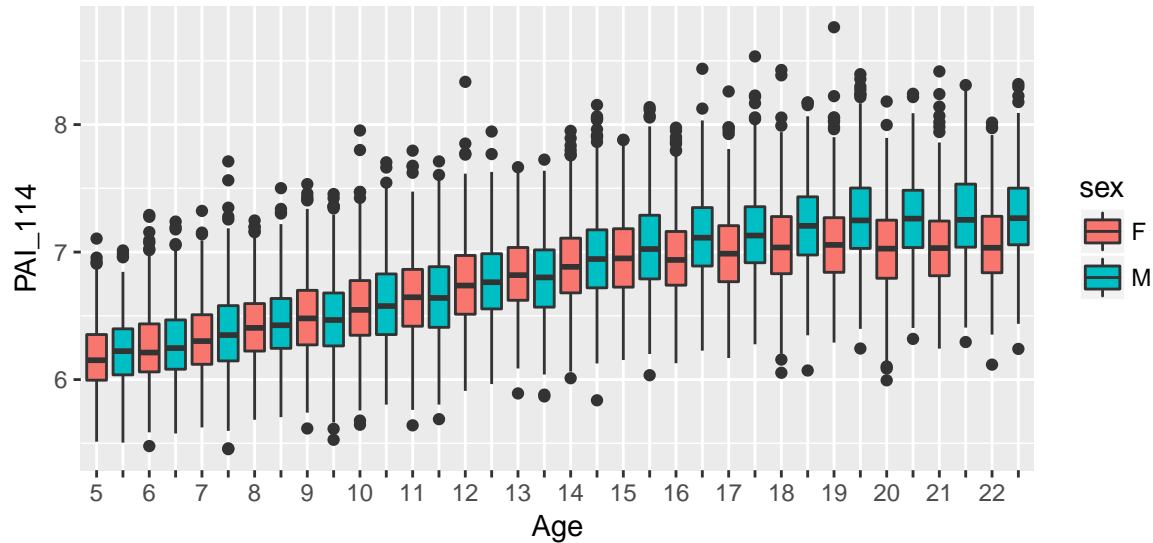

# Distributions of PAI\_115 by Sex and Age

ages from 5 years to 22 years old

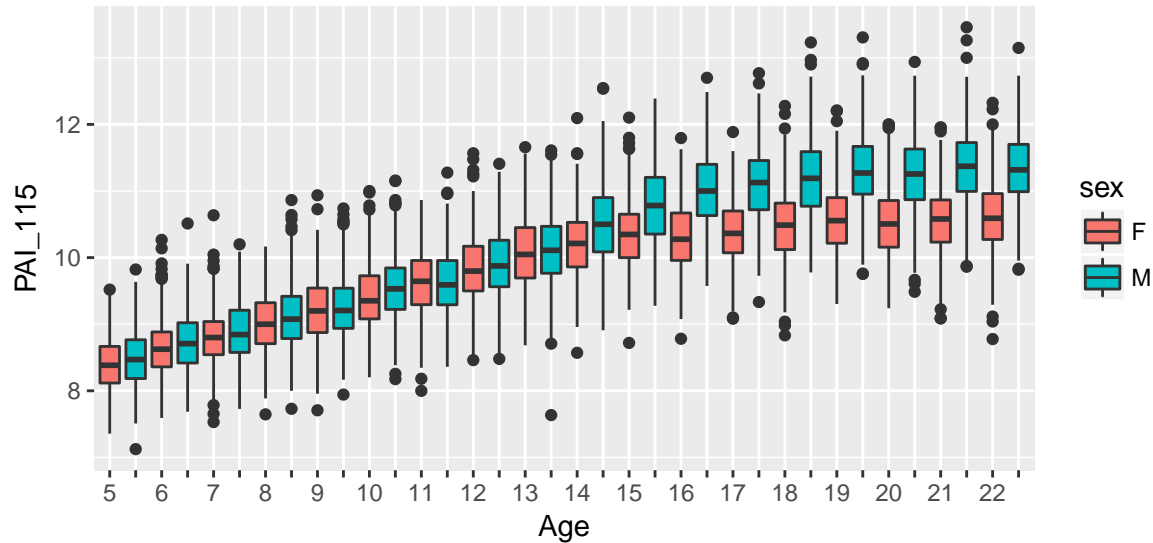

# Distributions of PAI\_116 by Sex and Age

ages from 5 years to 22 years old

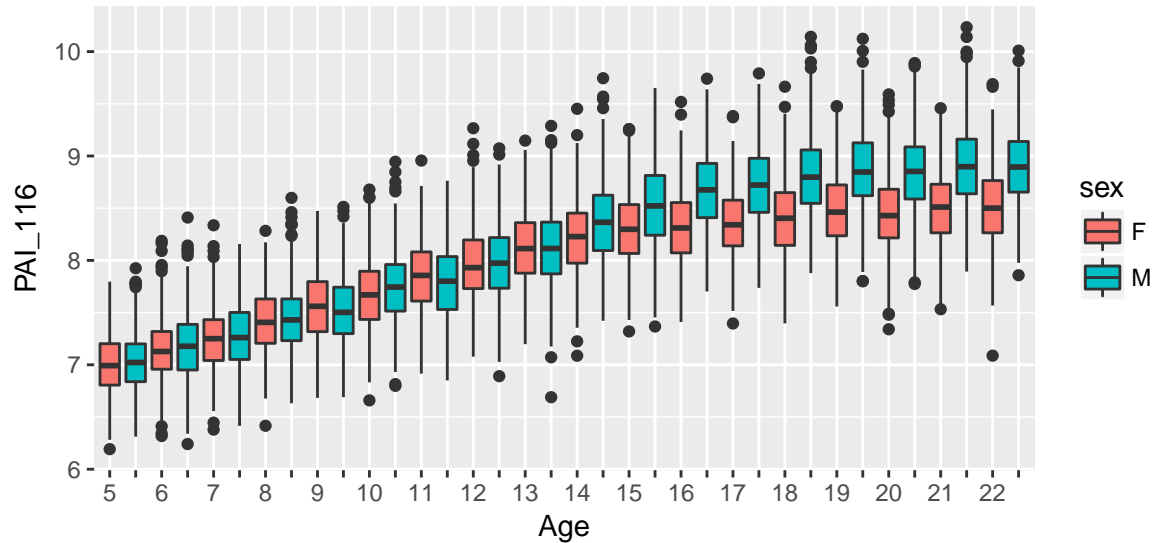

# Distributions of PAI\_117 by Sex and Age

ages from 5 years to 22 years old

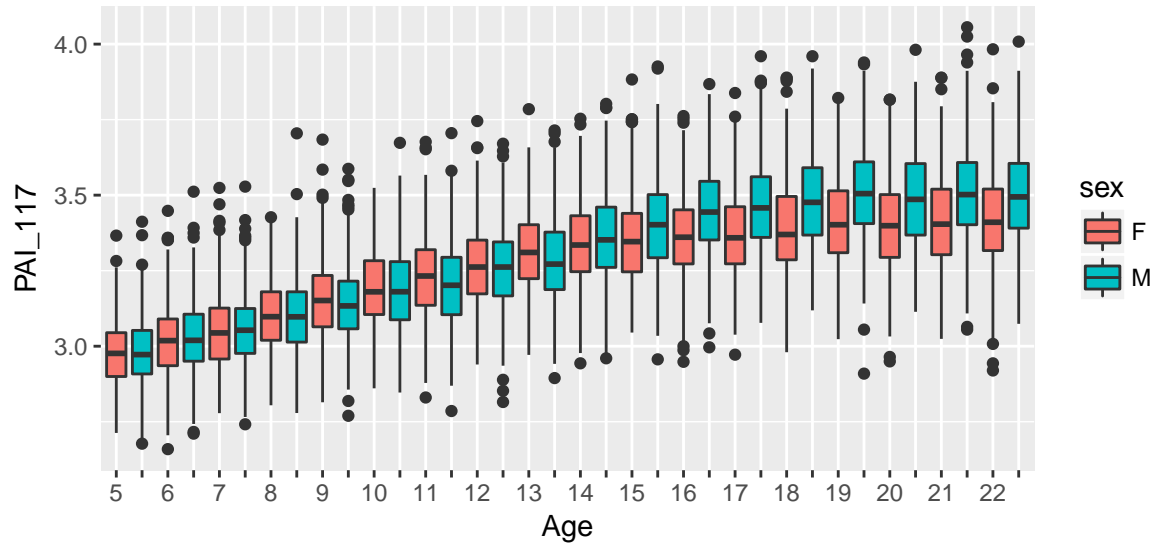

# Distributions of PAI\_118 by Sex and Age

ages from 5 years to 22 years old

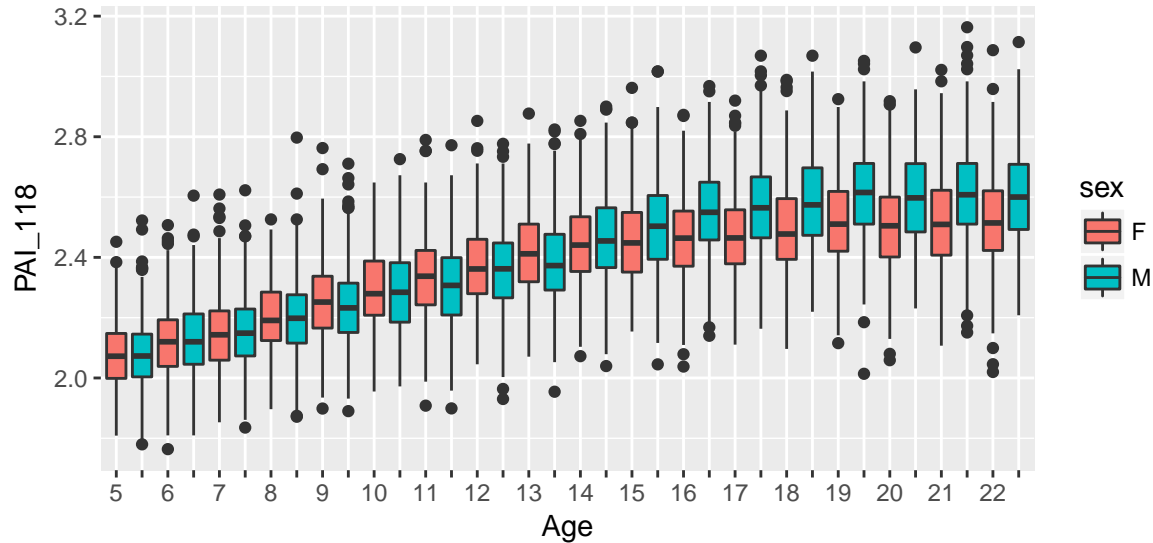

# Distributions of PAI\_119 by Sex and Age

ages from 5 years to 22 years old

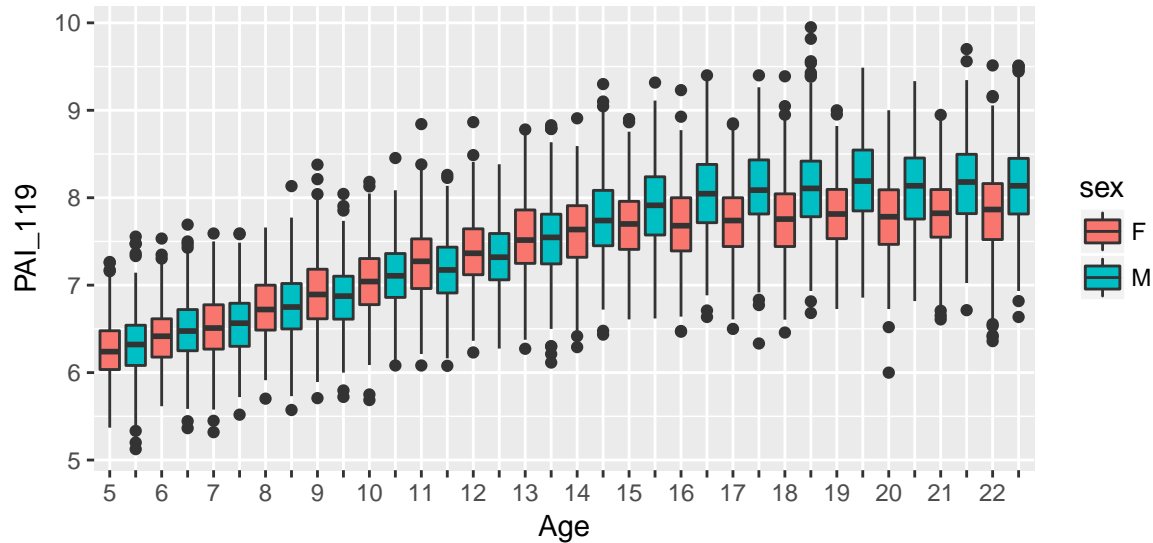

# Distributions of PAI\_11 by Sex and Age

ages from 5 years to 22 years old

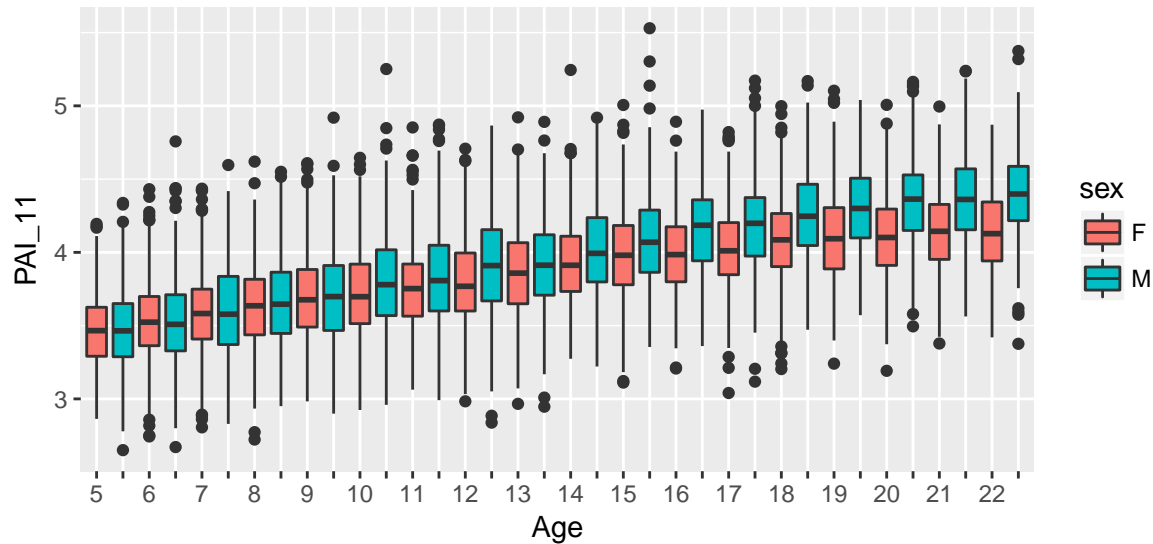

# Distributions of PAI\_120 by Sex and Age

ages from 5 years to 22 years old

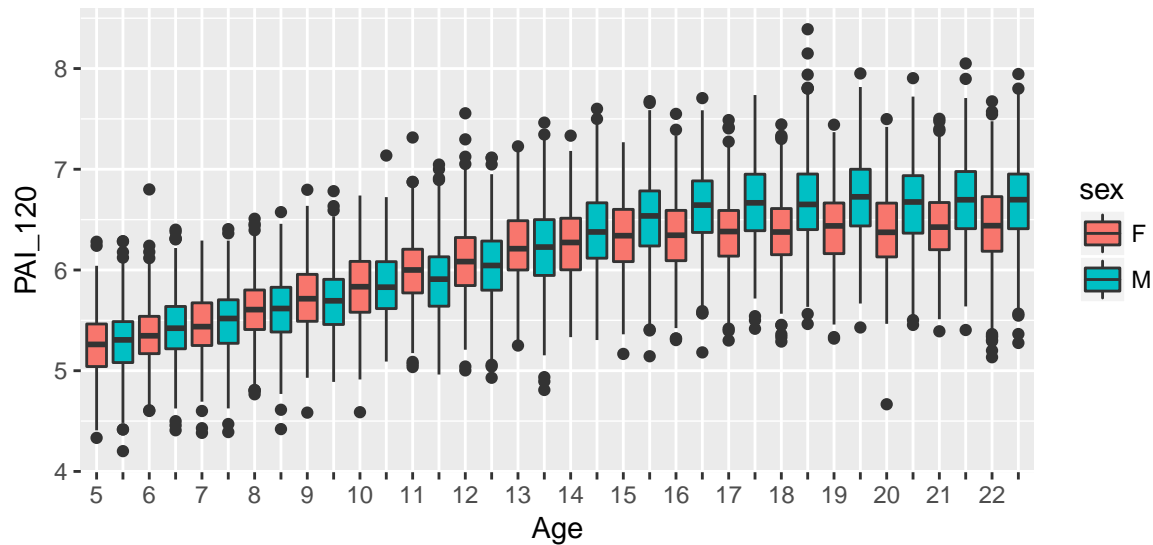

# Distributions of PAI\_121 by Sex and Age

ages from 5 years to 22 years old

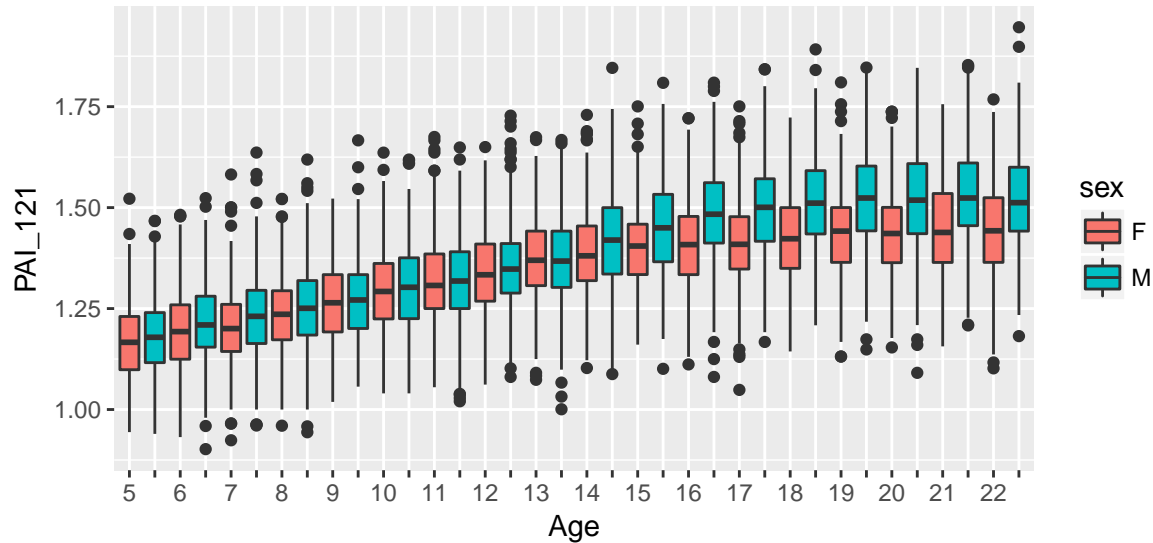

# Distributions of PAI\_122 by Sex and Age

ages from 5 years to 22 years old

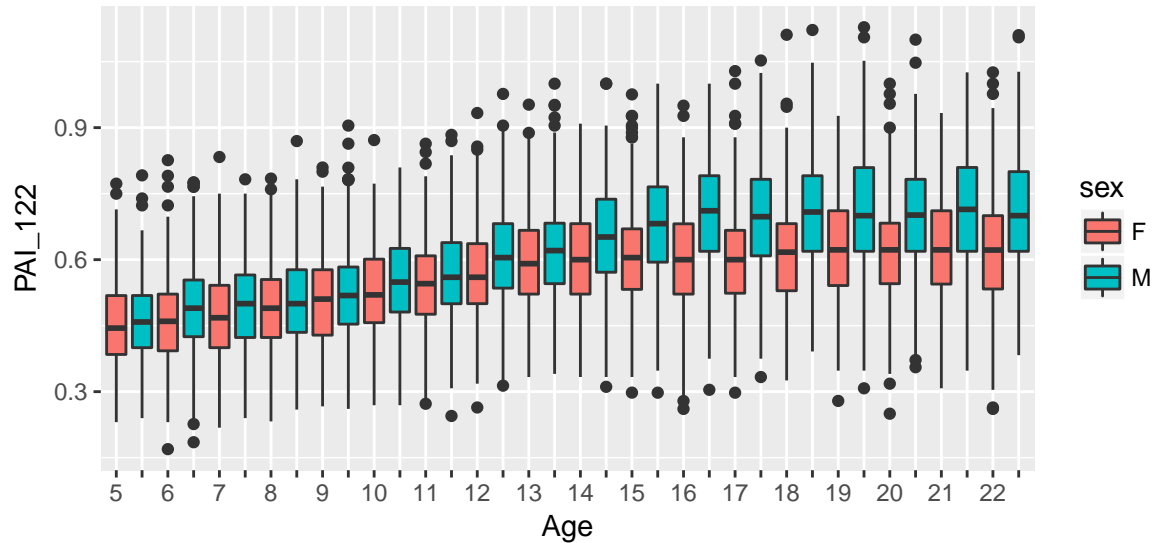

# Distributions of PAI\_123 by Sex and Age

ages from 5 years to 22 years old

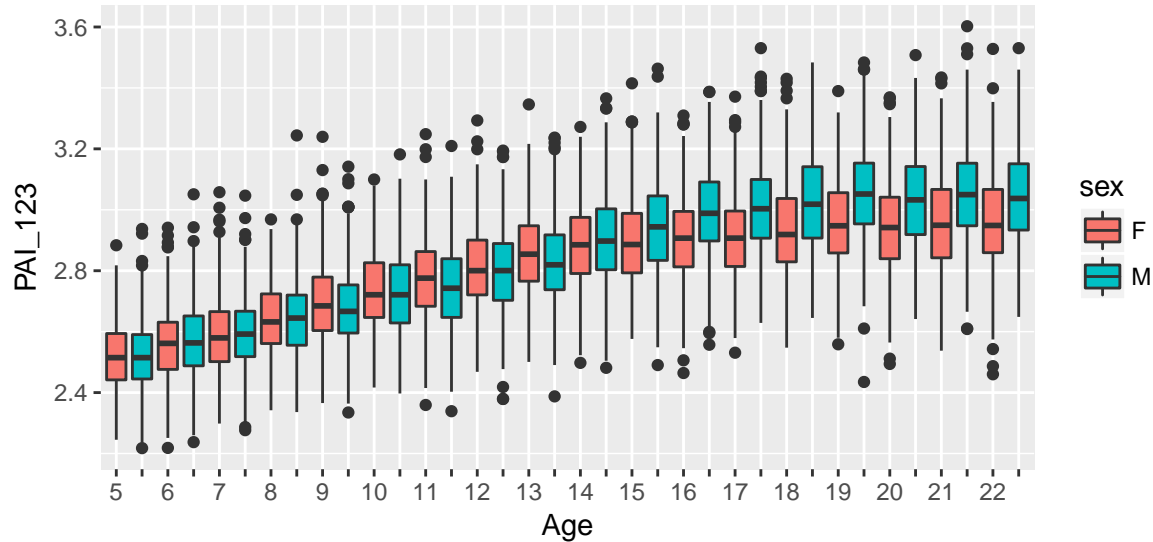

# Distributions of PAI\_124 by Sex and Age

ages from 5 years to 22 years old

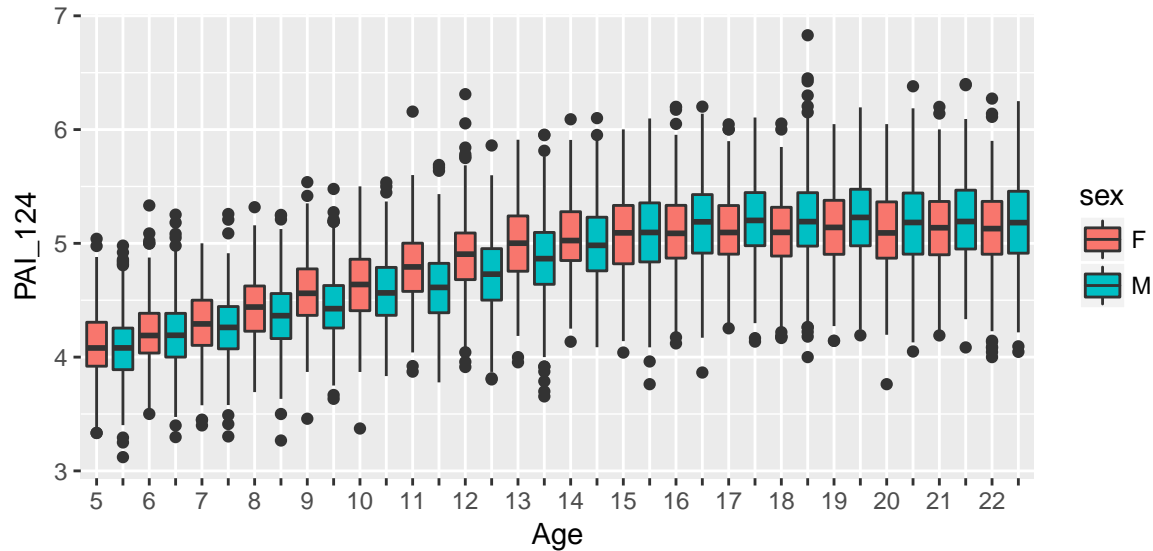

# Distributions of PAI\_125 by Sex and Age

ages from 5 years to 22 years old

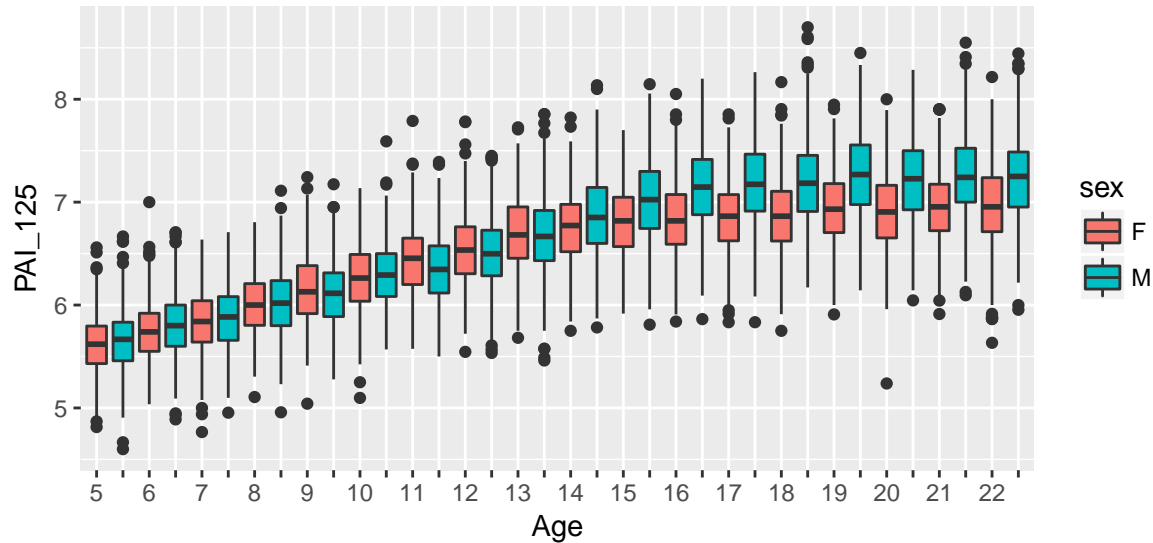

# Distributions of PAI\_126 by Sex and Age

ages from 5 years to 22 years old

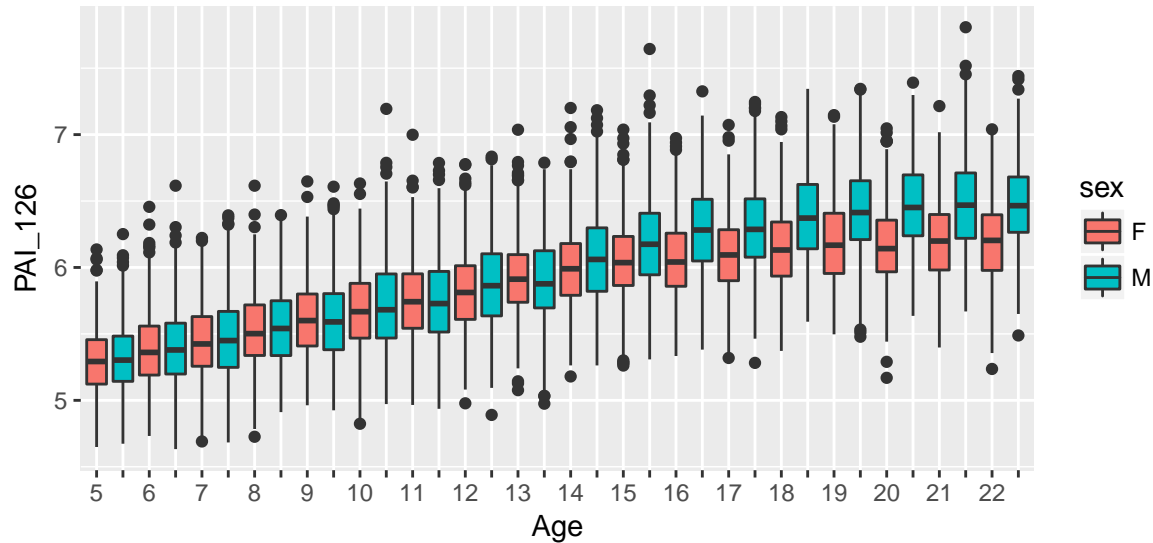

# Distributions of PAI\_127 by Sex and Age

ages from 5 years to 22 years old

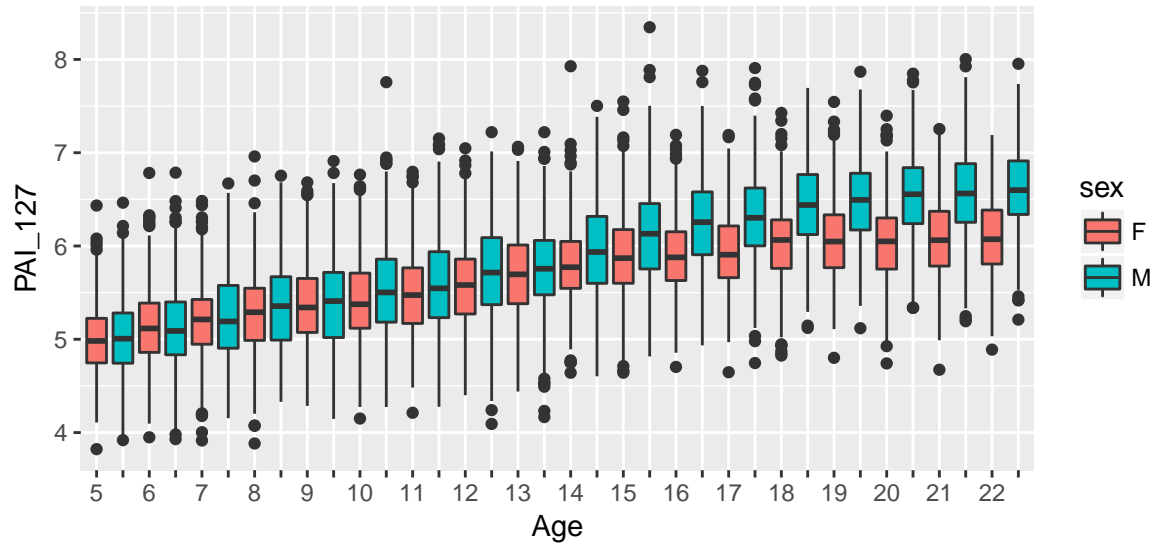

# Distributions of PAI\_128 by Sex and Age

ages from 5 years to 22 years old

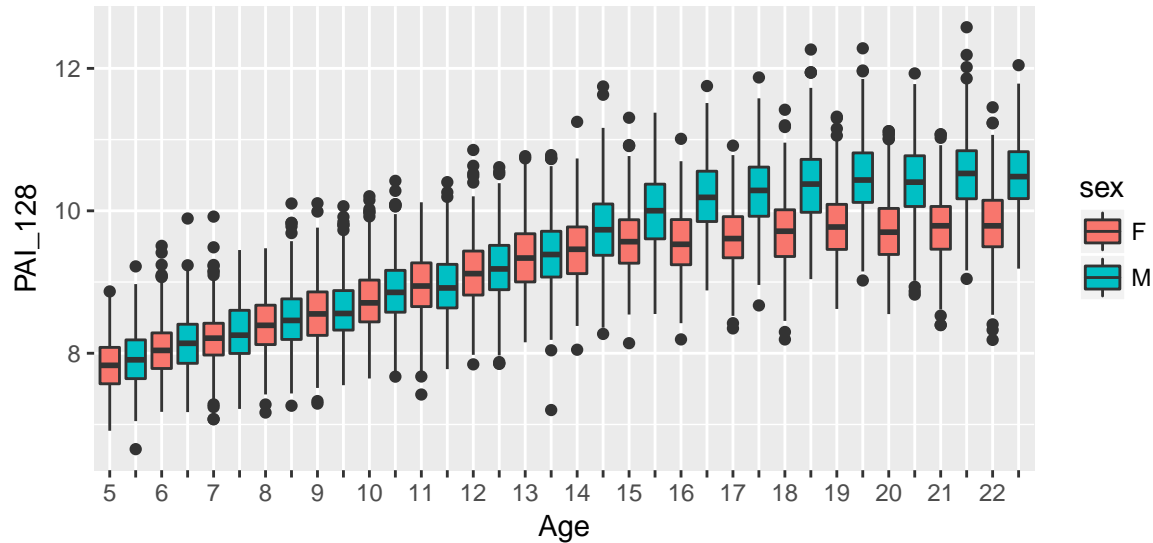

# Distributions of PAI\_129 by Sex and Age

ages from 5 years to 22 years old

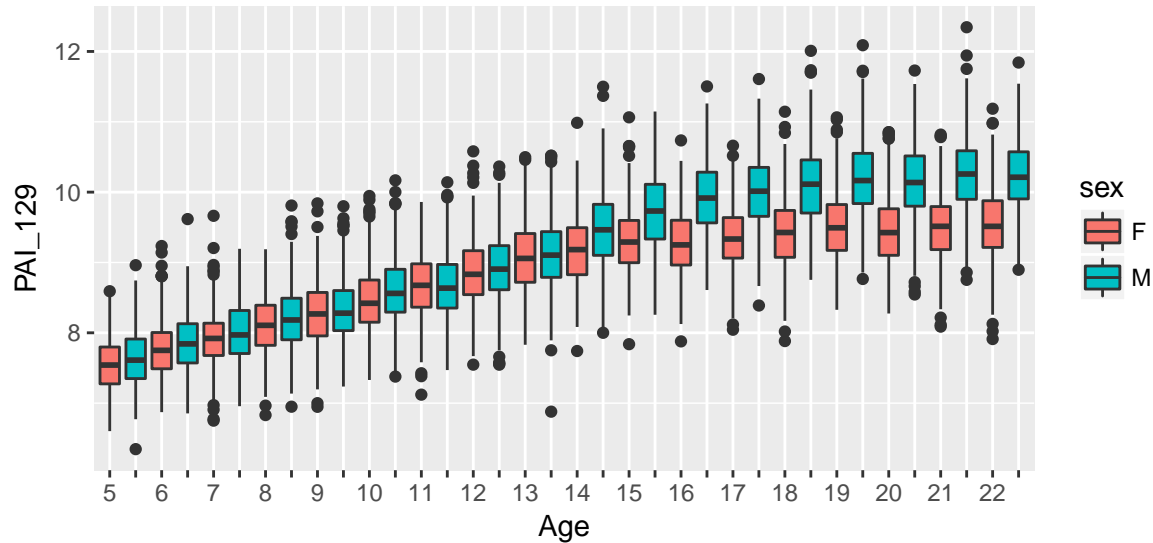

# Distributions of PAI\_12 by Sex and Age

ages from 5 years to 22 years old

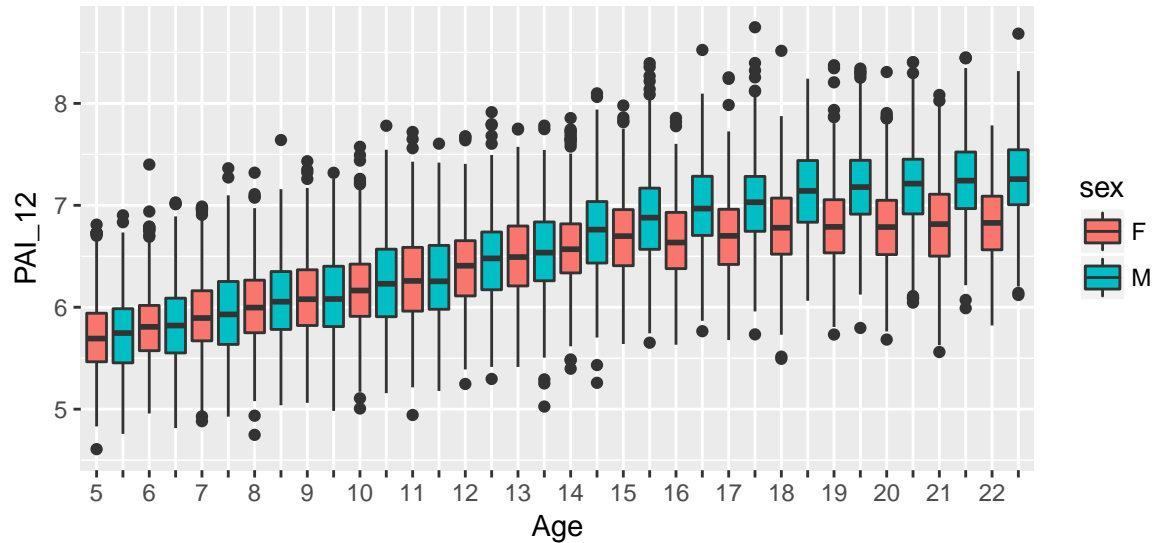

# Distributions of PAI\_130 by Sex and Age

ages from 5 years to 22 years old

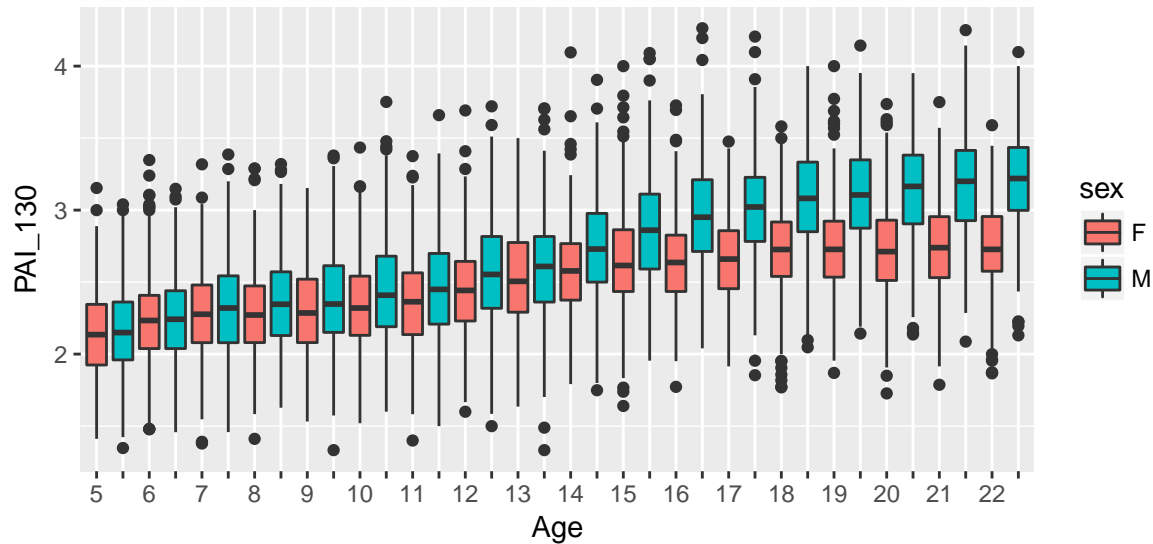

# Distributions of PAI\_131 by Sex and Age

ages from 5 years to 22 years old

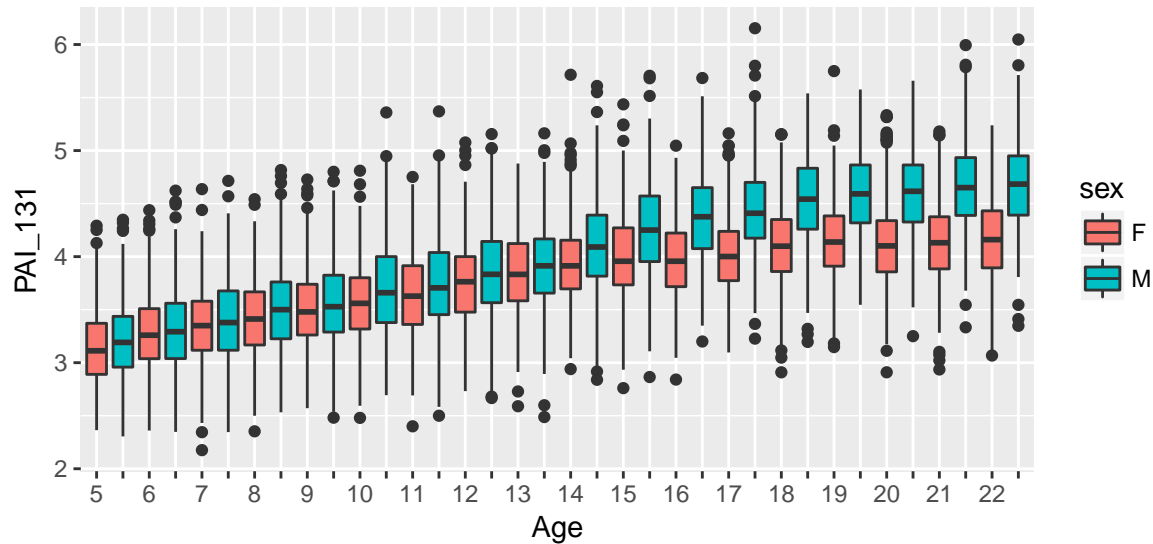

# Distributions of PAI\_132 by Sex and Age

ages from 5 years to 22 years old

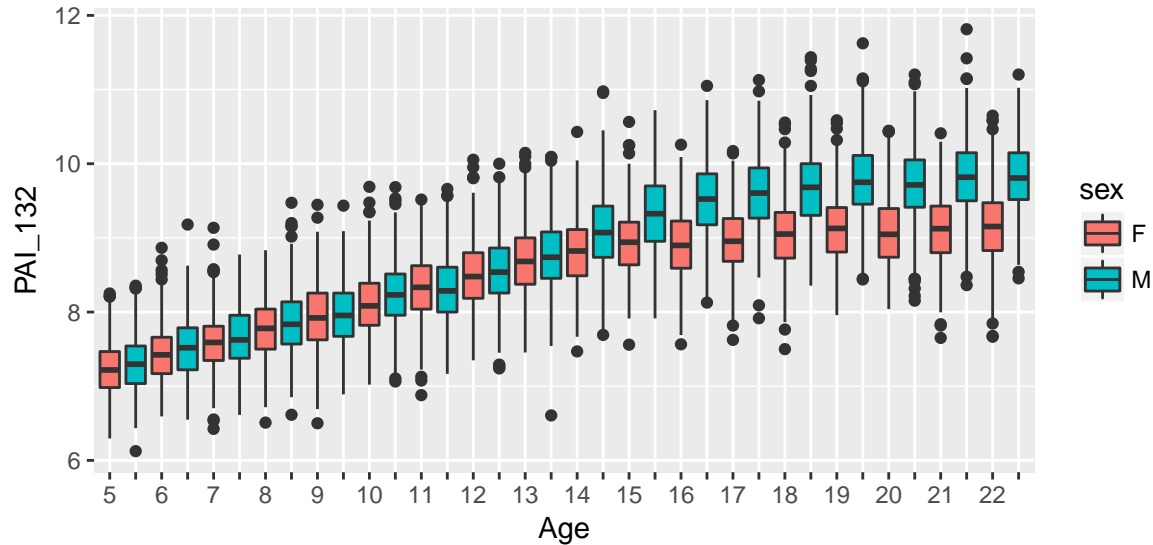

# Distributions of PAI\_133 by Sex and Age

ages from 5 years to 22 years old

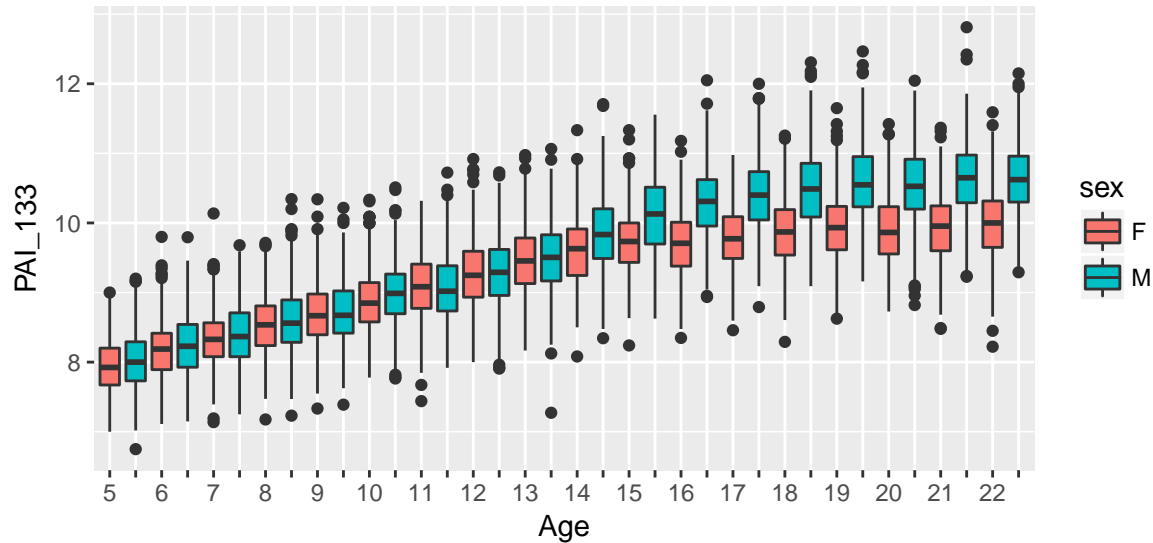

# Distributions of PAI\_134 by Sex and Age

ages from 5 years to 22 years old

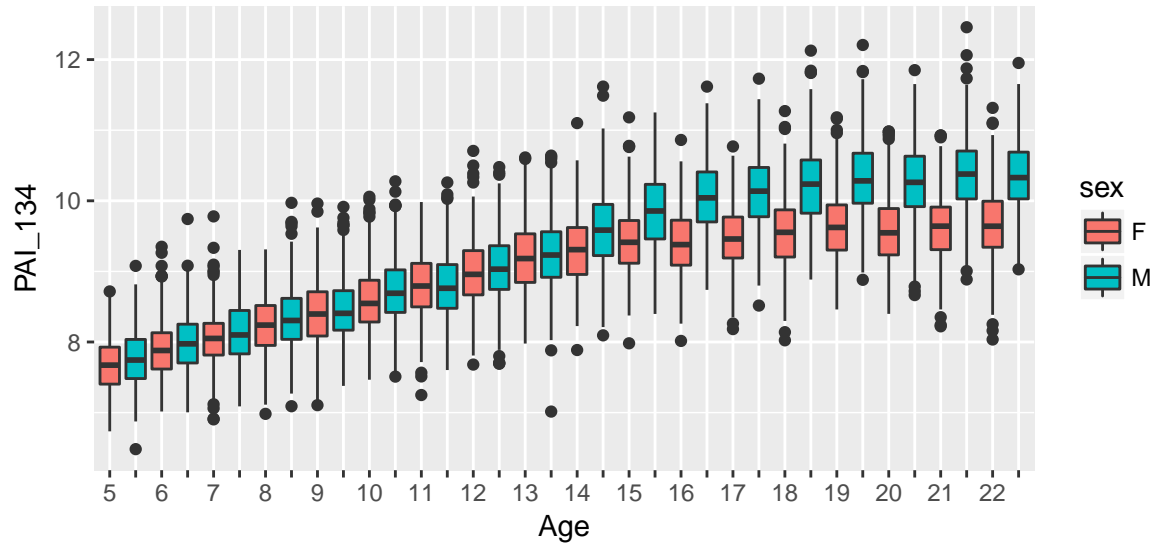

# Distributions of PAI\_135 by Sex and Age

ages from 5 years to 22 years old

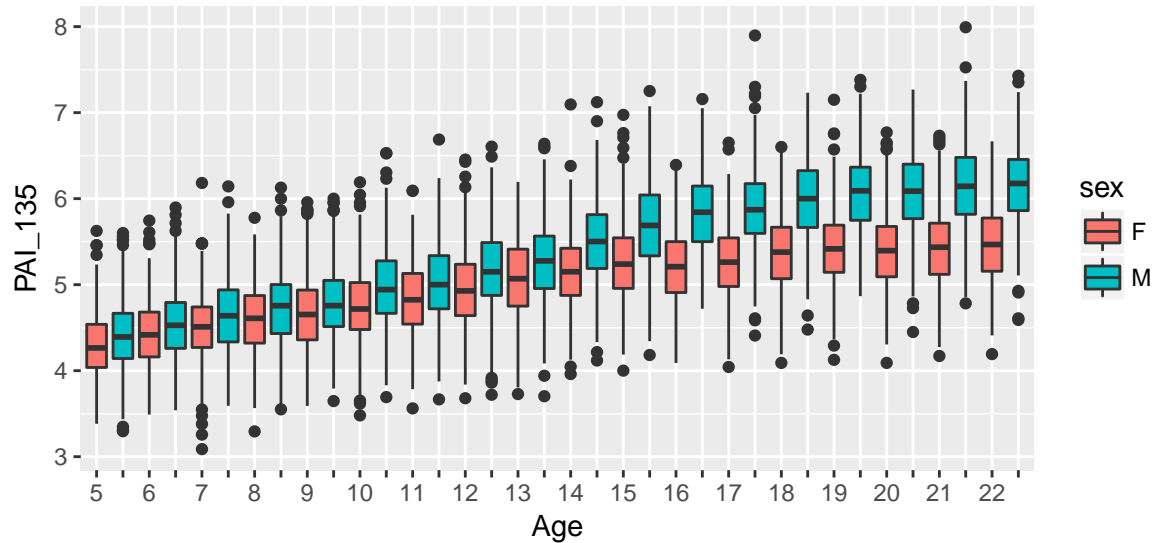

# Distributions of PAI\_136 by Sex and Age

ages from 5 years to 22 years old

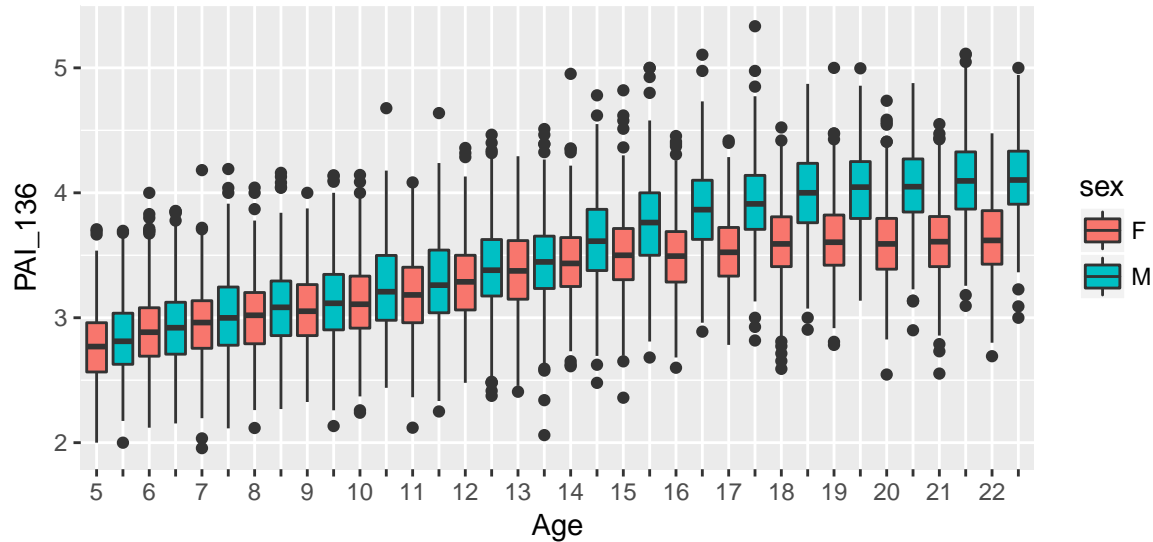

# Distributions of PAI\_137 by Sex and Age

ages from 5 years to 22 years old

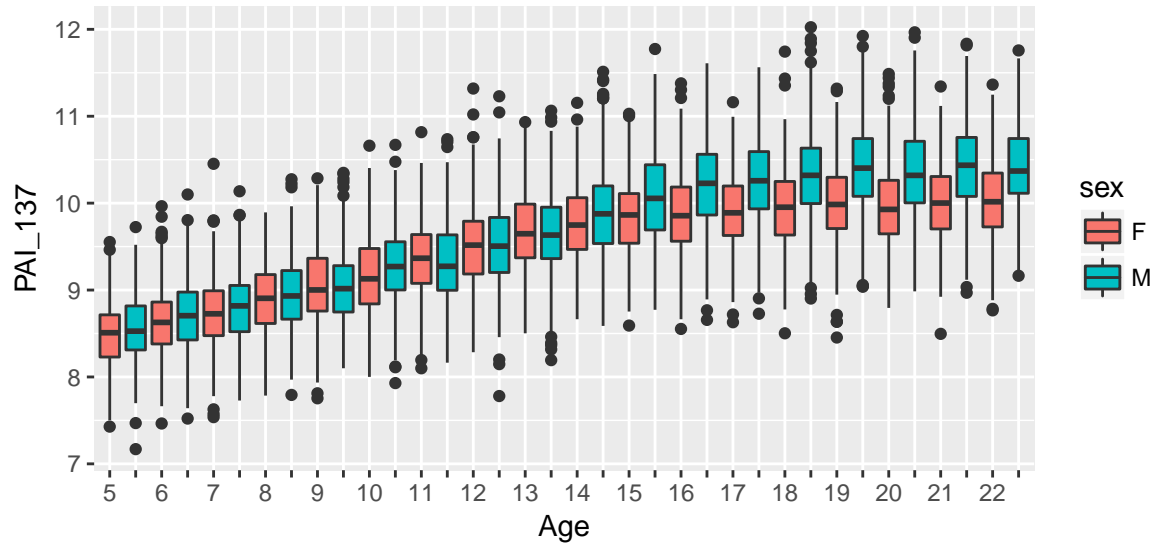

# Distributions of PAI\_138 by Sex and Age

ages from 5 years to 22 years old

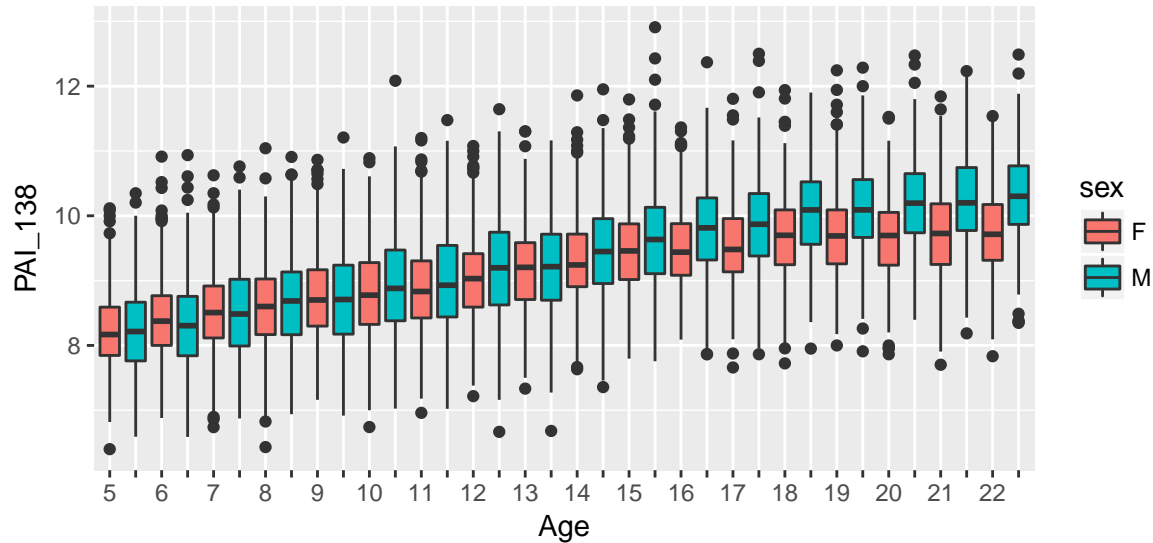

# Distributions of PAI\_139 by Sex and Age

ages from 5 years to 22 years old

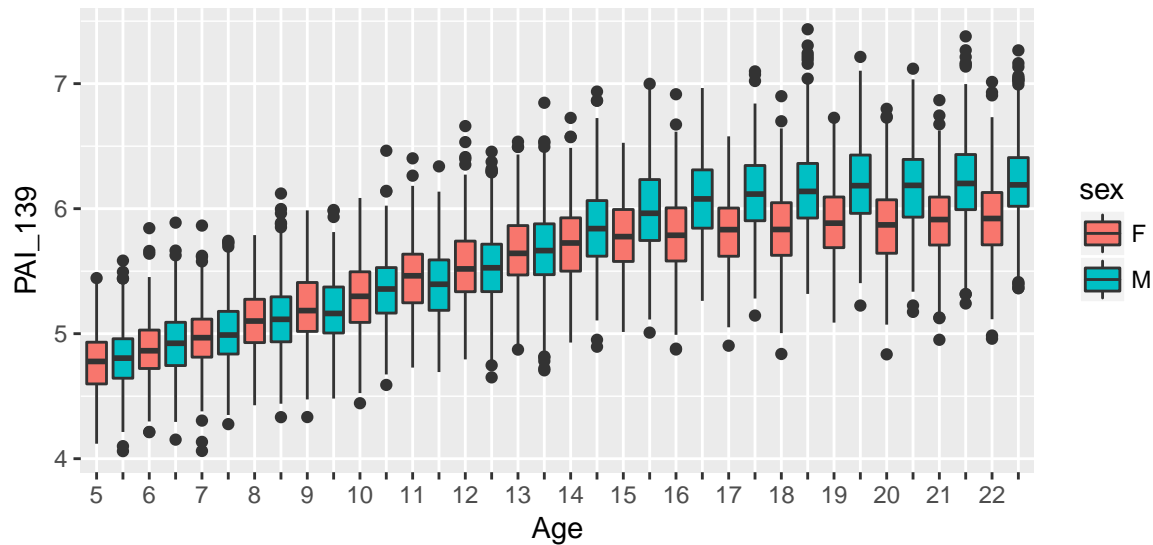

# Distributions of PAI\_13 by Sex and Age

ages from 5 years to 22 years old

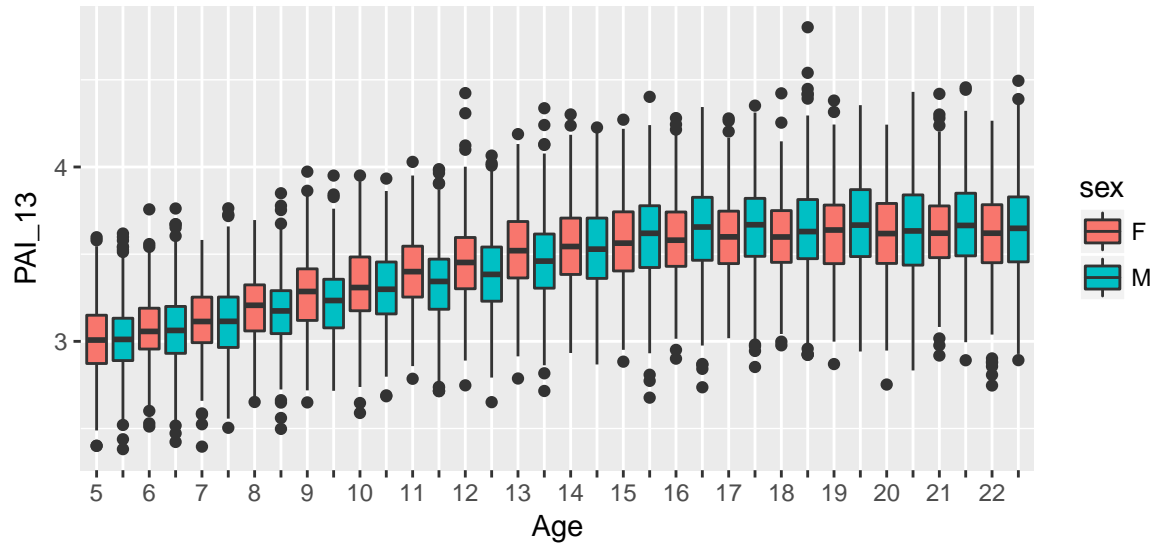

# Distributions of PAI\_140 by Sex and Age

ages from 5 years to 22 years old

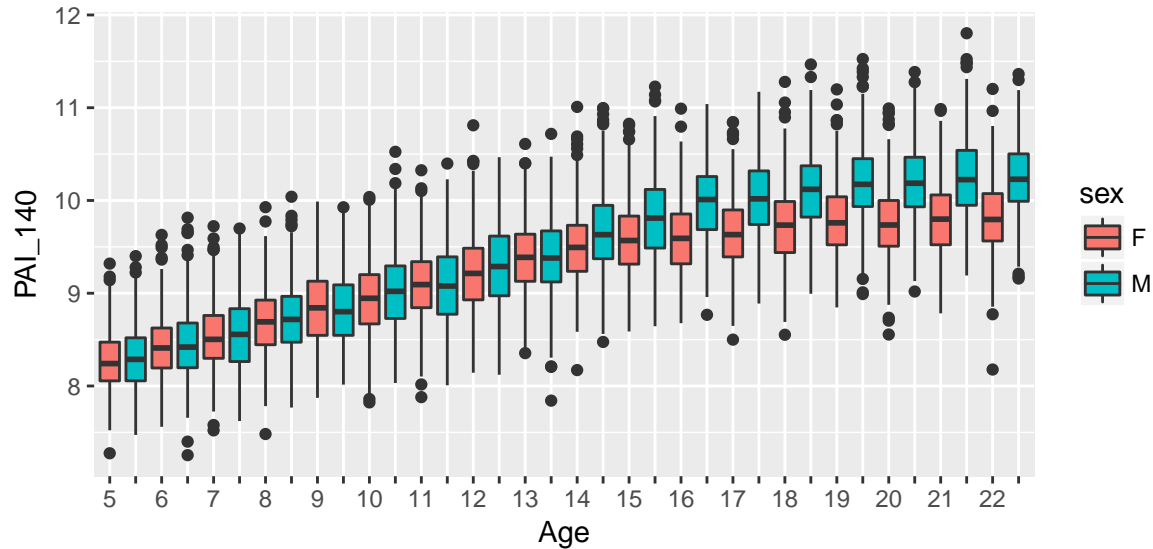

# Distributions of PAI\_141 by Sex and Age

ages from 5 years to 22 years old

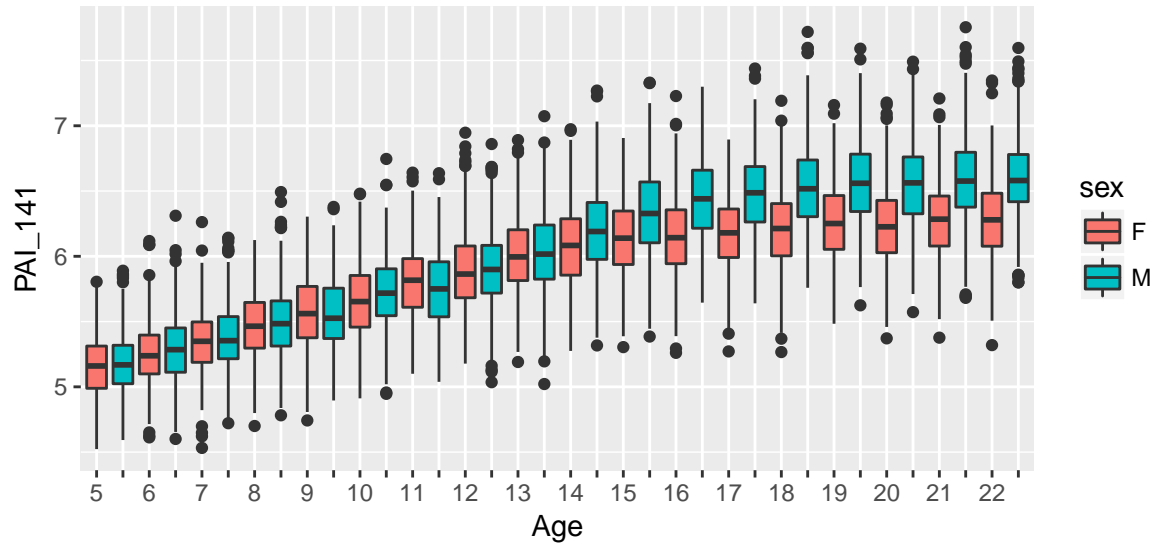

# Distributions of PAI\_142 by Sex and Age

ages from 5 years to 22 years old

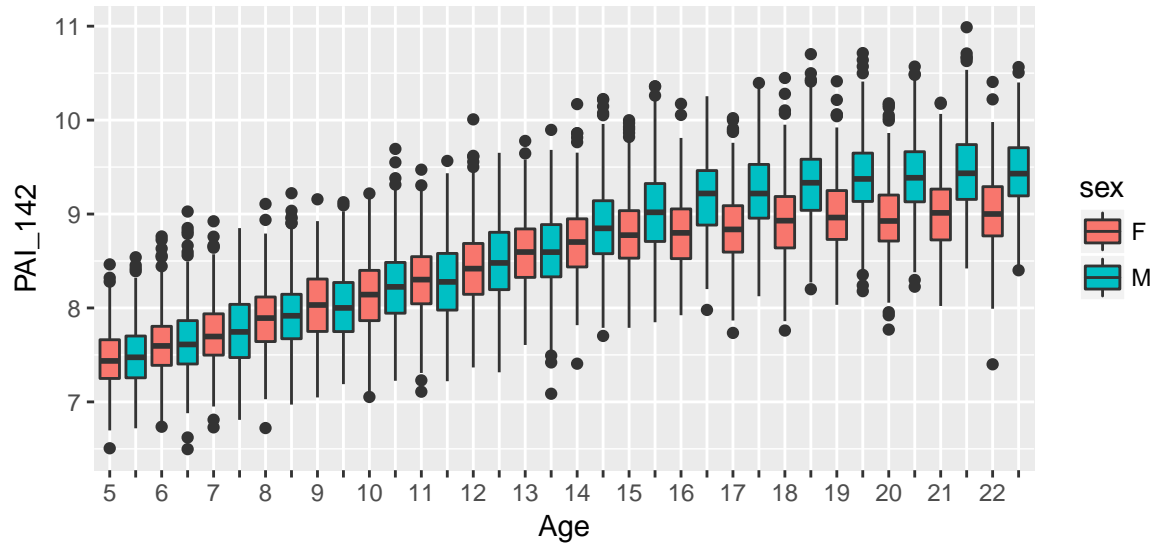

# Distributions of PAI\_143 by Sex and Age

ages from 5 years to 22 years old

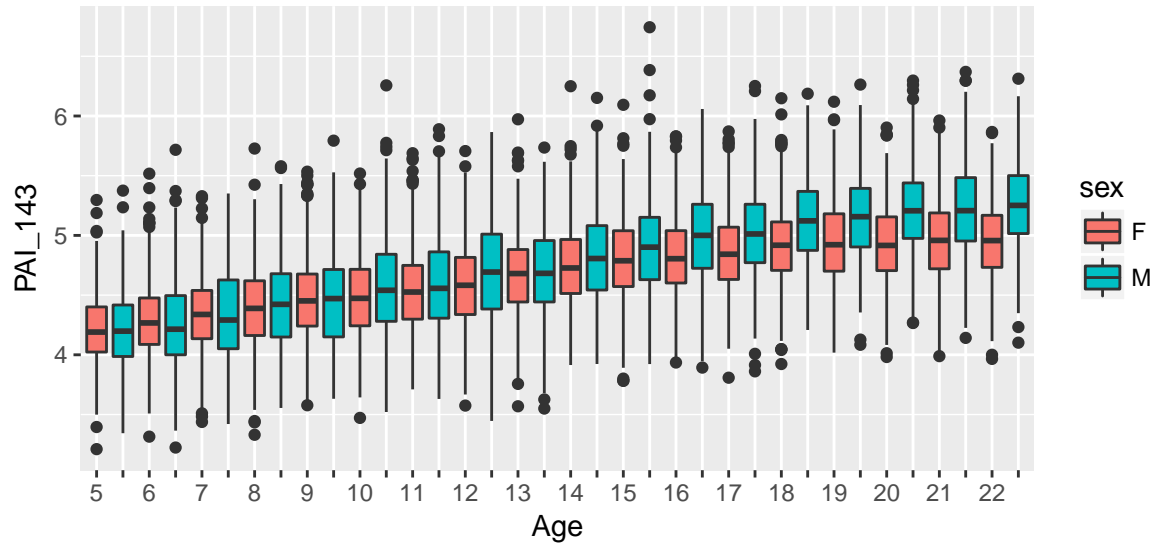

# Distributions of PAI\_144 by Sex and Age

ages from 5 years to 22 years old

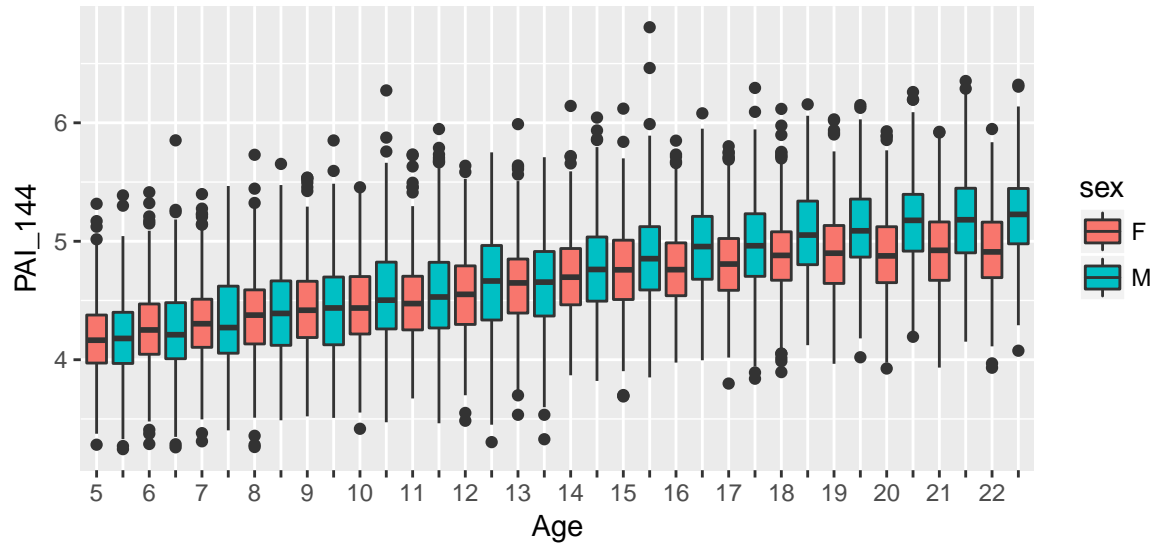

# Distributions of PAI\_145 by Sex and Age

ages from 5 years to 22 years old

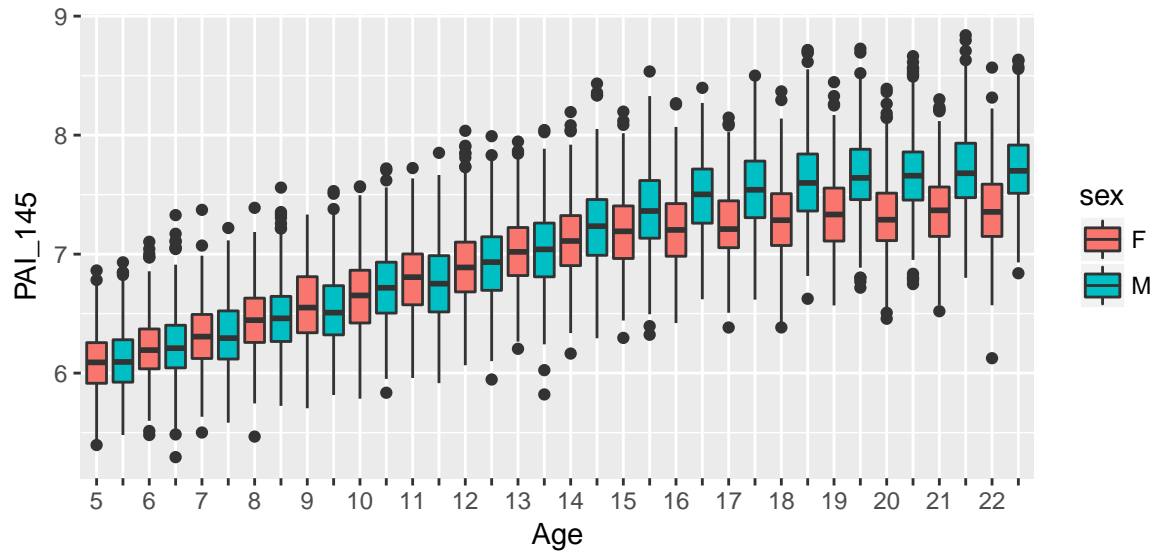

# Distributions of PAI\_146 by Sex and Age

ages from 5 years to 22 years old

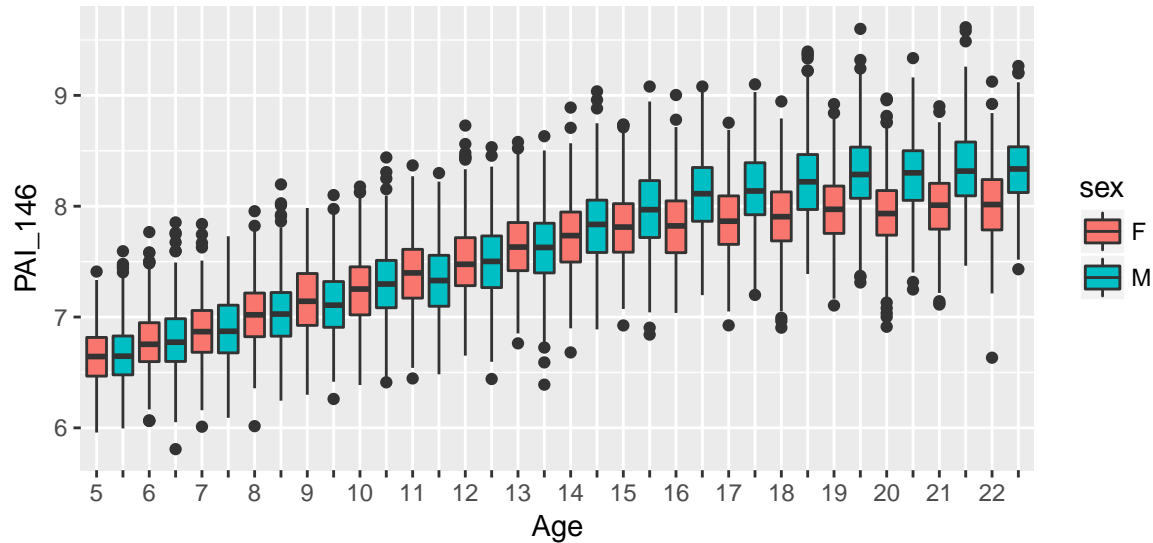

# Distributions of PAI\_147 by Sex and Age

ages from 5 years to 22 years old

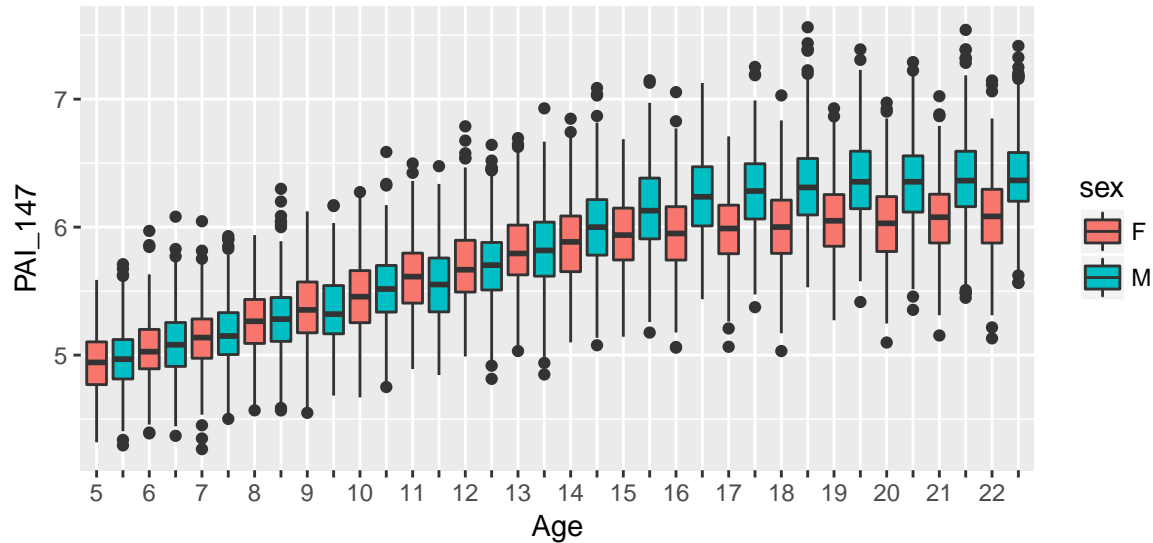

# Distributions of PAI\_148 by Sex and Age

ages from 5 years to 22 years old

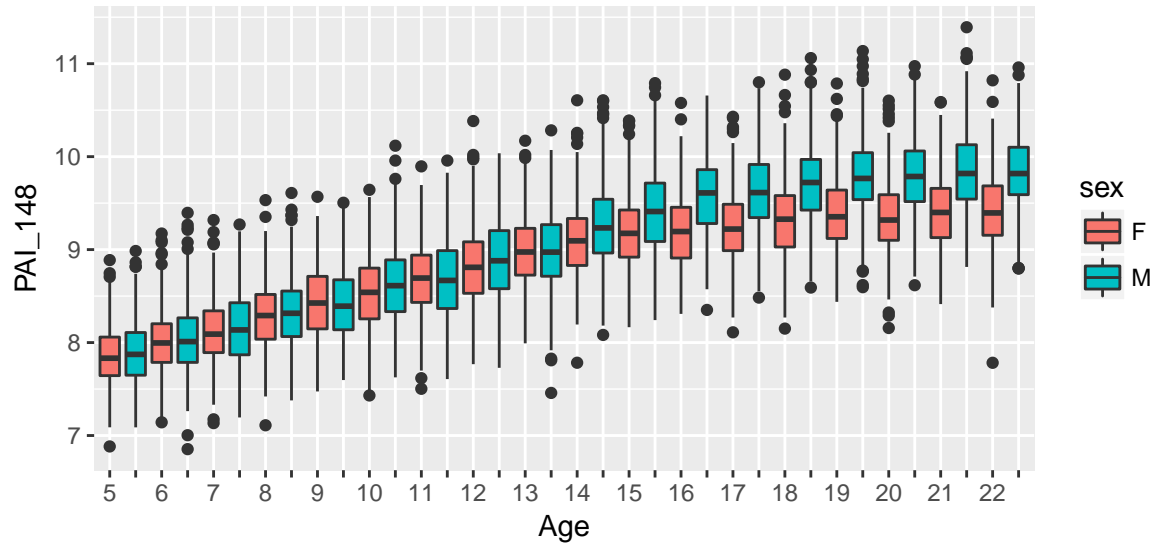

# Distributions of PAI\_149 by Sex and Age

ages from 5 years to 22 years old

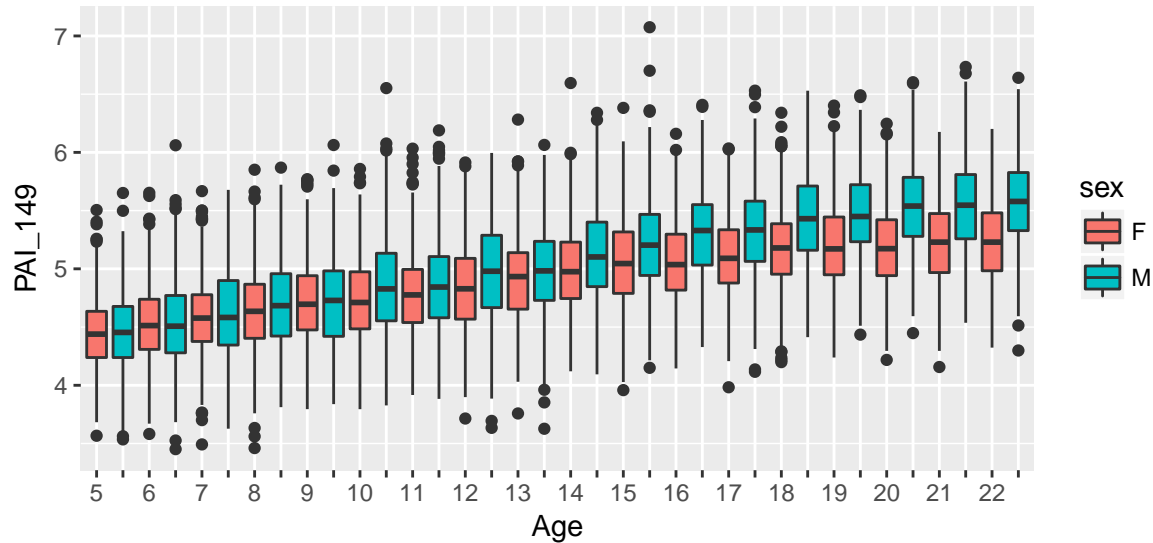

# Distributions of PAI\_14 by Sex and Age

ages from 5 years to 22 years old

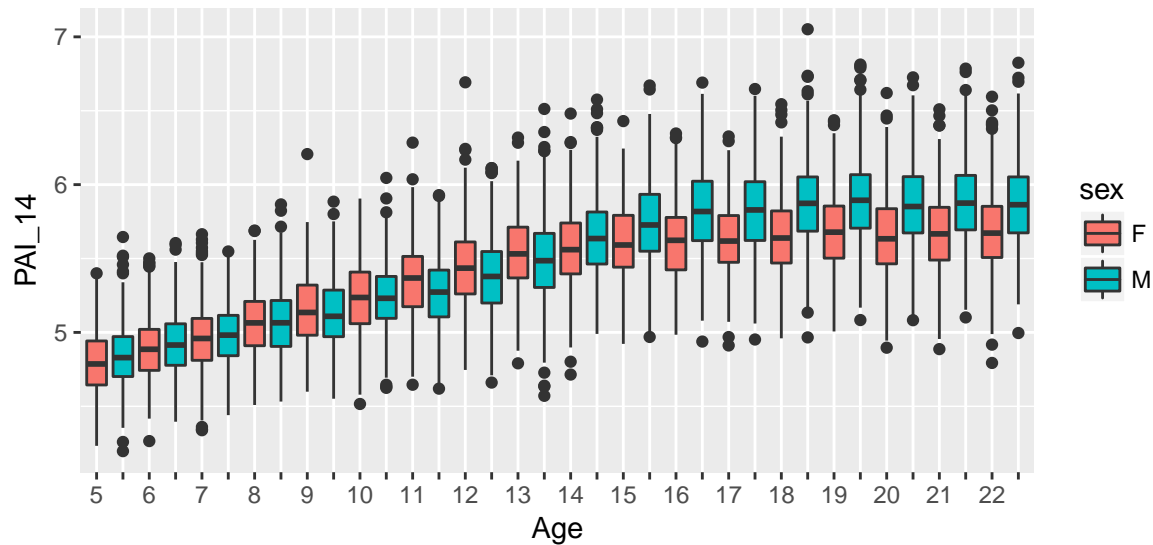

# Distributions of PAI\_150 by Sex and Age

ages from 5 years to 22 years old

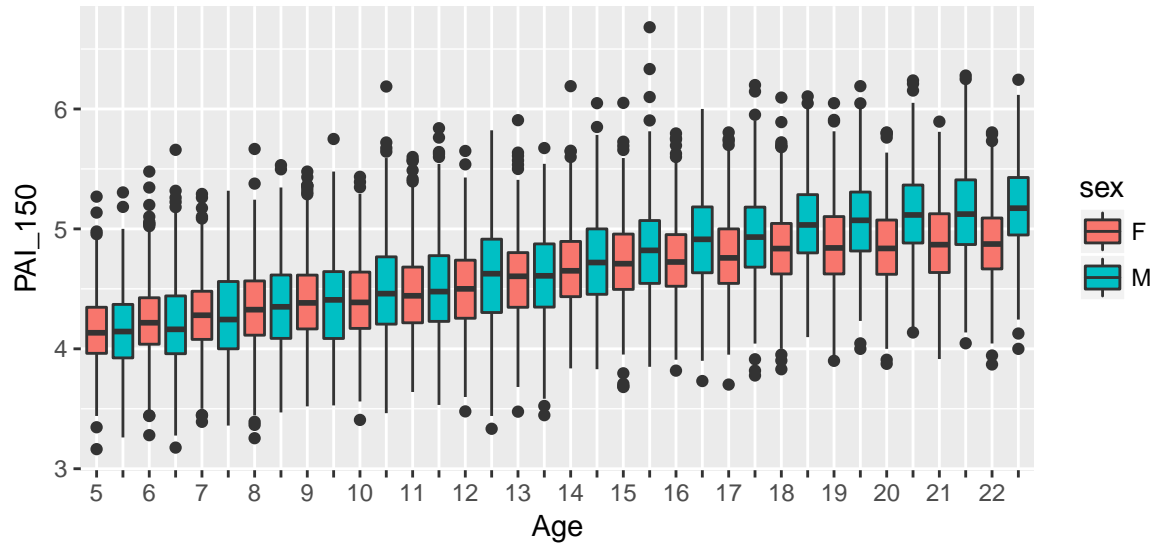

# Distributions of PAI\_151 by Sex and Age

ages from 5 years to 22 years old

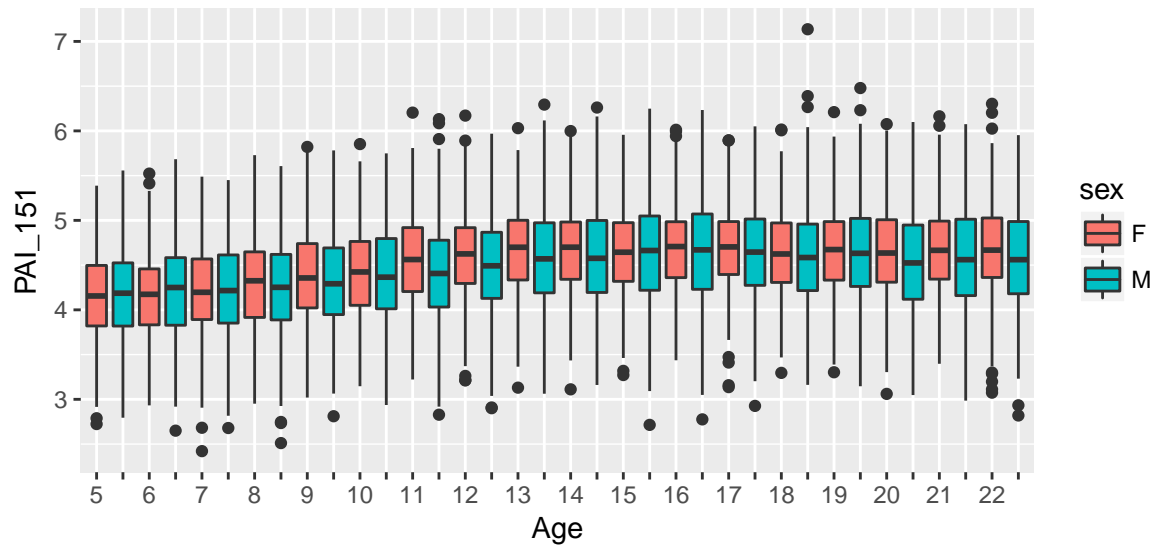

# Distributions of PAI\_152 by Sex and Age

ages from 5 years to 22 years old

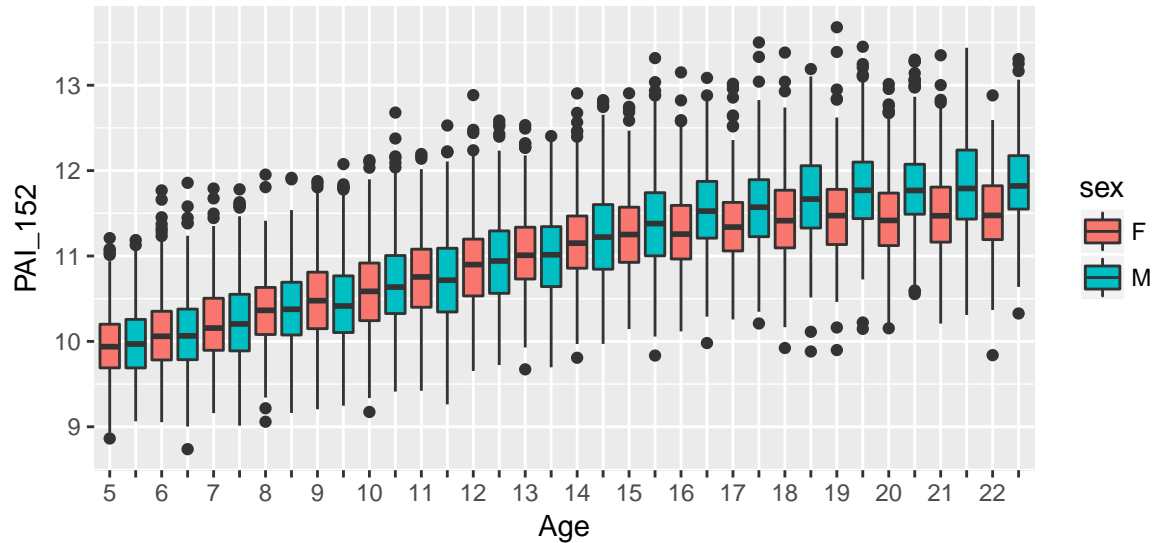

# Distributions of PAI\_153 by Sex and Age

ages from 5 years to 22 years old

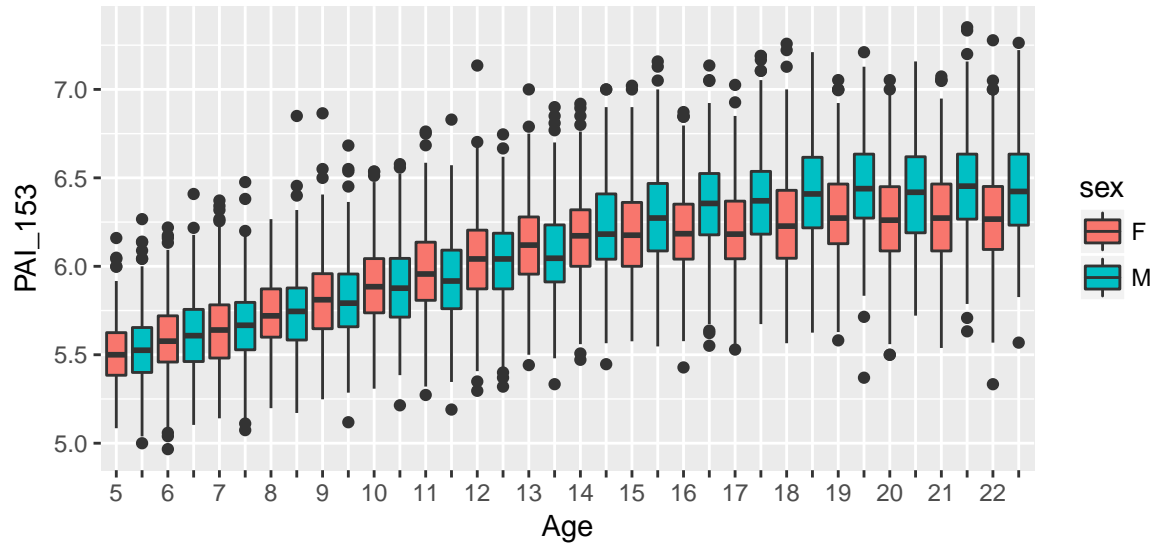

# Distributions of PAI\_154 by Sex and Age

ages from 5 years to 22 years old

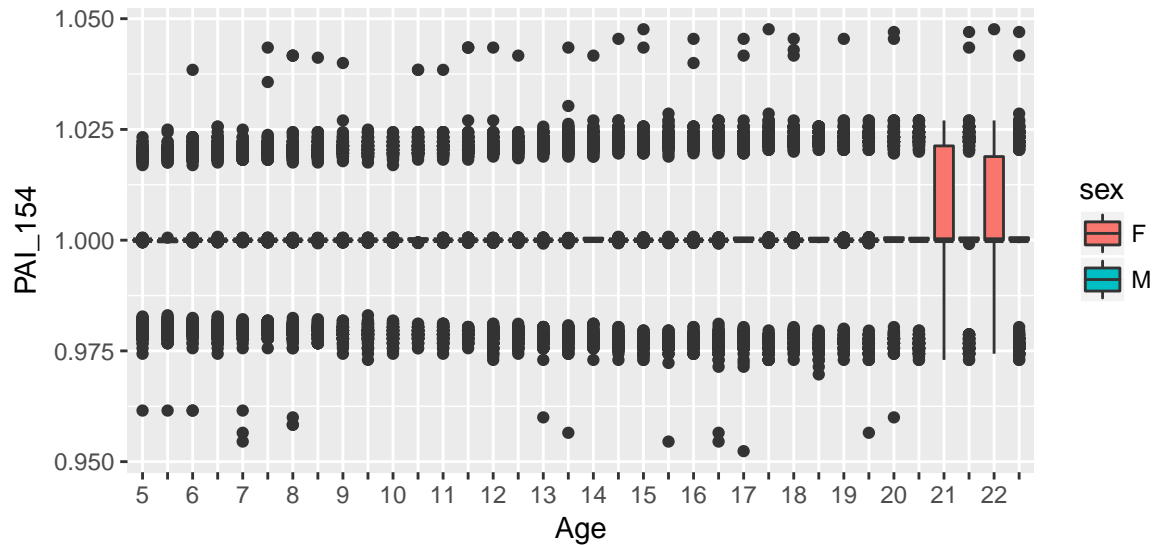

# Distributions of PAI\_155 by Sex and Age

ages from 5 years to 22 years old

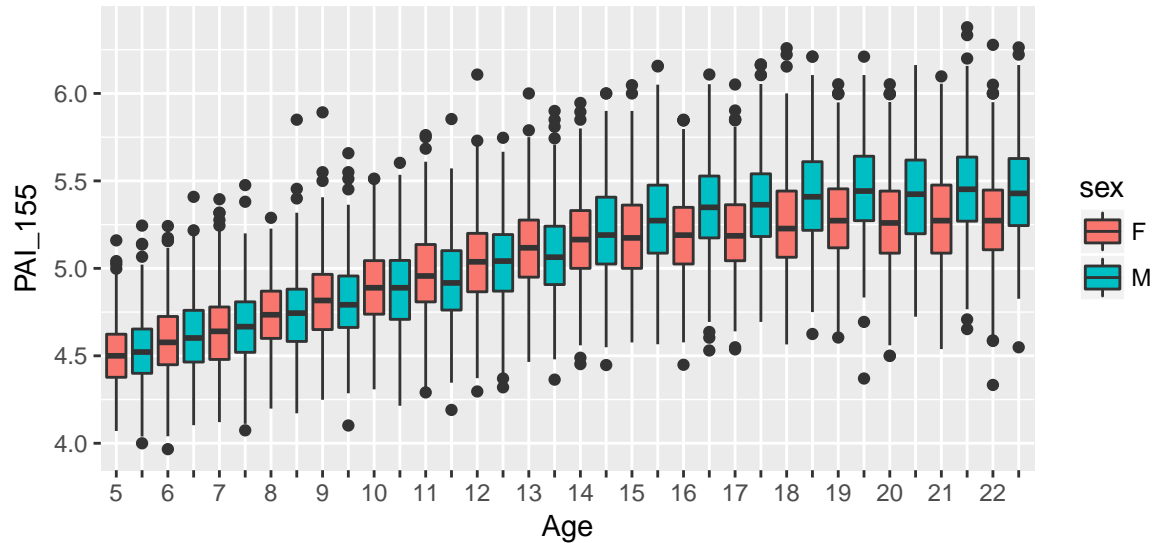

# Distributions of PAI\_156 by Sex and Age

ages from 5 years to 22 years old

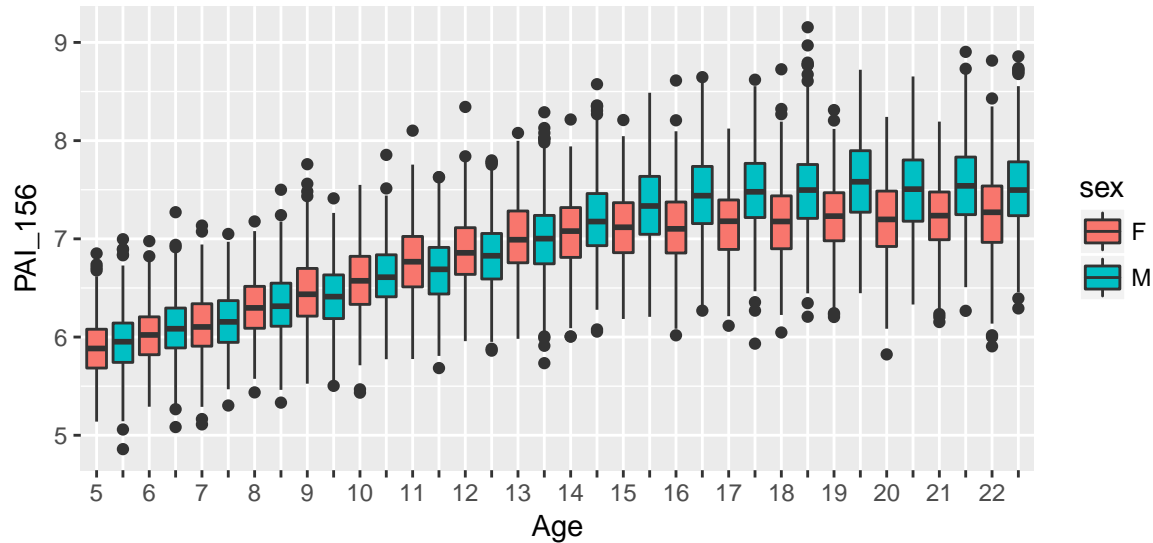

# Distributions of PAI\_157 by Sex and Age

ages from 5 years to 22 years old

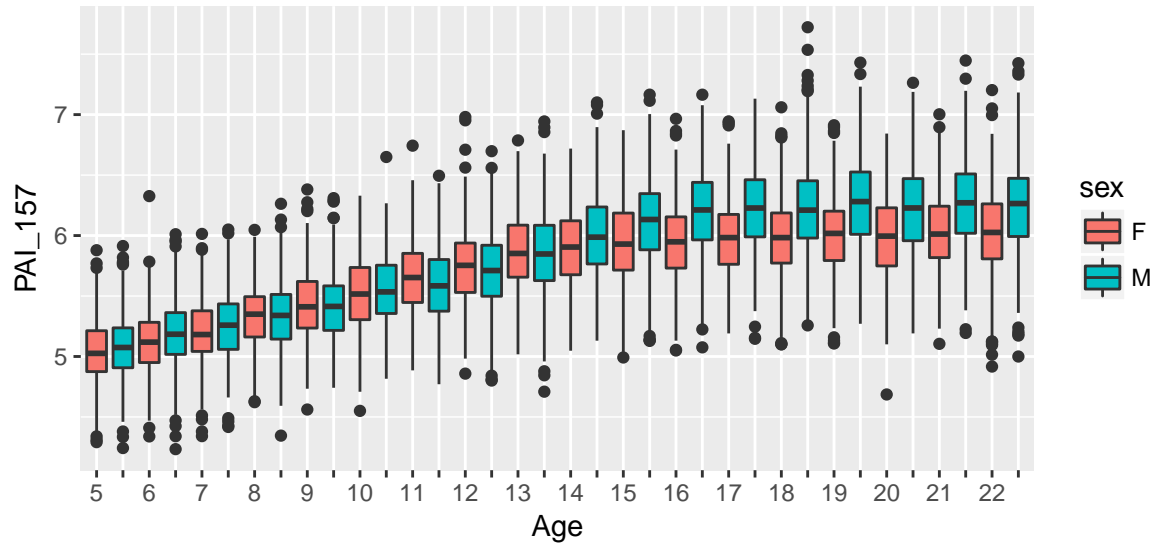

# Distributions of PAI\_158 by Sex and Age

ages from 5 years to 22 years old

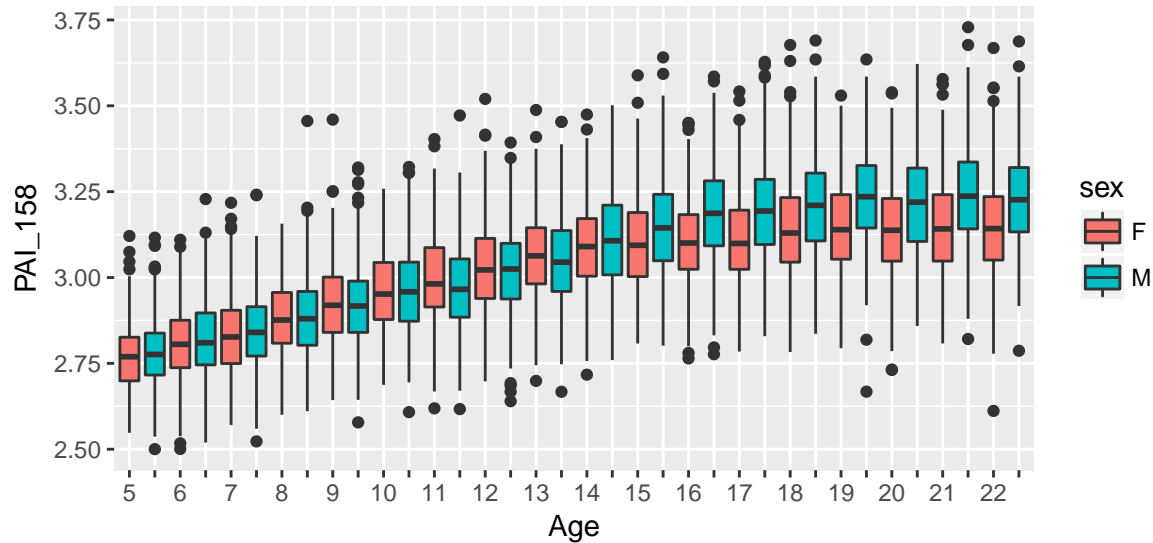

# Distributions of PAI\_159 by Sex and Age

ages from 5 years to 22 years old

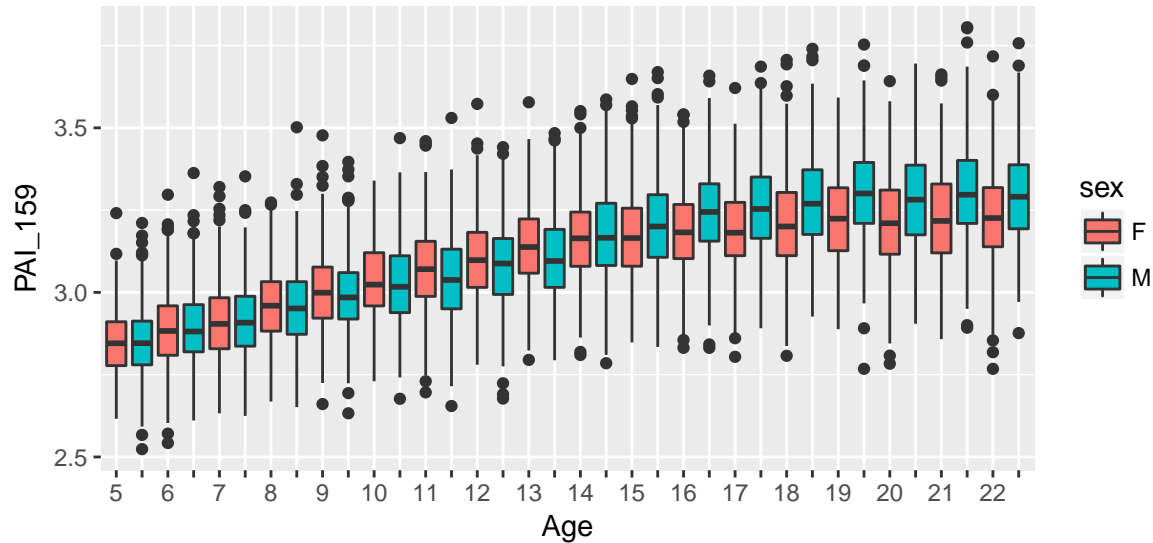

# Distributions of PAI\_15 by Sex and Age

ages from 5 years to 22 years old

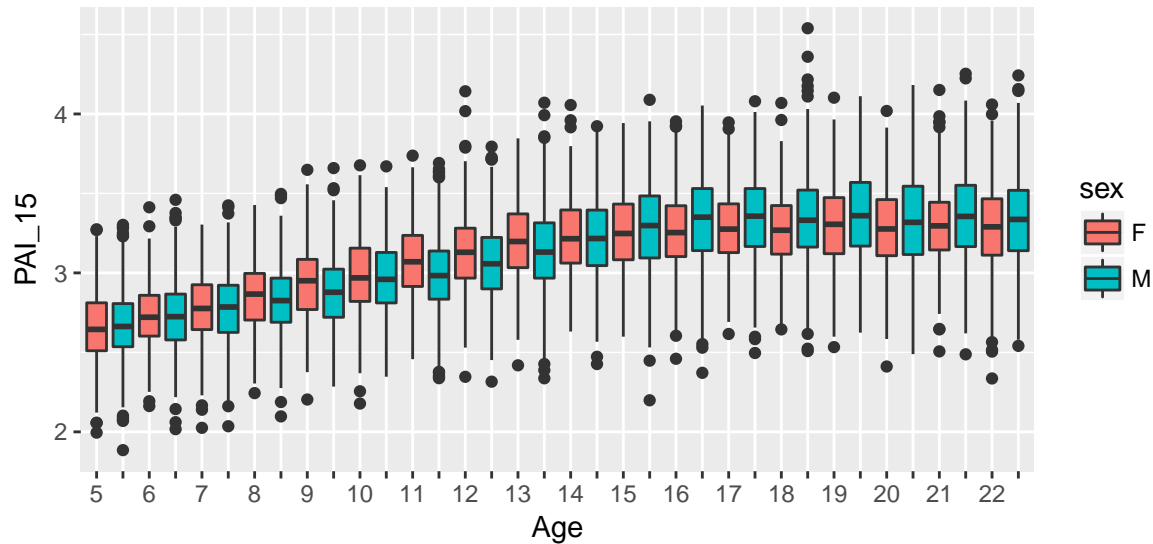

# Distributions of PAI\_160 by Sex and Age

ages from 5 years to 22 years old

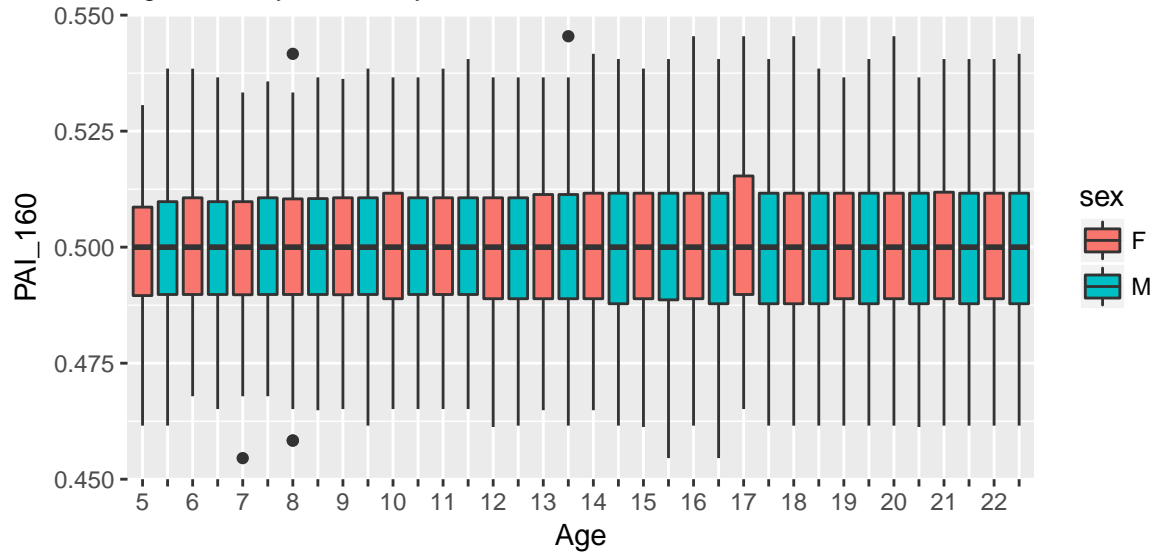

# Distributions of PAI\_161 by Sex and Age

ages from 5 years to 22 years old

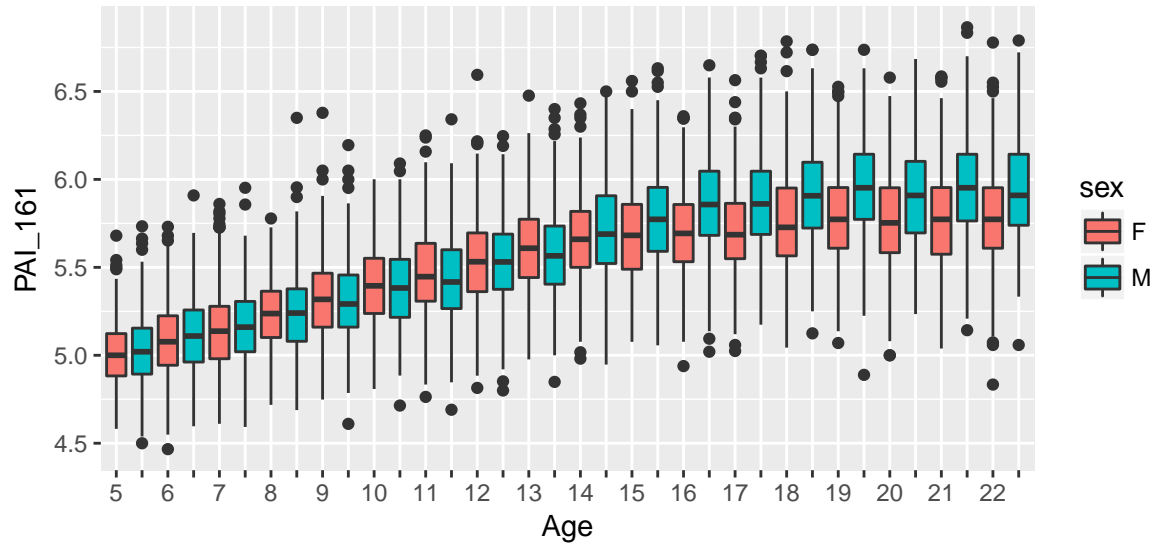

# Distributions of PAI\_162 by Sex and Age

ages from 5 years to 22 years old

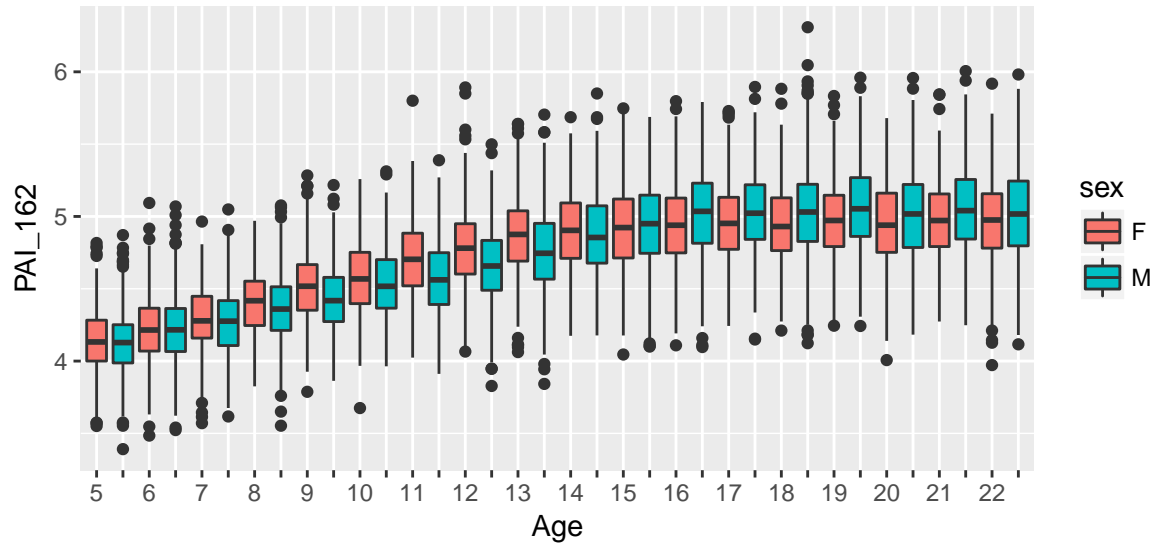

# Distributions of PAI\_163 by Sex and Age

ages from 5 years to 22 years old

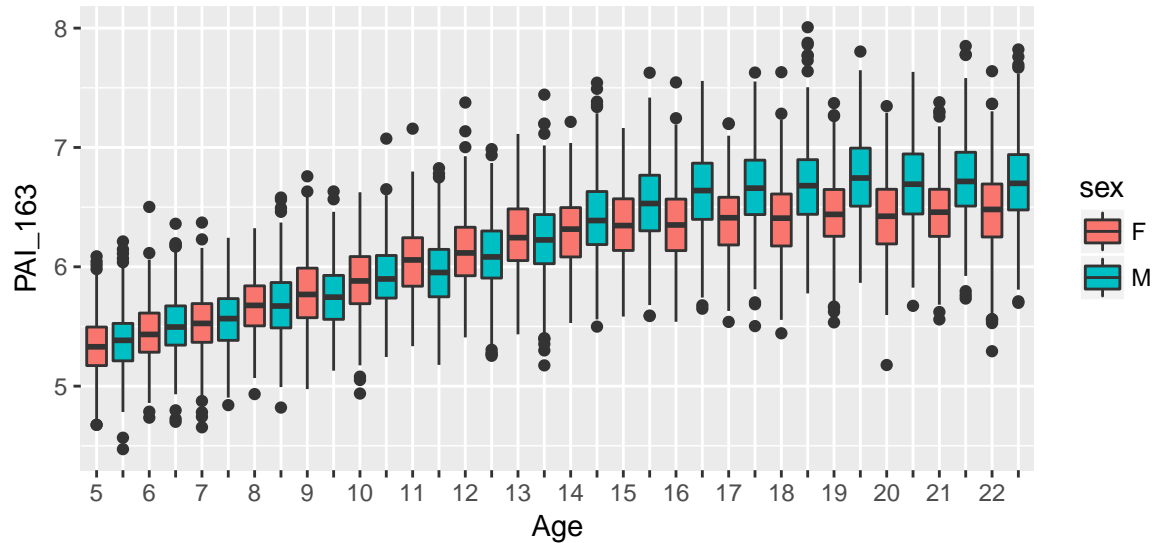

# Distributions of PAI\_164 by Sex and Age

ages from 5 years to 22 years old

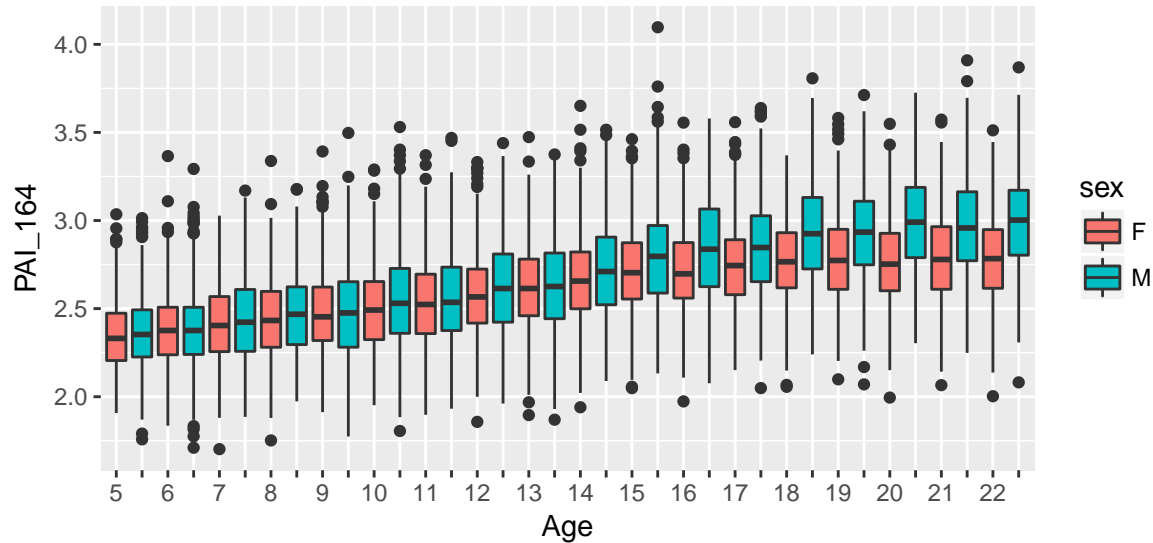

# Distributions of PAI\_165 by Sex and Age

ages from 5 years to 22 years old

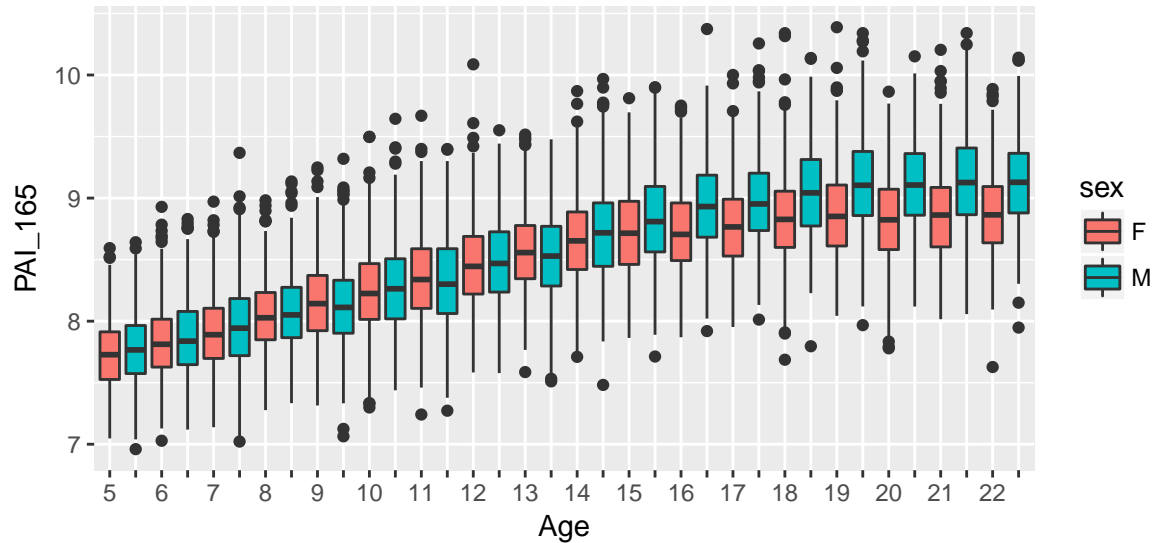

# Distributions of PAI\_166 by Sex and Age

ages from 5 years to 22 years old

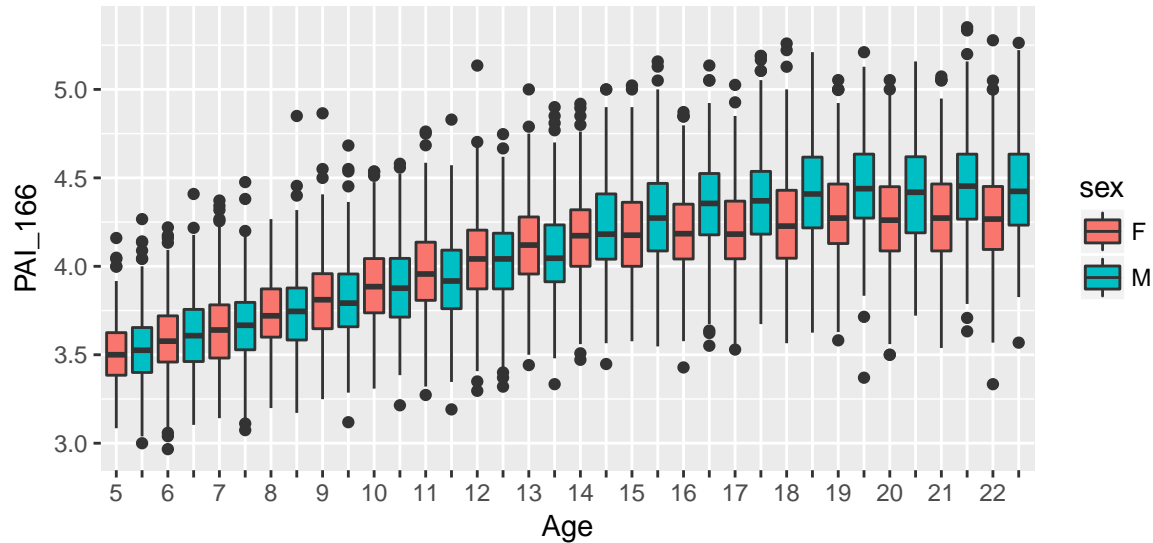

# Distributions of PAI\_167 by Sex and Age

ages from 5 years to 22 years old

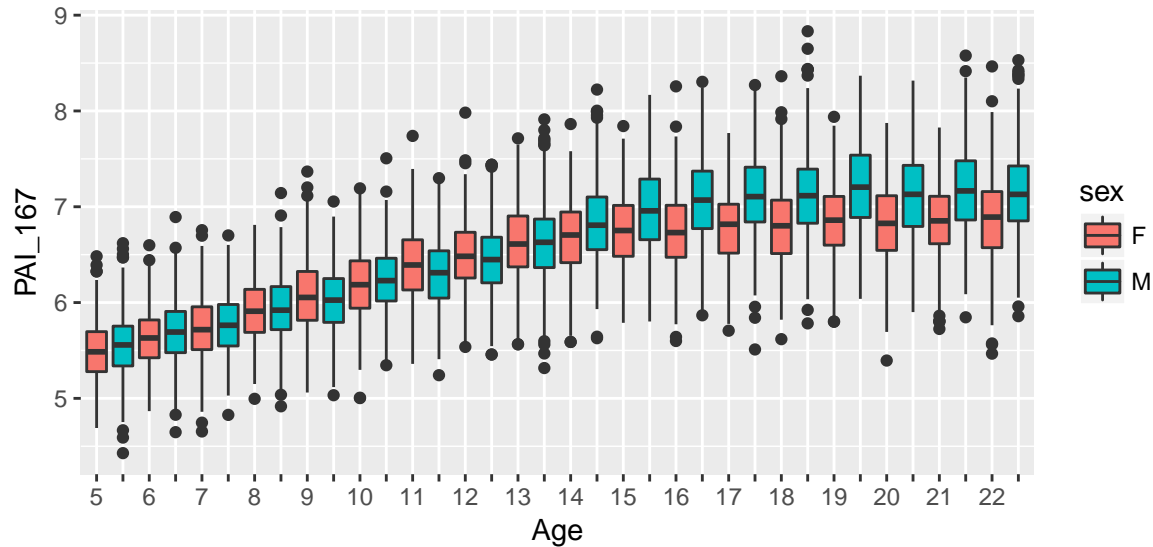

# Distributions of PAI\_168 by Sex and Age

ages from 5 years to 22 years old

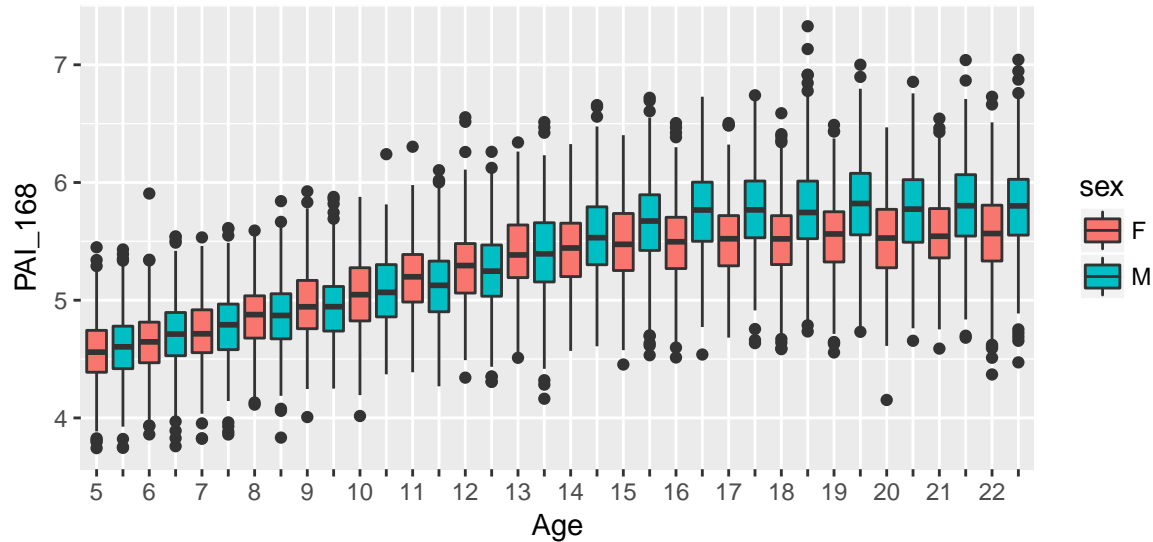

# Distributions of PAI\_169 by Sex and Age

ages from 5 years to 22 years old

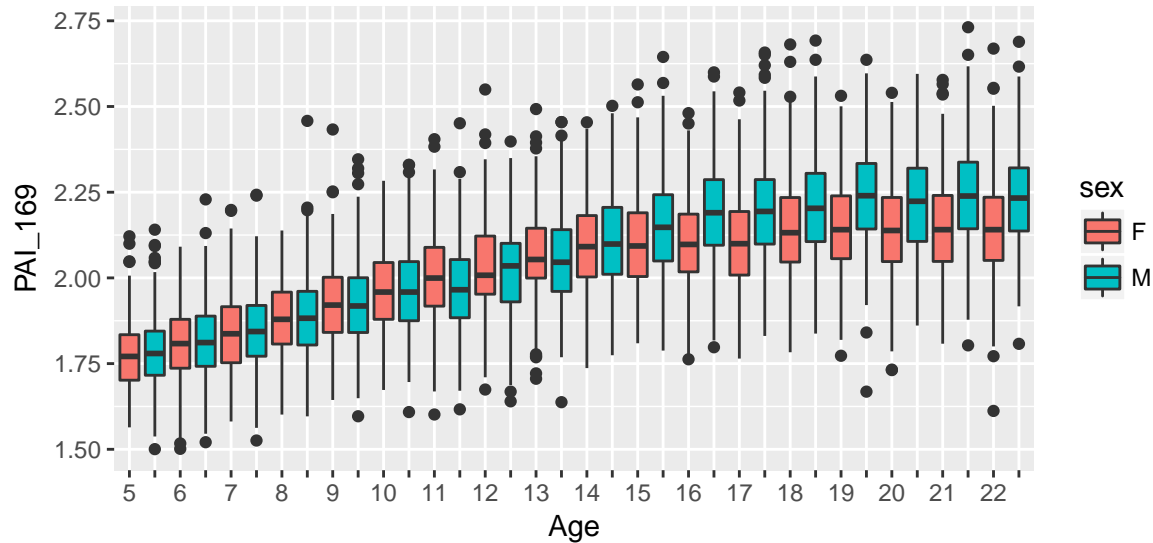

# Distributions of PAI\_16 by Sex and Age

ages from 5 years to 22 years old

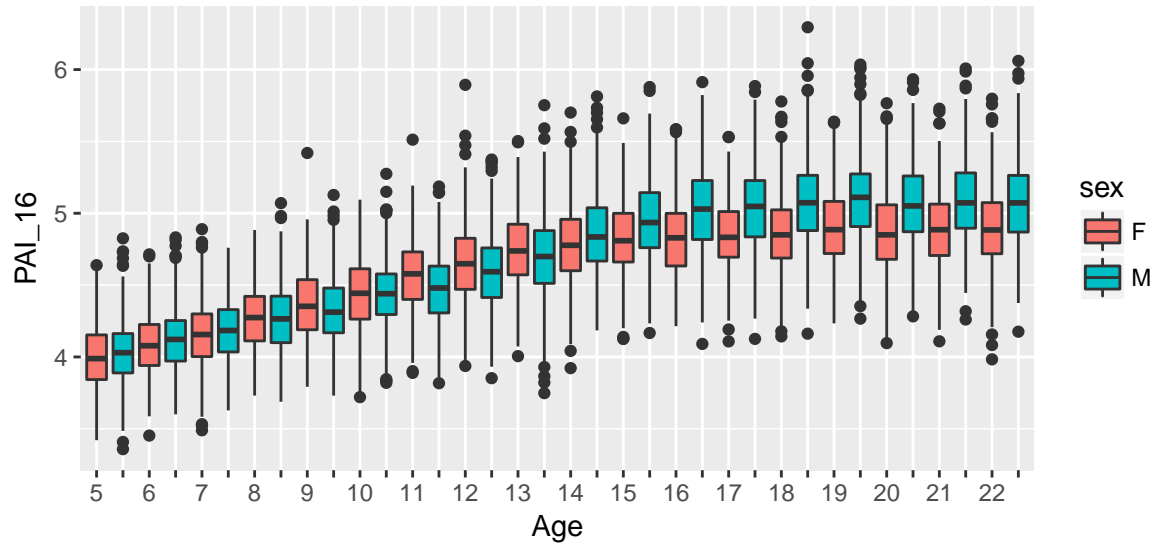

# Distributions of PAI\_170 by Sex and Age

ages from 5 years to 22 years old

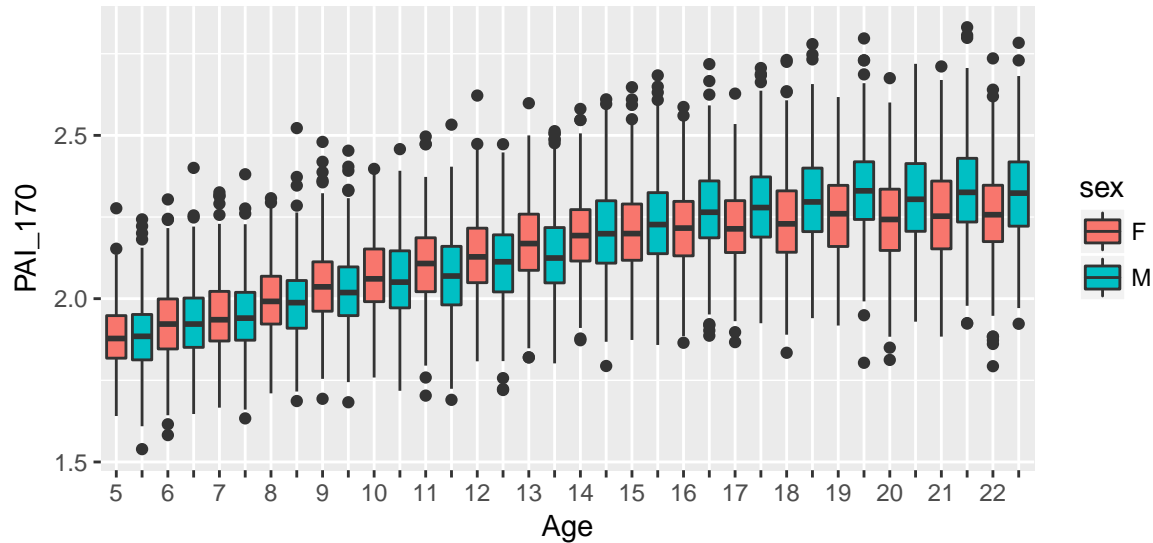

# Distributions of PAI\_171 by Sex and Age

ages from 5 years to 22 years old

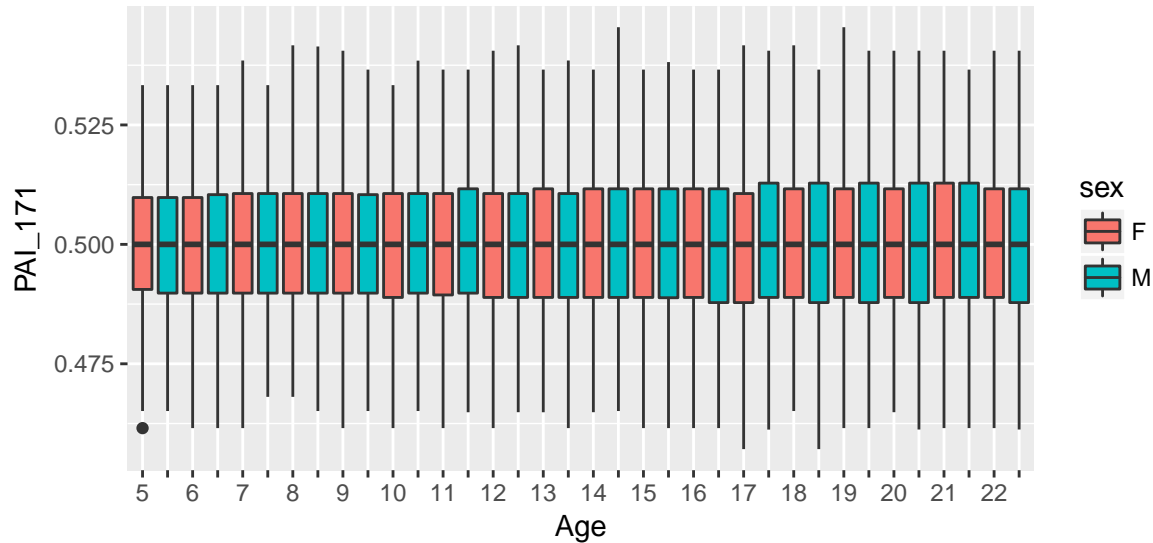

# Distributions of PAI\_172 by Sex and Age

ages from 5 years to 22 years old

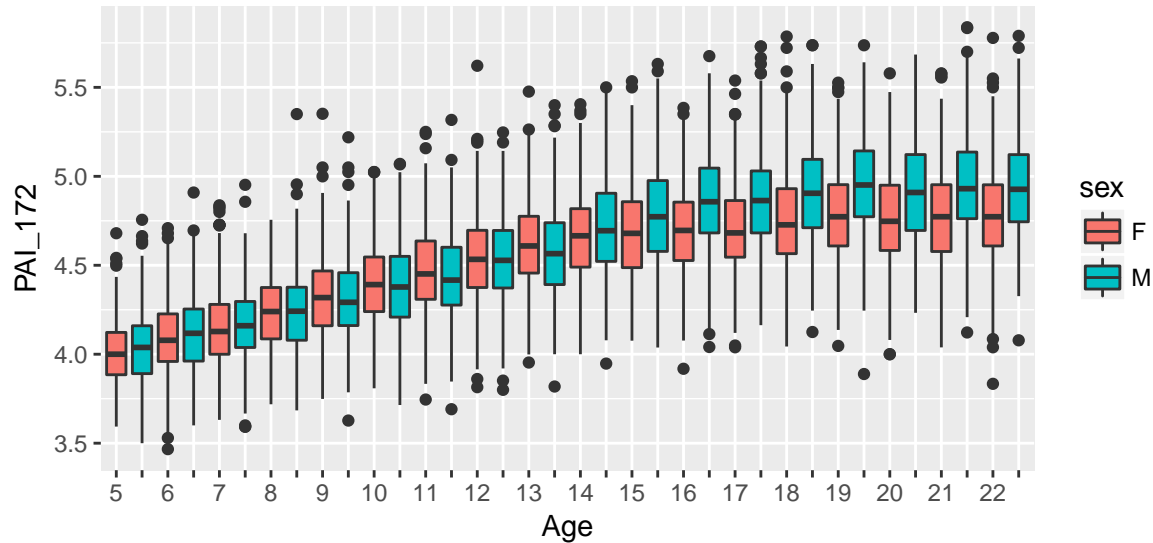

# Distributions of PAI\_173 by Sex and Age

ages from 5 years to 22 years old

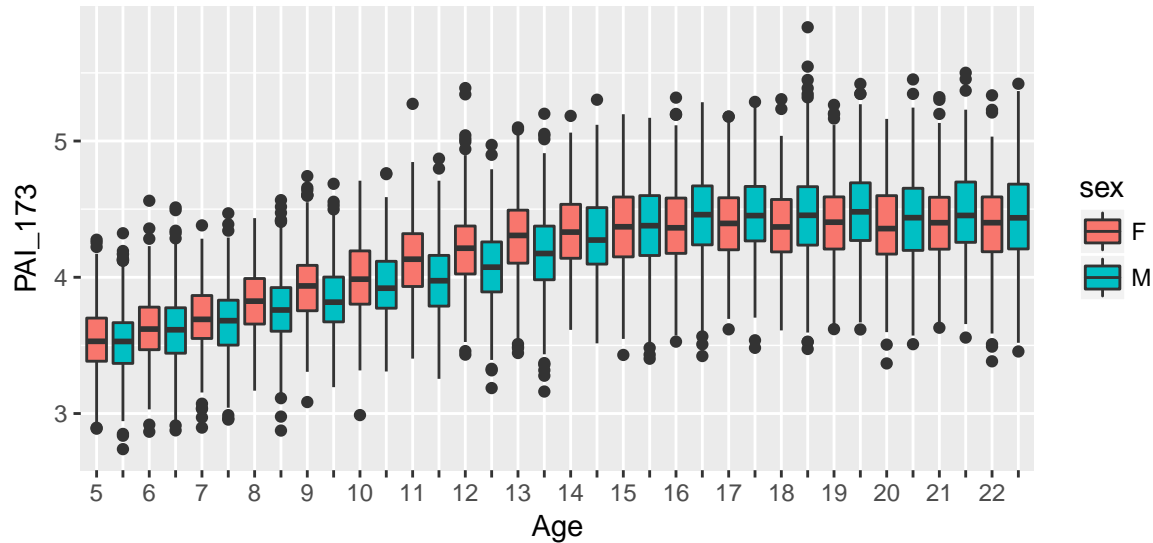

# Distributions of PAI\_174 by Sex and Age

ages from 5 years to 22 years old

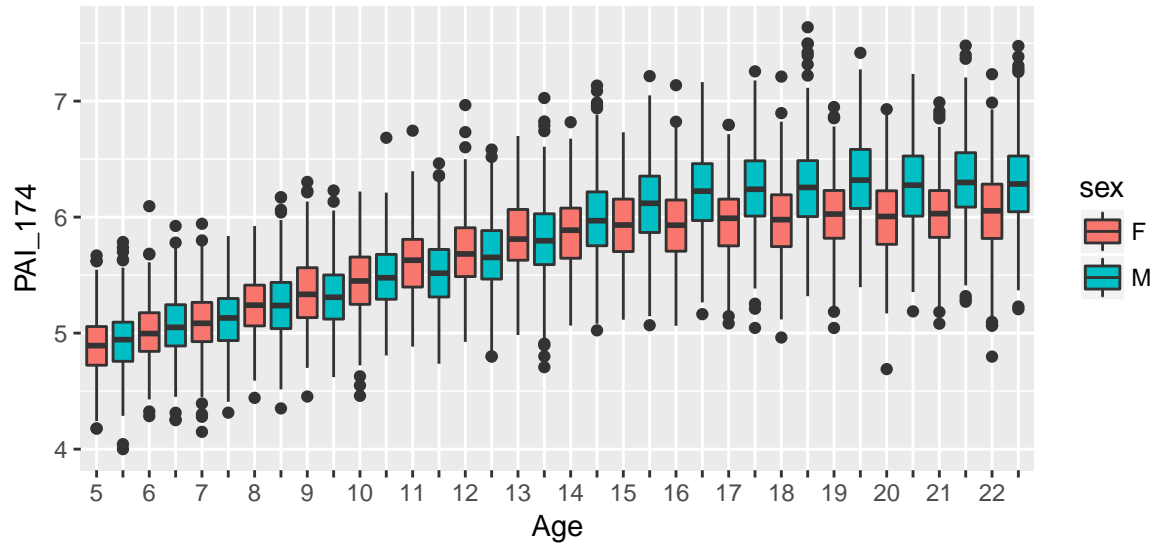

# Distributions of PAI\_175 by Sex and Age

ages from 5 years to 22 years old

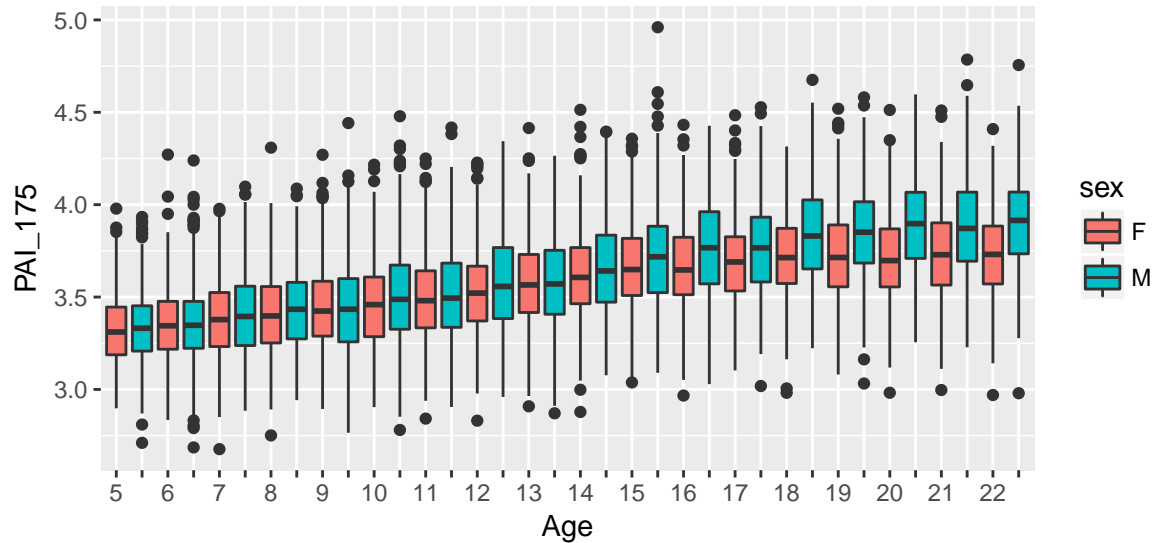

# Distributions of PAI\_176 by Sex and Age

ages from 5 years to 22 years old

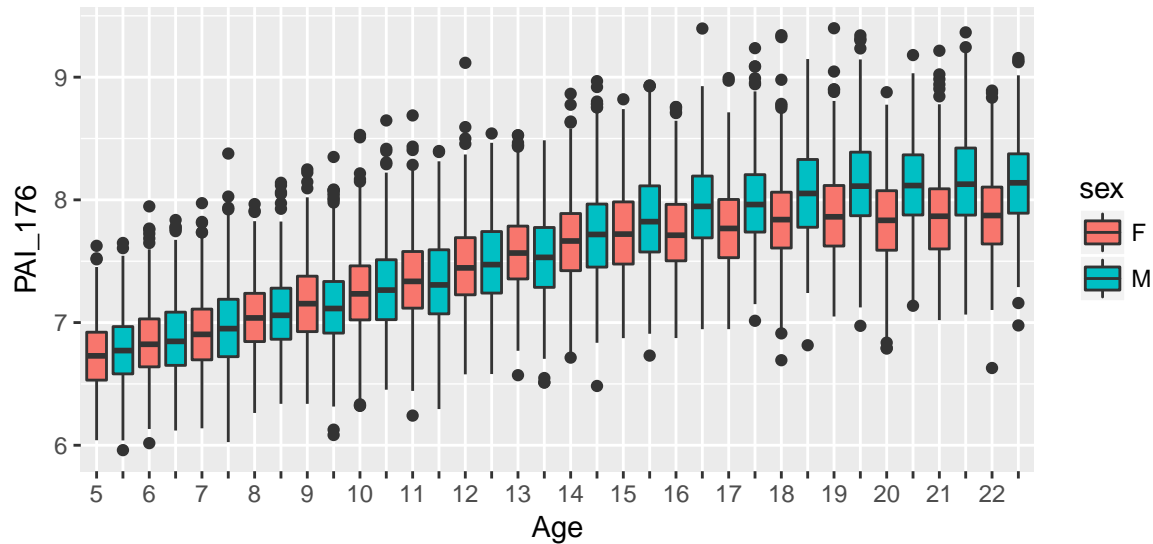

# Distributions of PAI\_177 by Sex and Age

ages from 5 years to 22 years old

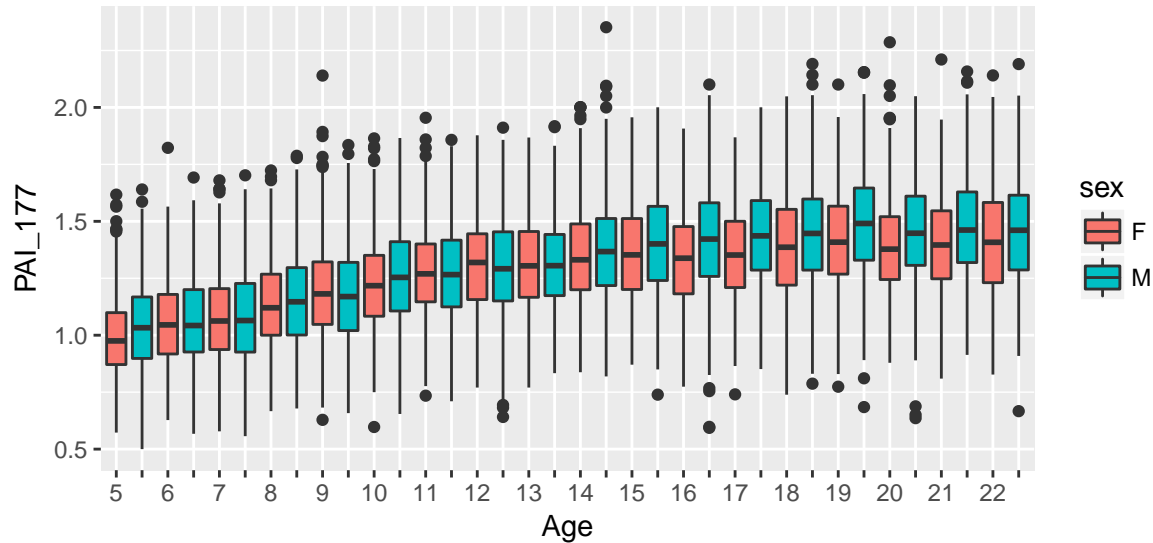

# Distributions of PAI\_178 by Sex and Age

ages from 5 years to 22 years old

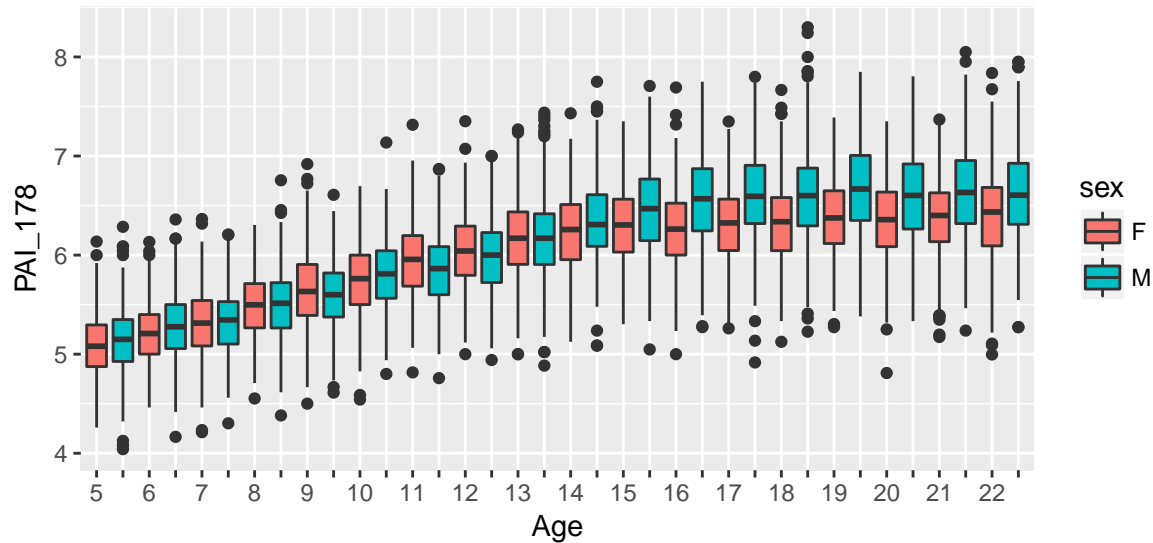

# Distributions of PAI\_179 by Sex and Age

ages from 5 years to 22 years old

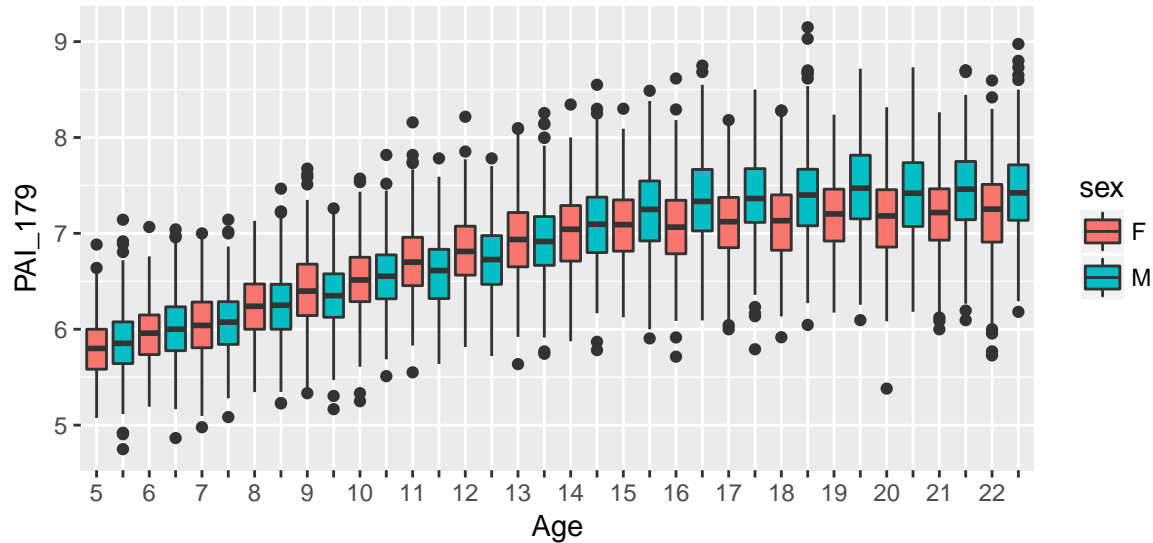

# Distributions of PAI\_17 by Sex and Age

ages from 5 years to 22 years old

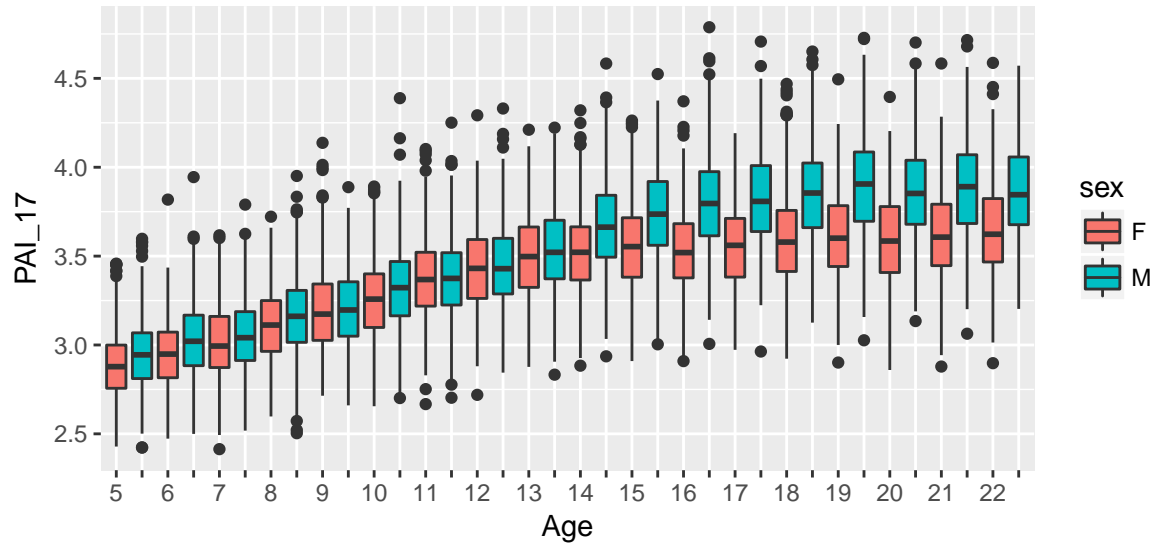

# Distributions of PAI\_180 by Sex and Age

ages from 5 years to 22 years old

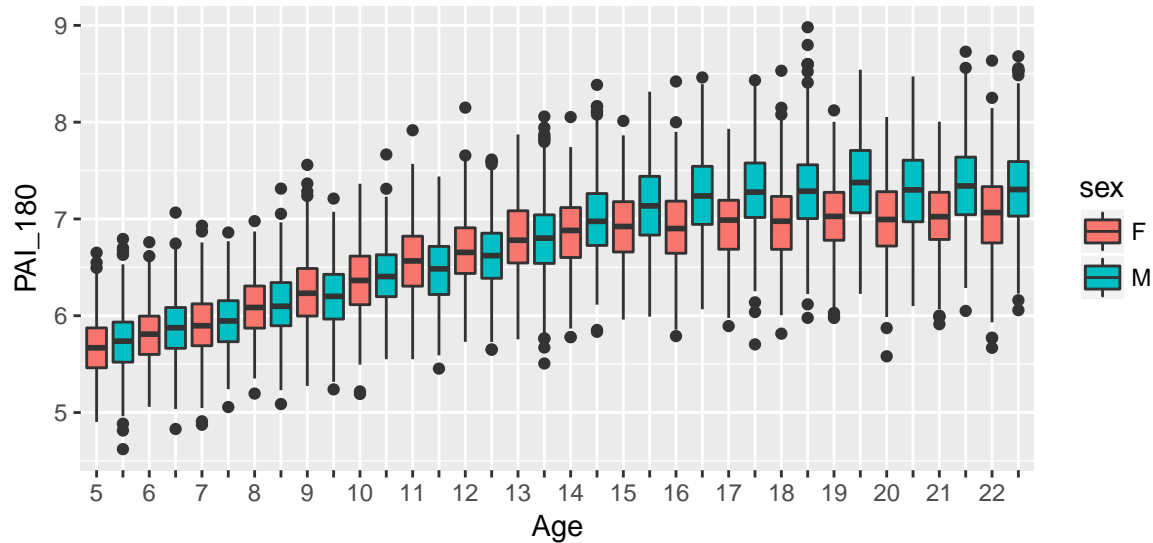

# Distributions of PAI\_181 by Sex and Age

ages from 5 years to 22 years old

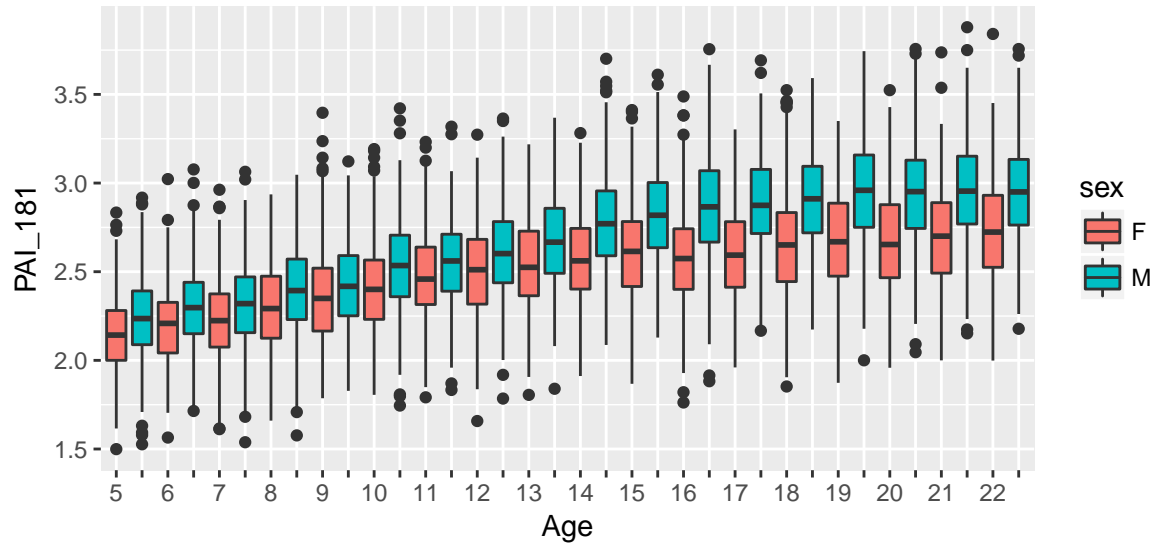

# Distributions of PAI\_182 by Sex and Age

ages from 5 years to 22 years old

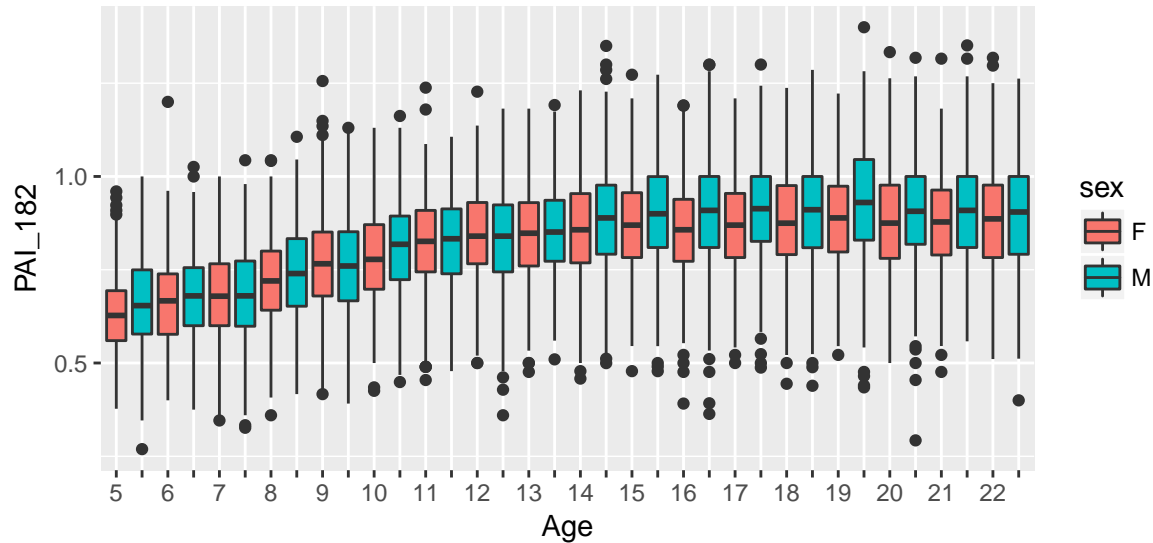

# Distributions of PAI\_183 by Sex and Age

ages from 5 years to 22 years old

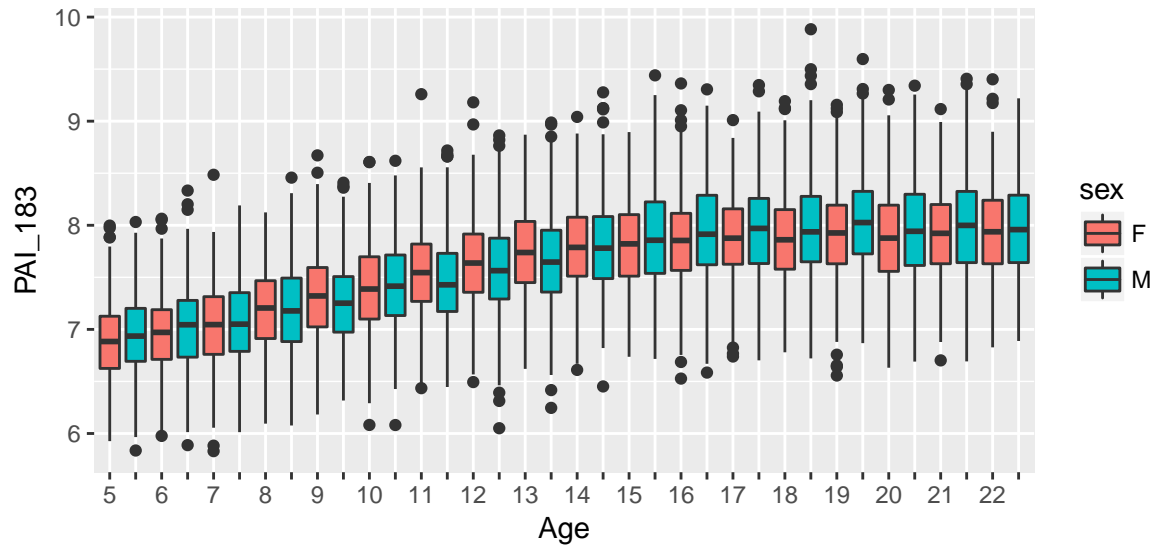

# Distributions of PAI\_184 by Sex and Age

ages from 5 years to 22 years old

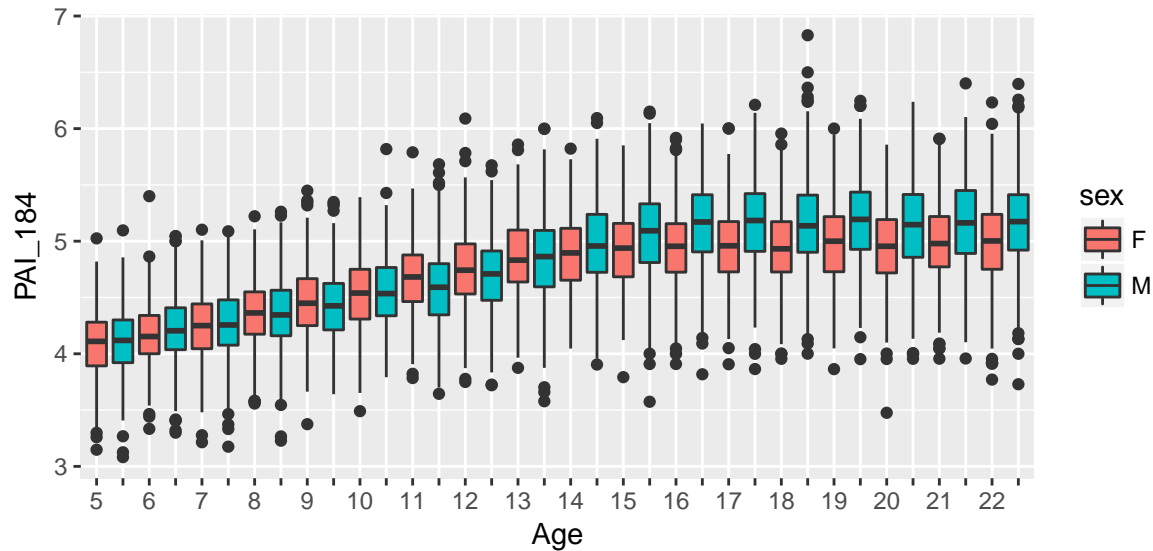

# Distributions of PAI\_185 by Sex and Age

ages from 5 years to 22 years old

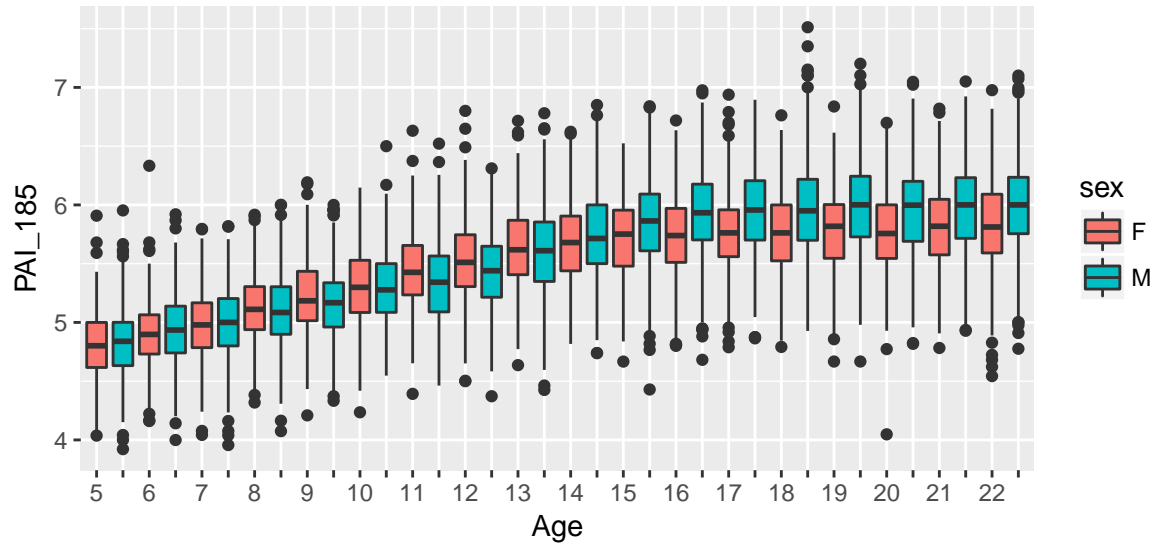

# Distributions of PAI\_186 by Sex and Age

ages from 5 years to 22 years old

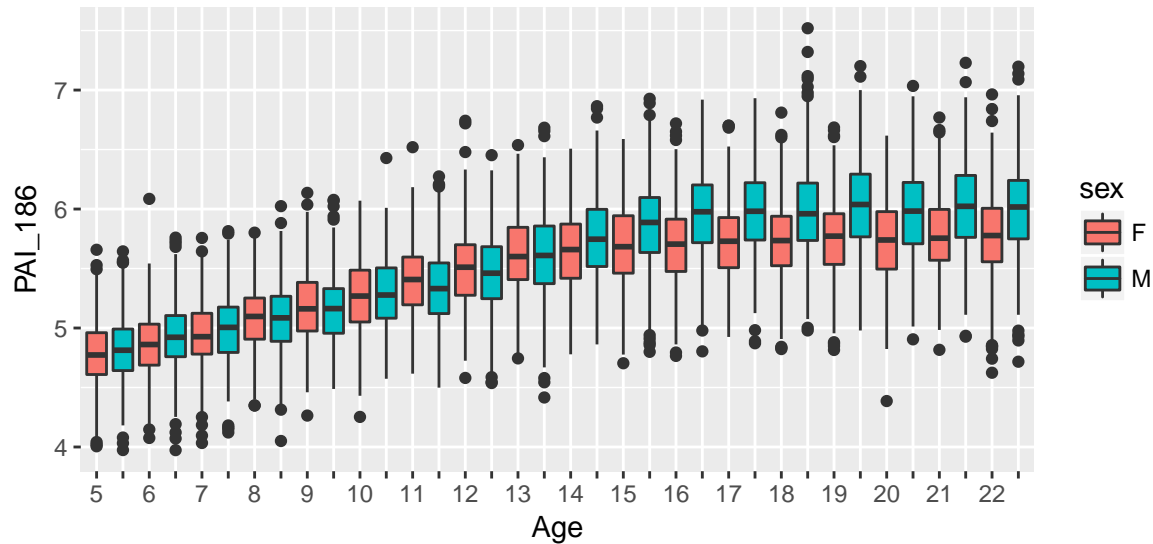

# Distributions of PAI\_187 by Sex and Age

ages from 5 years to 22 years old

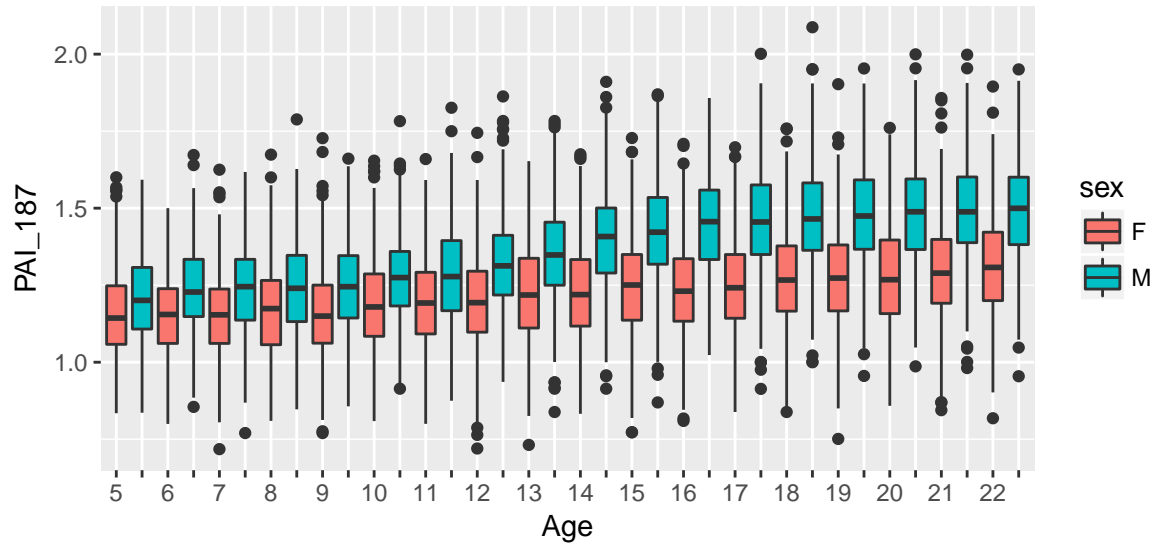

# Distributions of PAI\_188 by Sex and Age

ages from 5 years to 22 years old

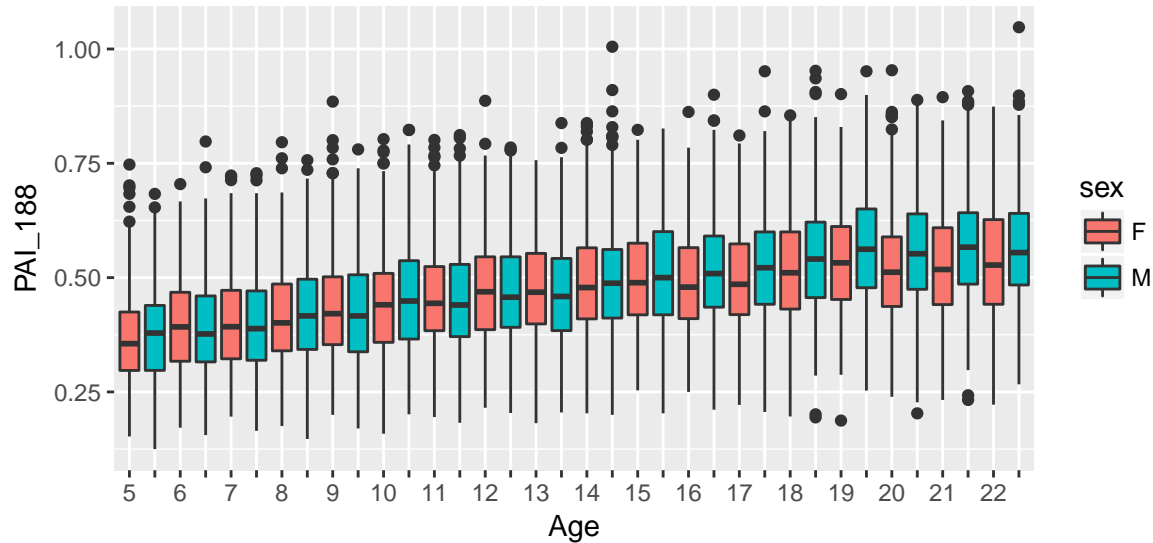

# Distributions of PAI\_189 by Sex and Age

ages from 5 years to 22 years old

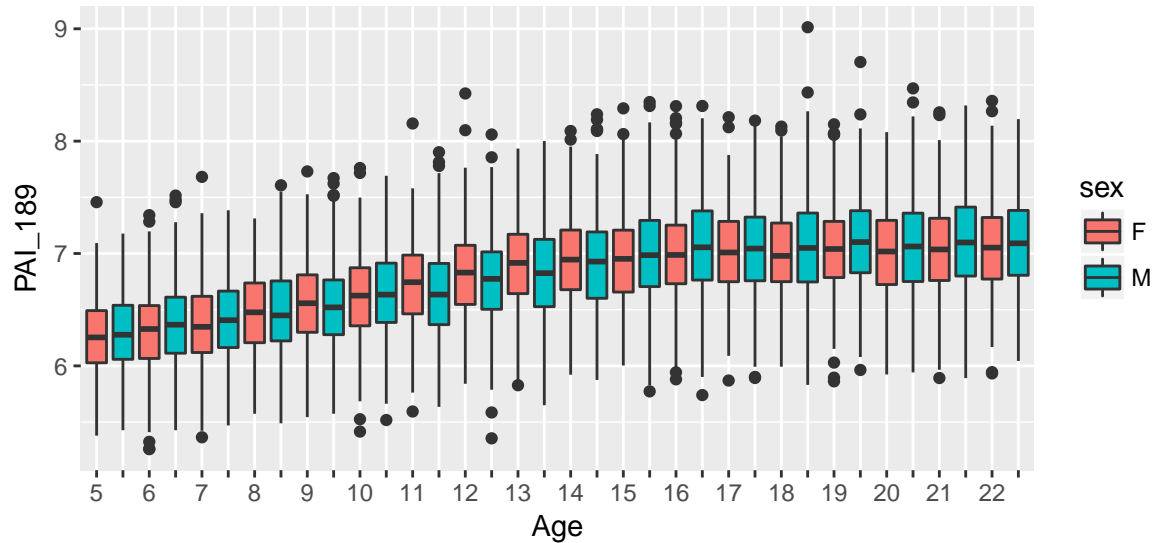

# Distributions of PAI\_18 by Sex and Age

ages from 5 years to 22 years old

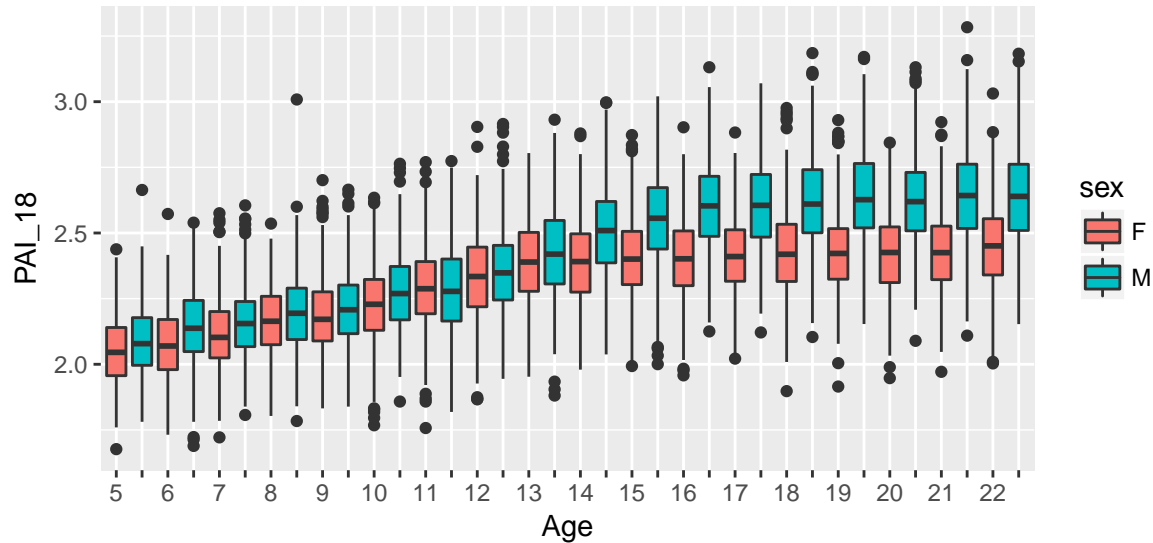

# Distributions of PAI\_190 by Sex and Age

ages from 5 years to 22 years old

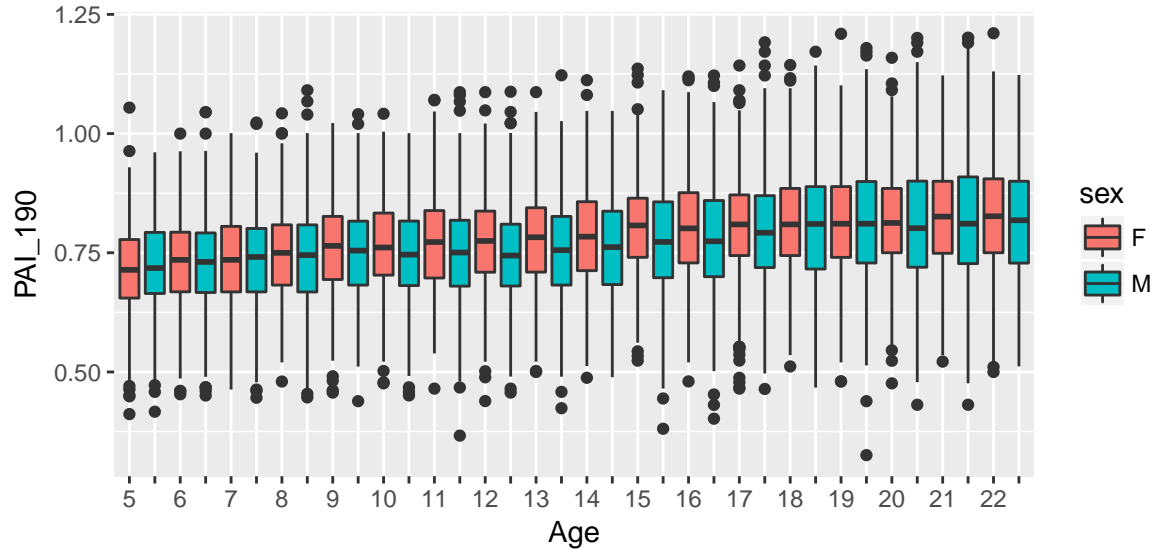

# Distributions of PAI\_191 by Sex and Age

ages from 5 years to 22 years old

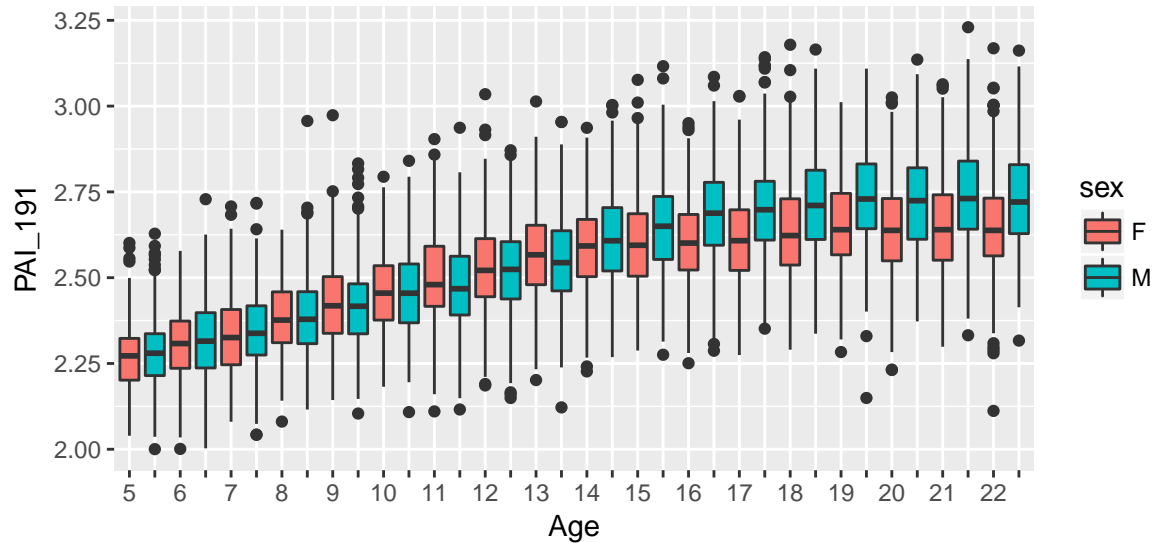

# Distributions of PAI\_192 by Sex and Age

ages from 5 years to 22 years old

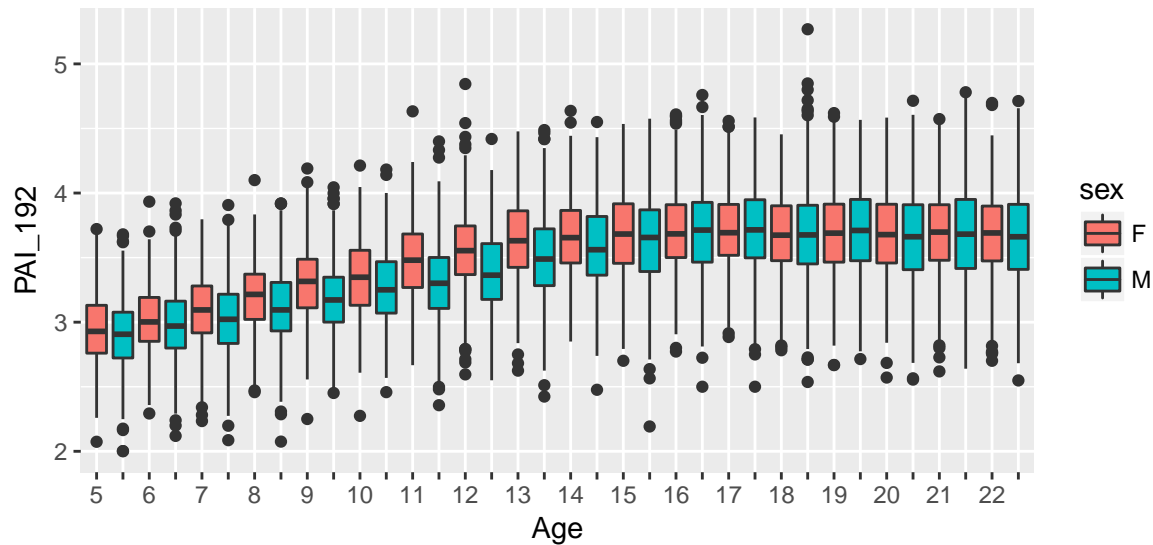

# Distributions of PAI\_193 by Sex and Age

ages from 5 years to 22 years old

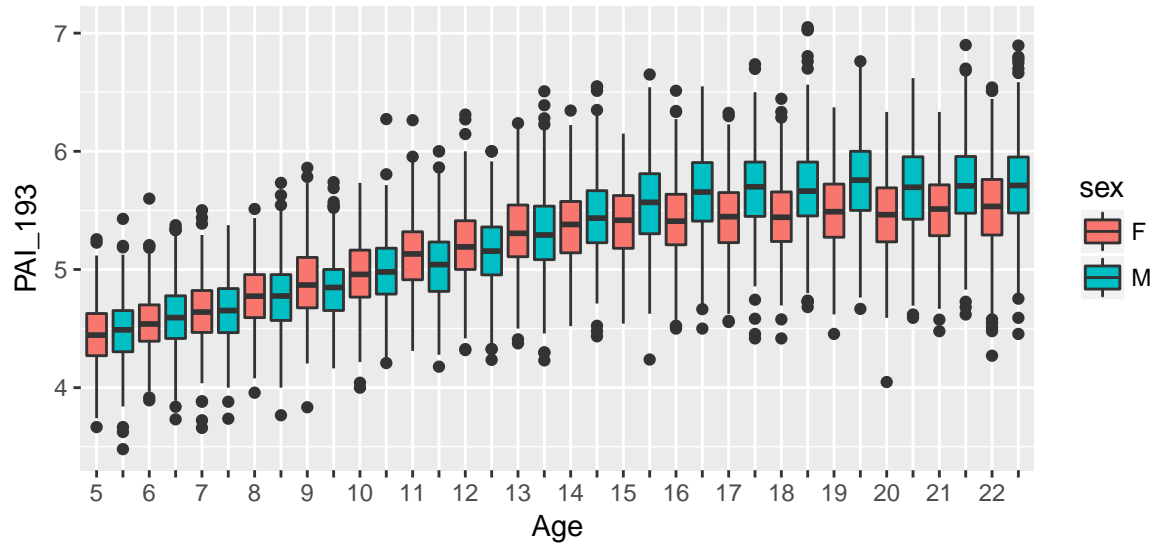

# Distributions of PAI\_194 by Sex and Age

ages from 5 years to 22 years old

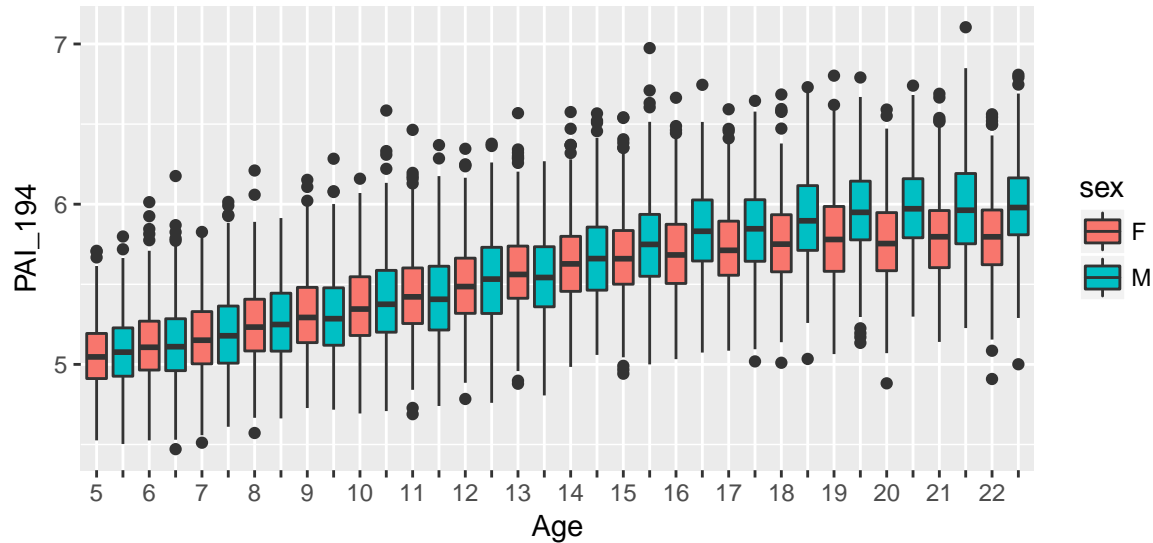

# Distributions of PAI\_195 by Sex and Age

ages from 5 years to 22 years old

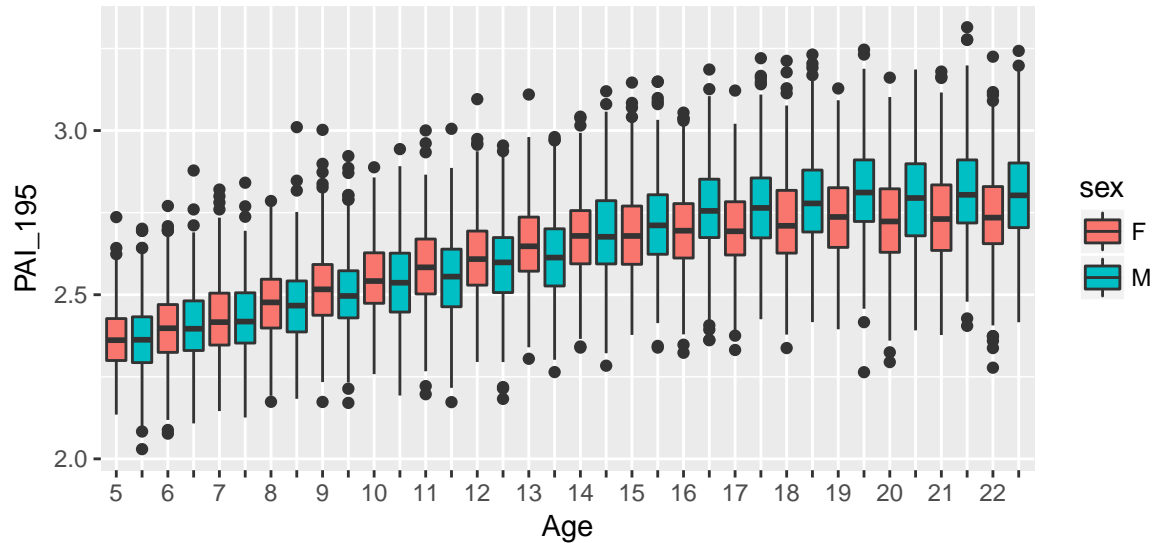

# Distributions of PAI\_196 by Sex and Age

ages from 5 years to 22 years old

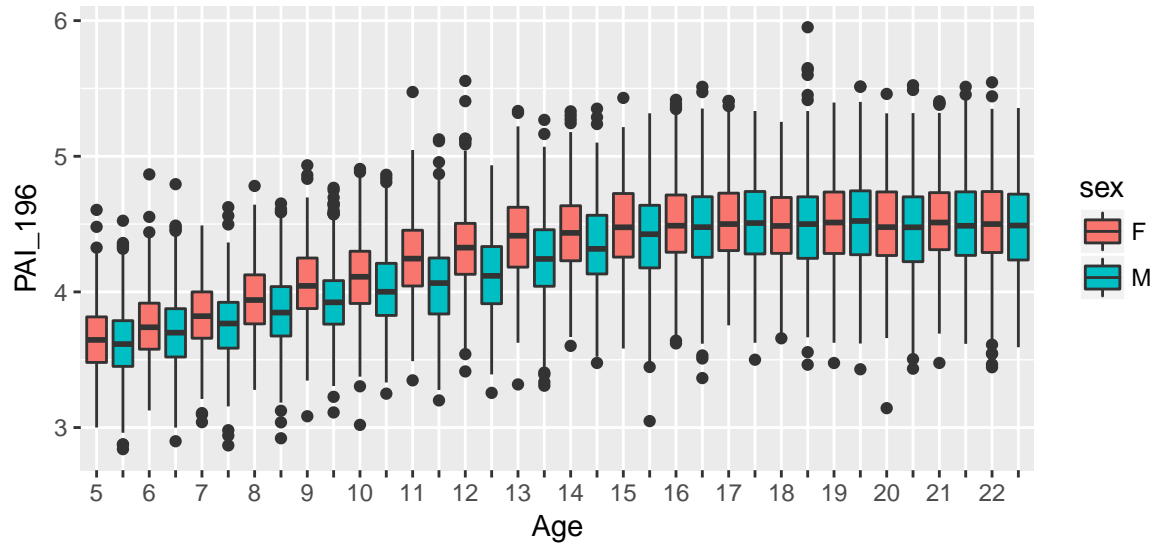

# Distributions of PAI\_197 by Sex and Age

ages from 5 years to 22 years old

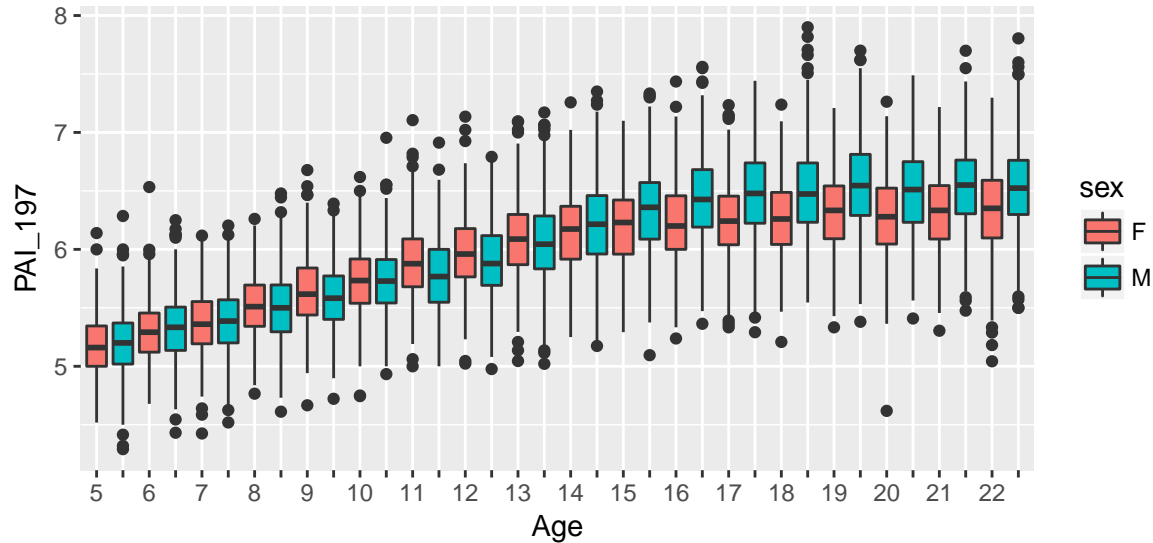

# Distributions of PAI\_198 by Sex and Age

ages from 5 years to 22 years old

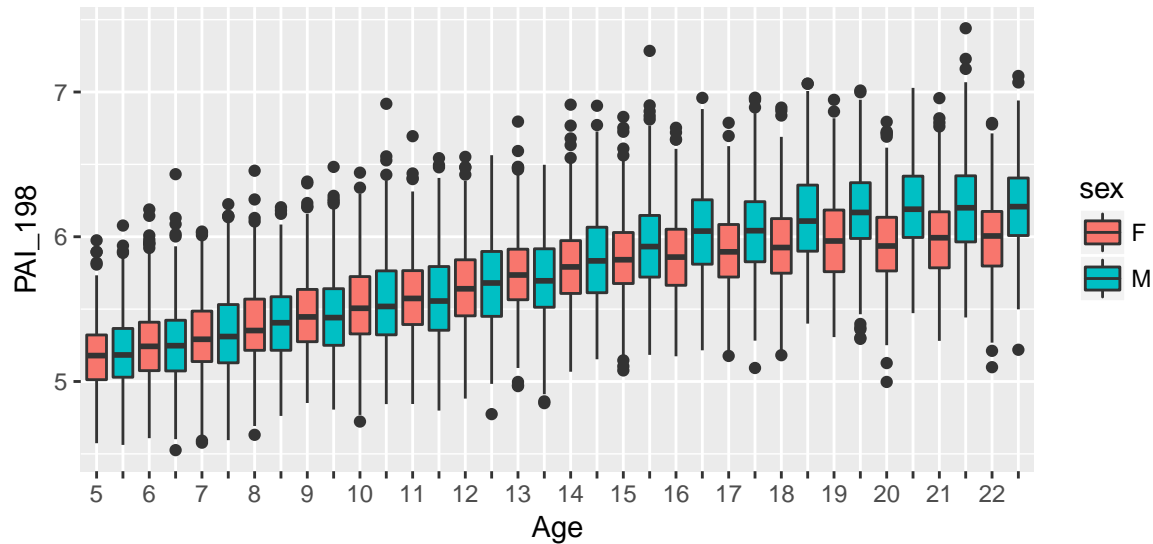

# Distributions of PAI\_199 by Sex and Age

ages from 5 years to 22 years old

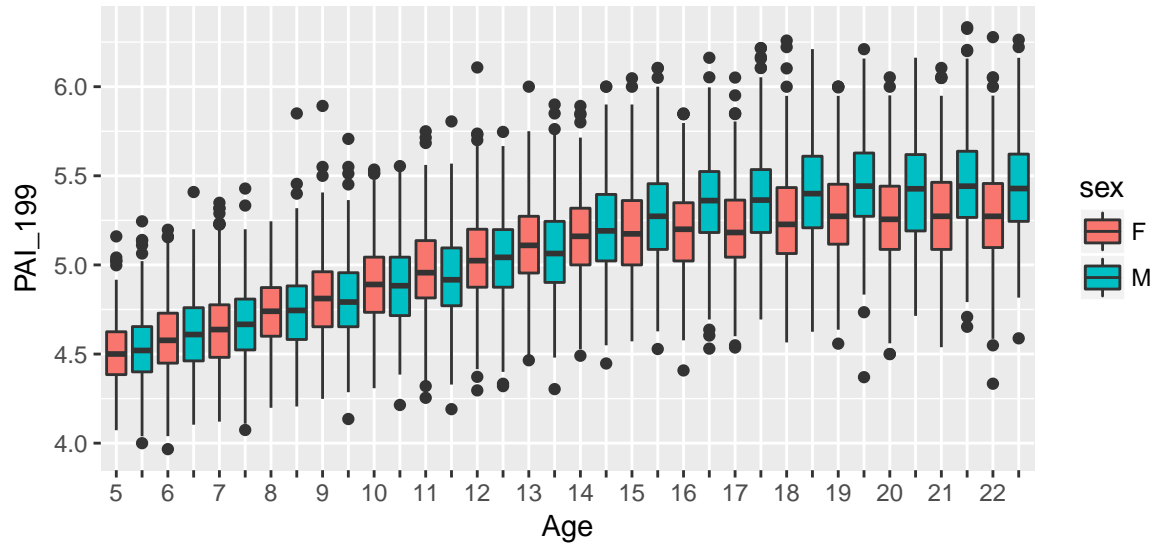

# Distributions of PAI\_19 by Sex and Age

ages from 5 years to 22 years old

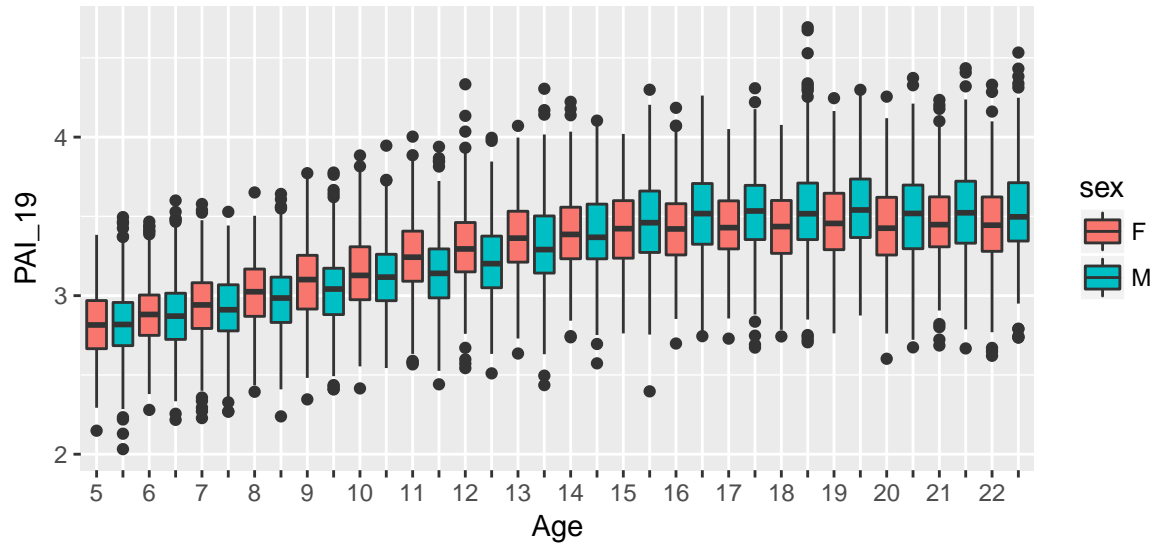

# Distributions of PAI\_1 by Sex and Age

ages from 5 years to 22 years old

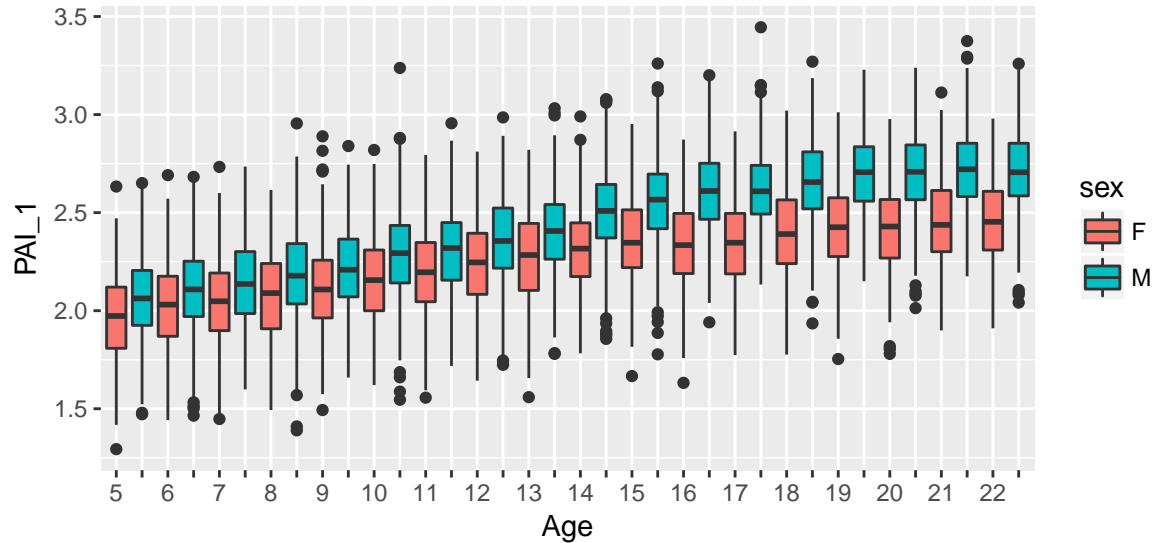

# Distributions of PAI\_200 by Sex and Age

ages from 5 years to 22 years old

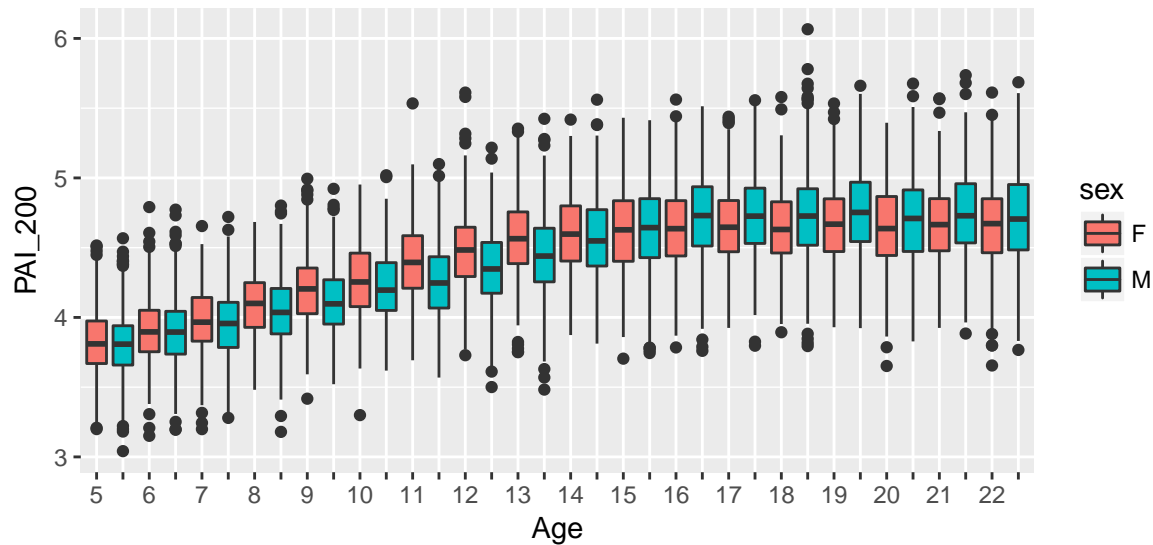

# Distributions of PAI\_201 by Sex and Age

ages from 5 years to 22 years old

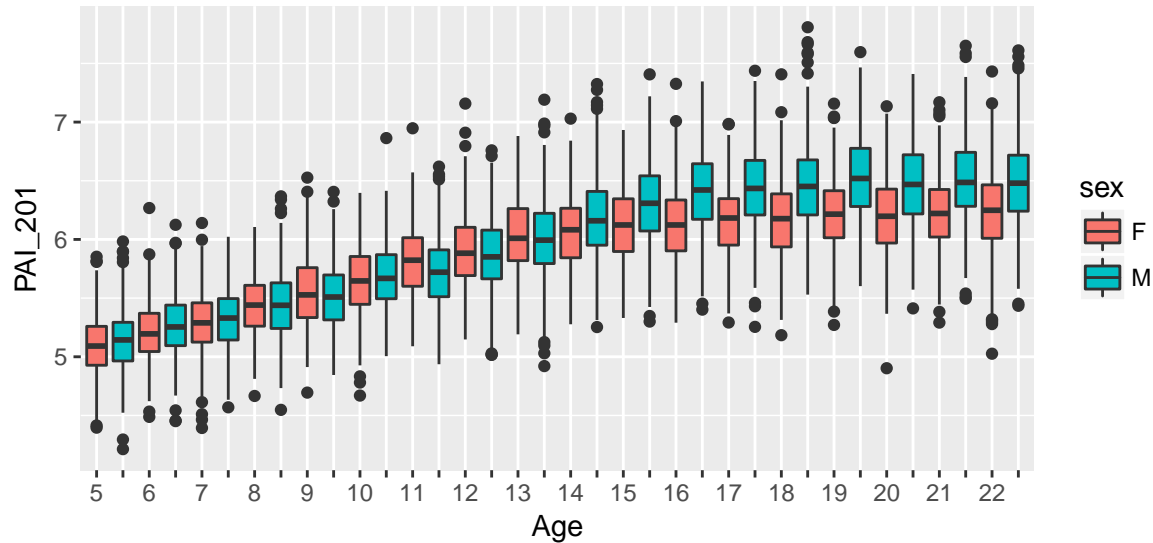

# Distributions of PAI\_202 by Sex and Age

ages from 5 years to 22 years old

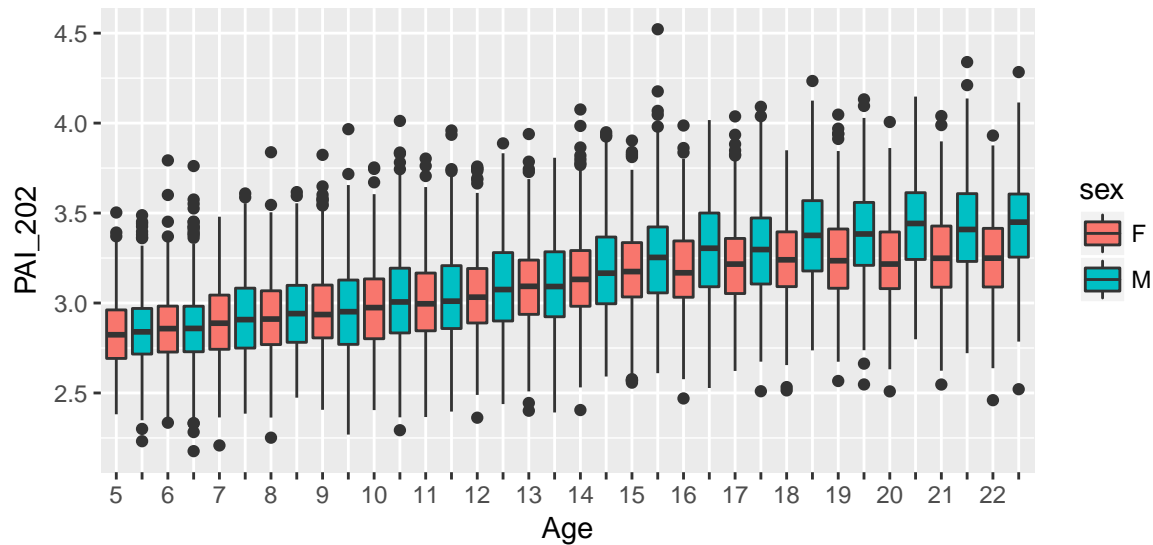

# Distributions of PAI\_203 by Sex and Age

ages from 5 years to 22 years old

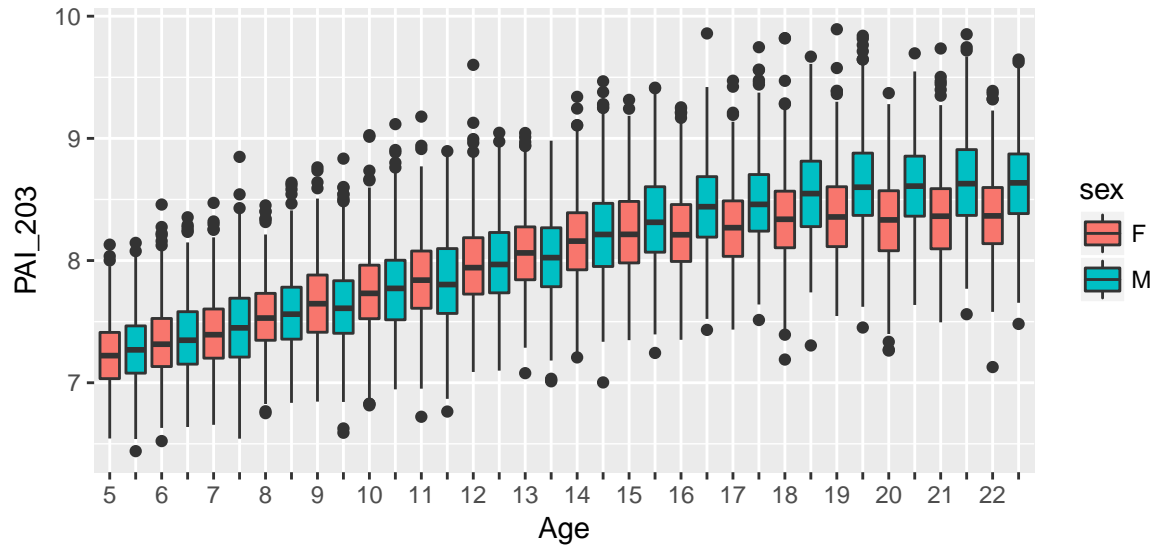

# Distributions of PAI\_204 by Sex and Age

ages from 5 years to 22 years old

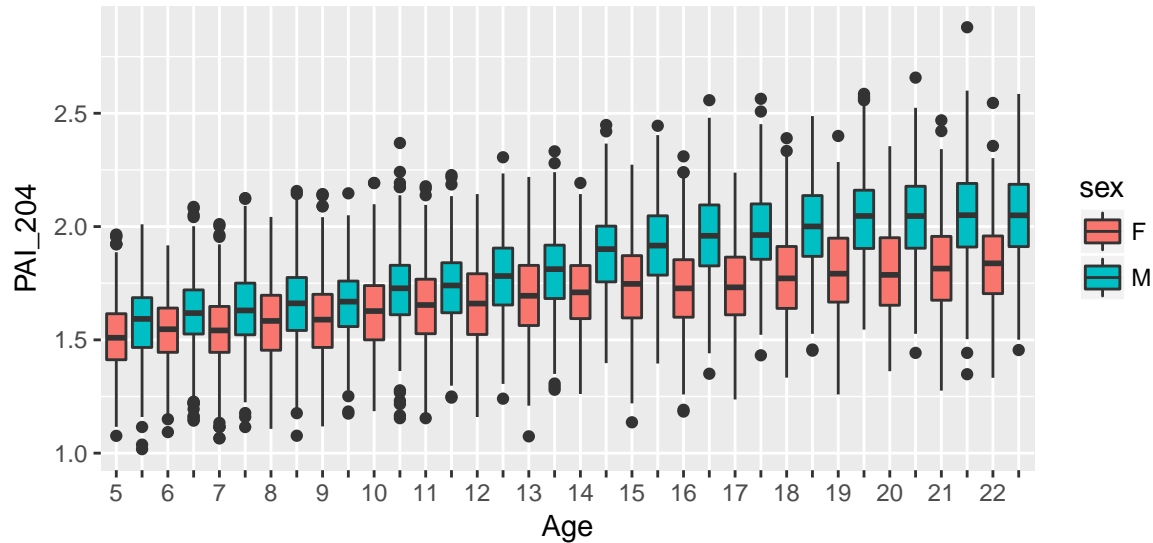

# Distributions of PAI\_205 by Sex and Age

ages from 5 years to 22 years old

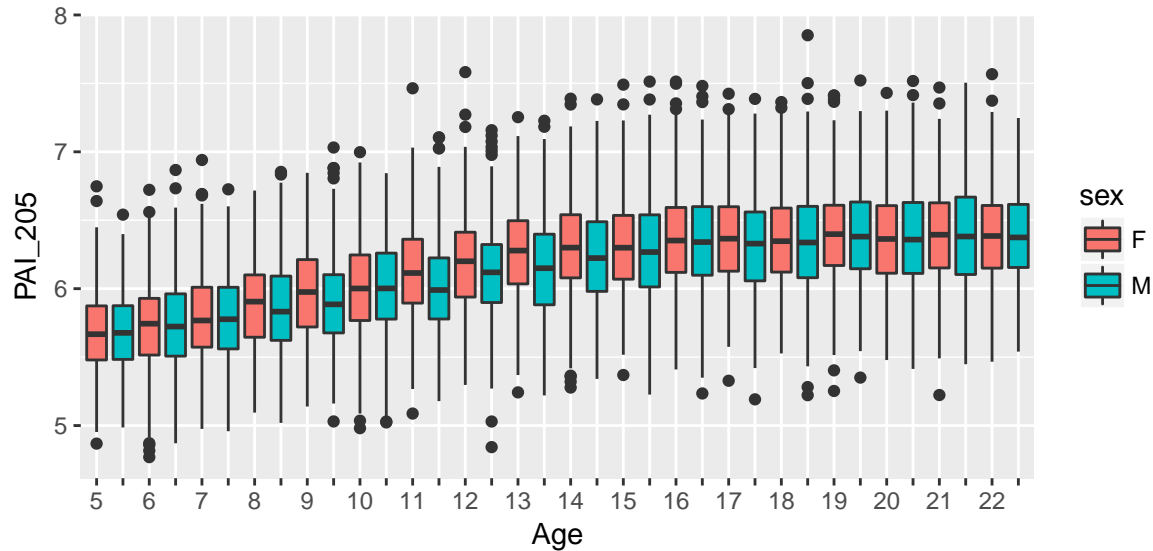

# Distributions of PAI\_206 by Sex and Age

ages from 5 years to 22 years old

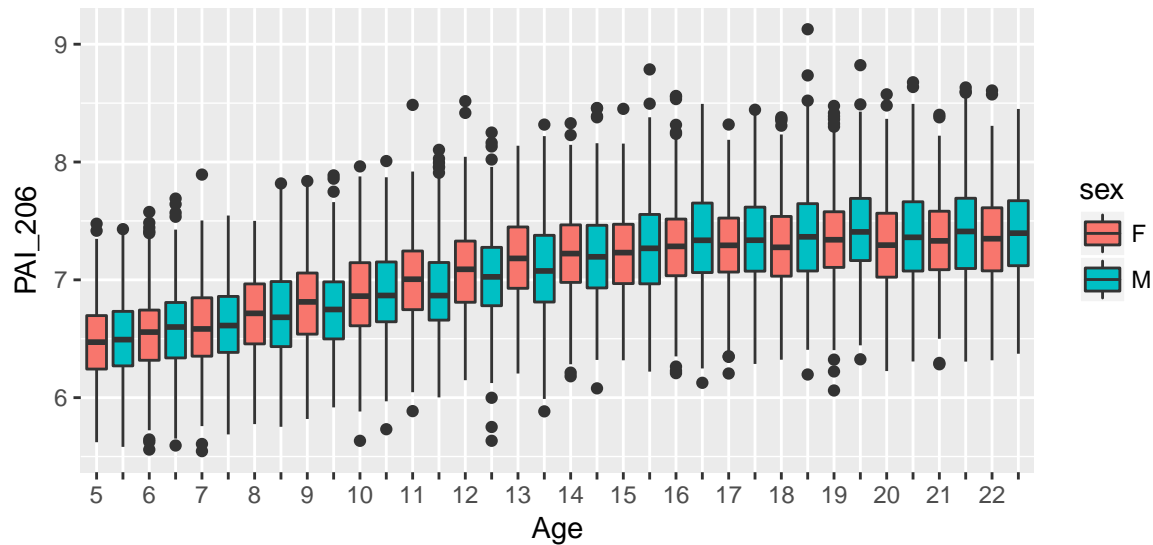

# Distributions of PAI\_207 by Sex and Age

ages from 5 years to 22 years old

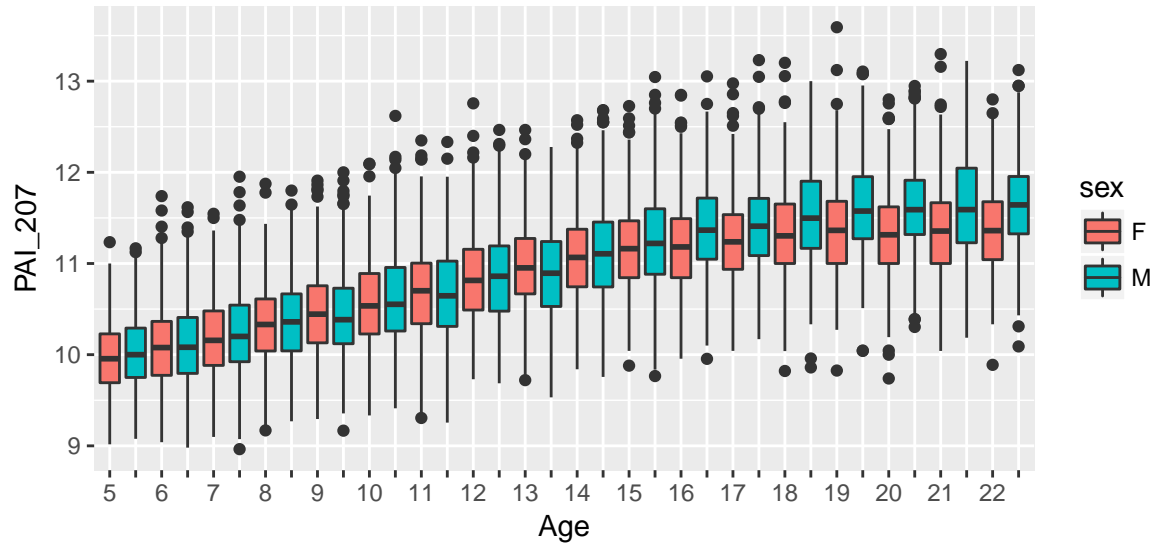

# Distributions of PAI\_20 by Sex and Age

ages from 5 years to 22 years old

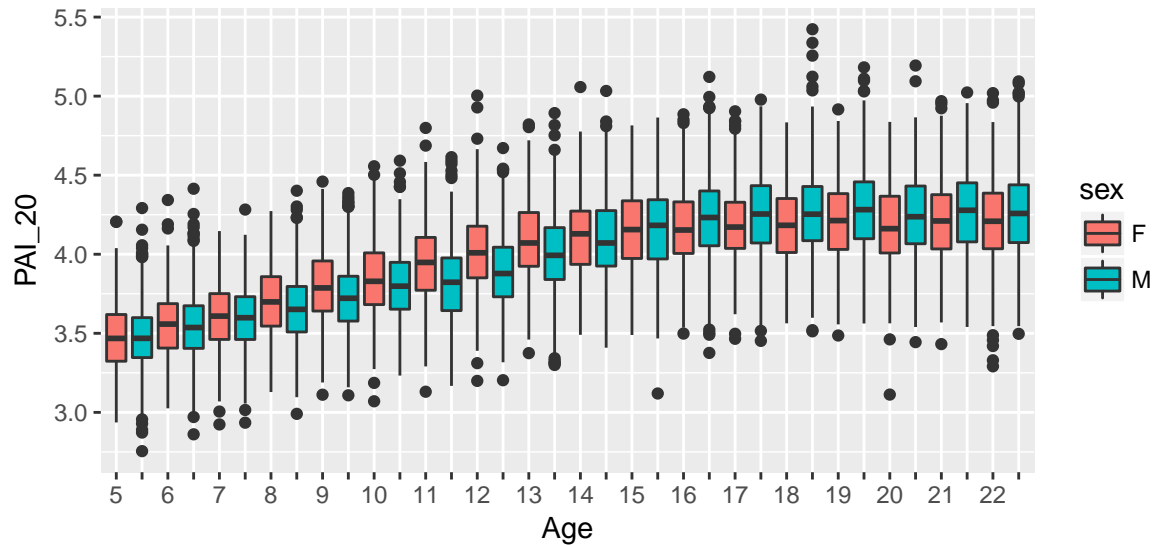

# Distributions of PAI\_21 by Sex and Age

ages from 5 years to 22 years old

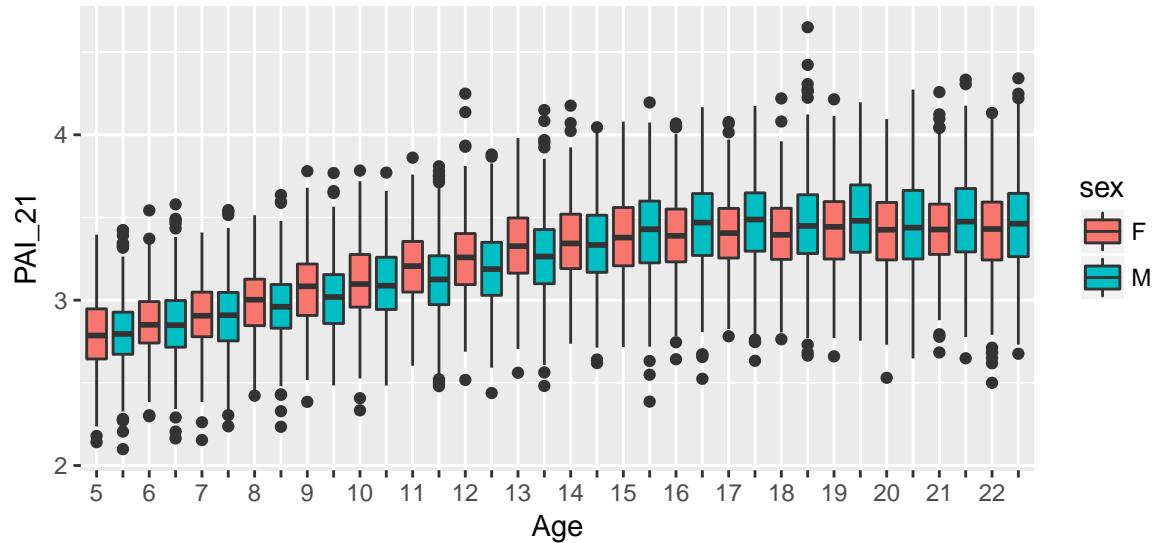

# Distributions of PAI\_22 by Sex and Age

ages from 5 years to 22 years old

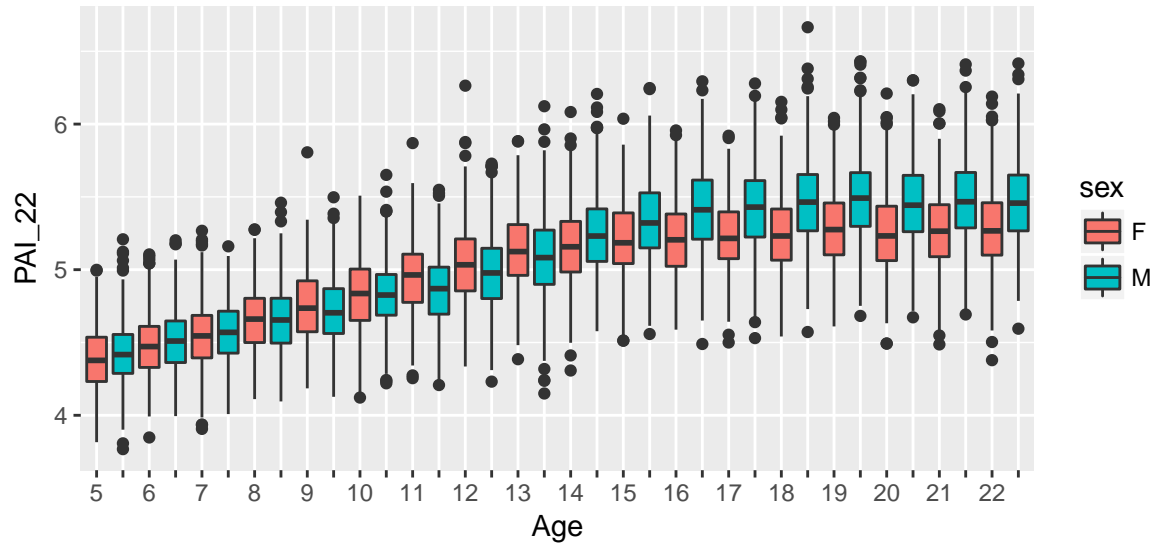

# Distributions of PAI\_23 by Sex and Age

ages from 5 years to 22 years old

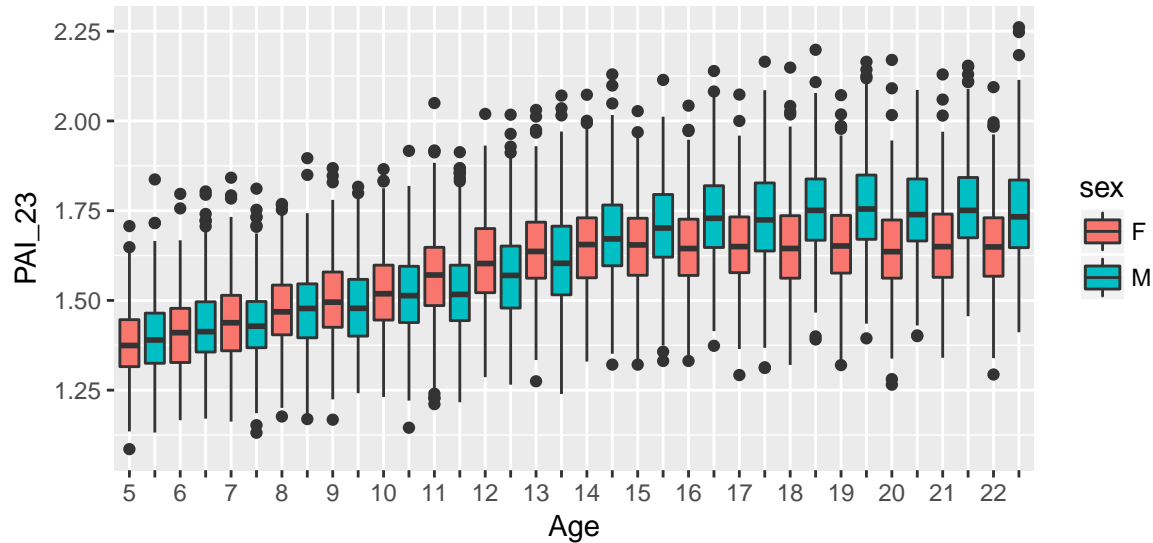

# Distributions of PAI\_24 by Sex and Age

ages from 5 years to 22 years old

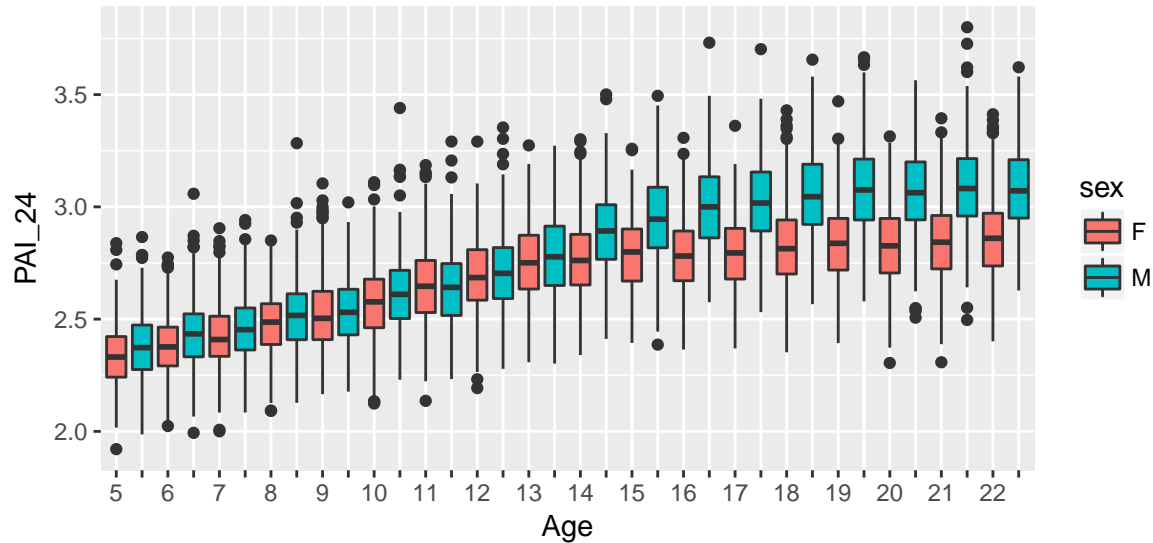

# Distributions of PAI\_25 by Sex and Age

ages from 5 years to 22 years old

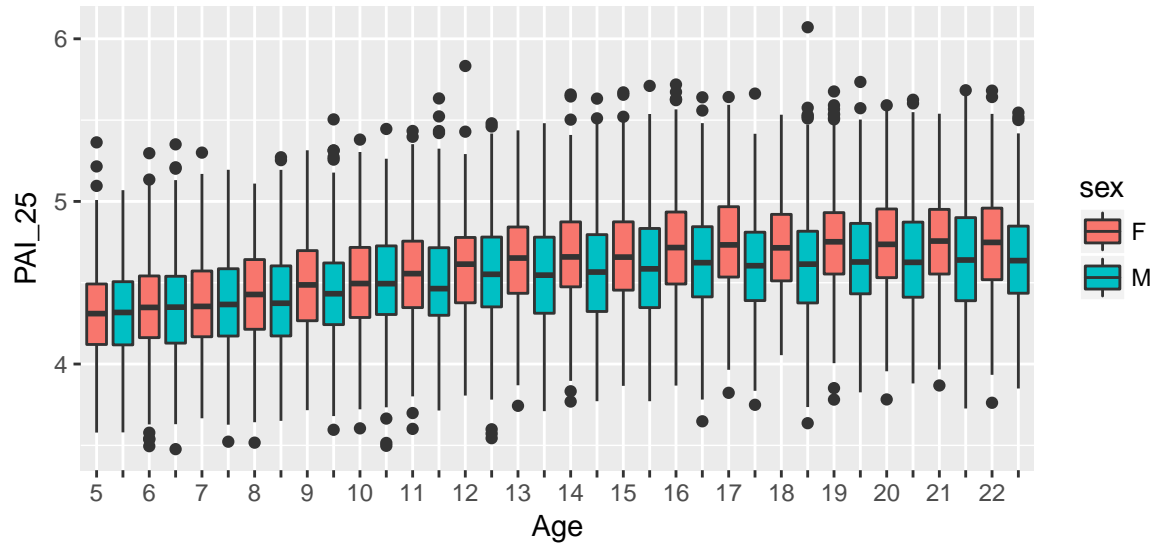

# Distributions of PAI\_26 by Sex and Age

ages from 5 years to 22 years old

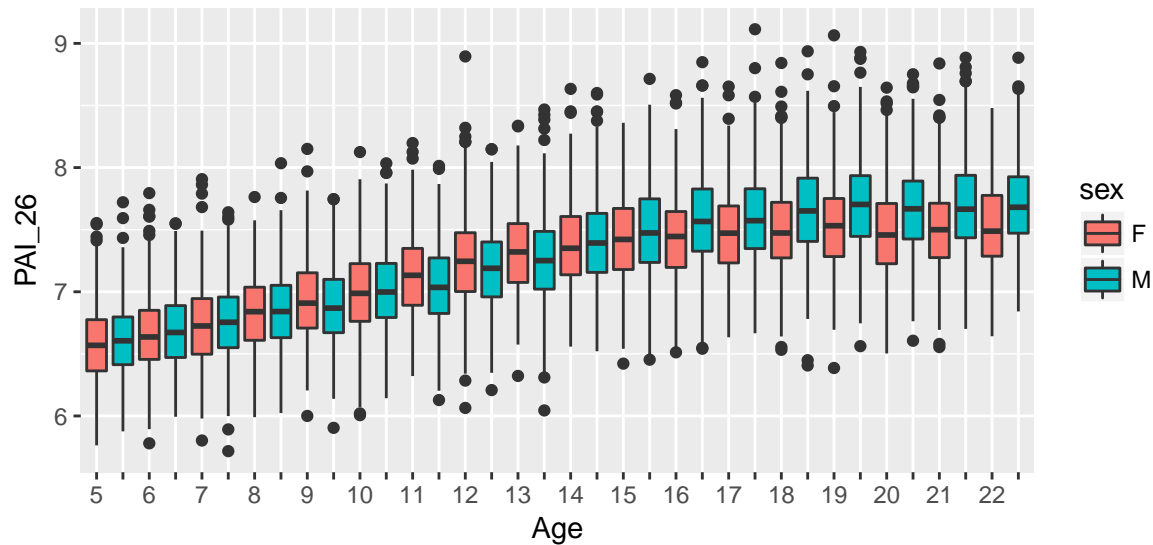

# Distributions of PAI\_27 by Sex and Age

ages from 5 years to 22 years old

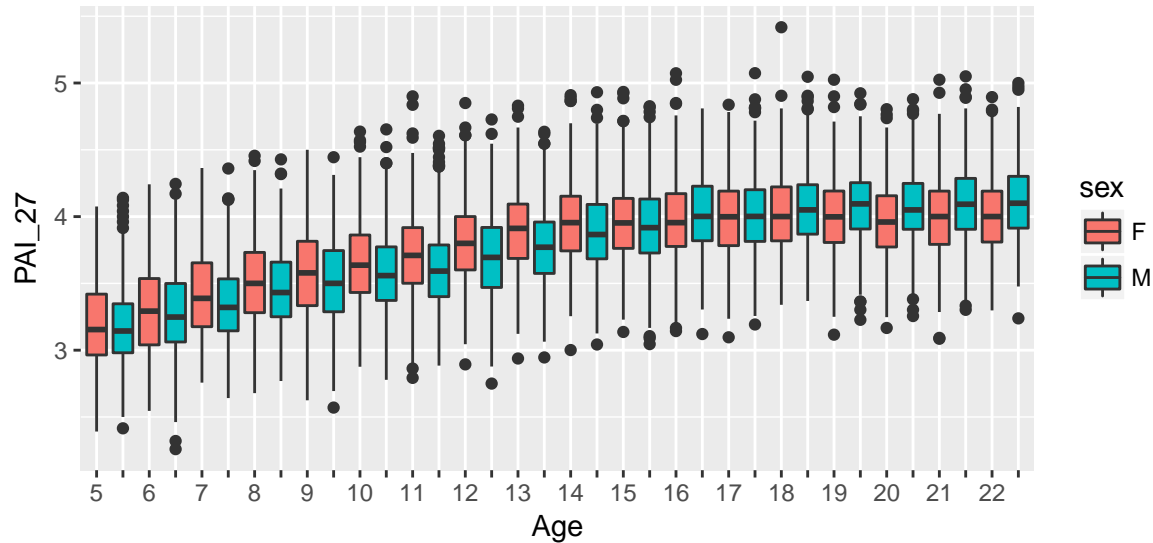

# Distributions of PAI\_28 by Sex and Age

ages from 5 years to 22 years old

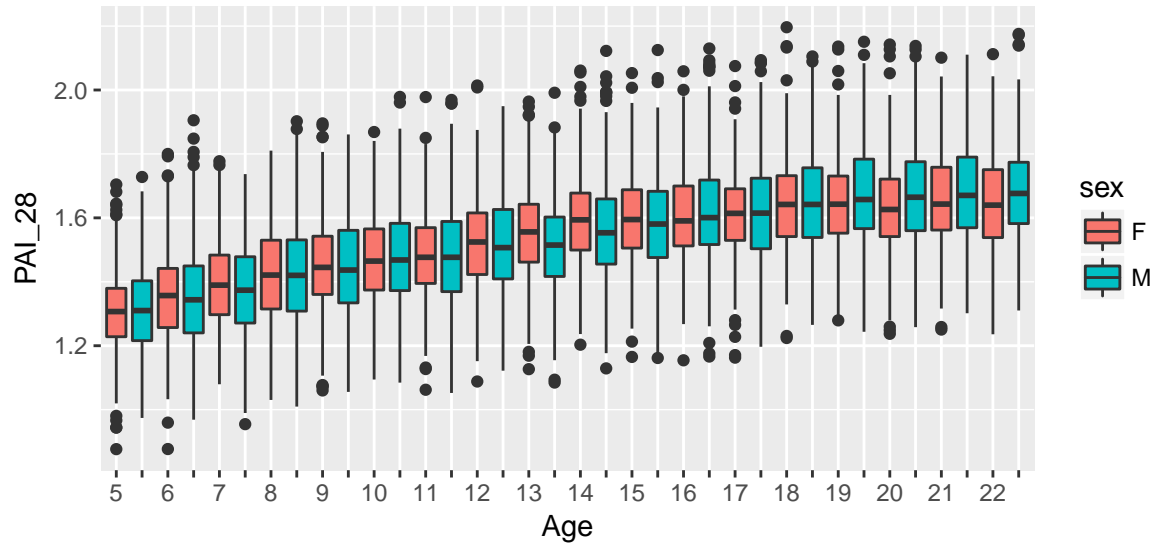

# Distributions of PAI\_29 by Sex and Age

ages from 5 years to 22 years old

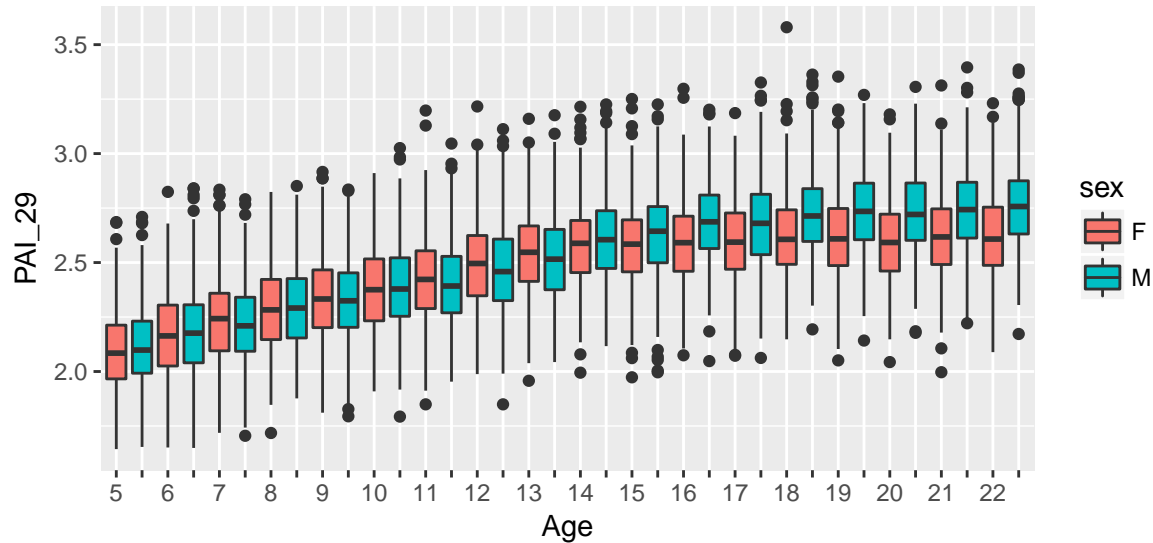

# Distributions of PAI\_2 by Sex and Age

ages from 5 years to 22 years old

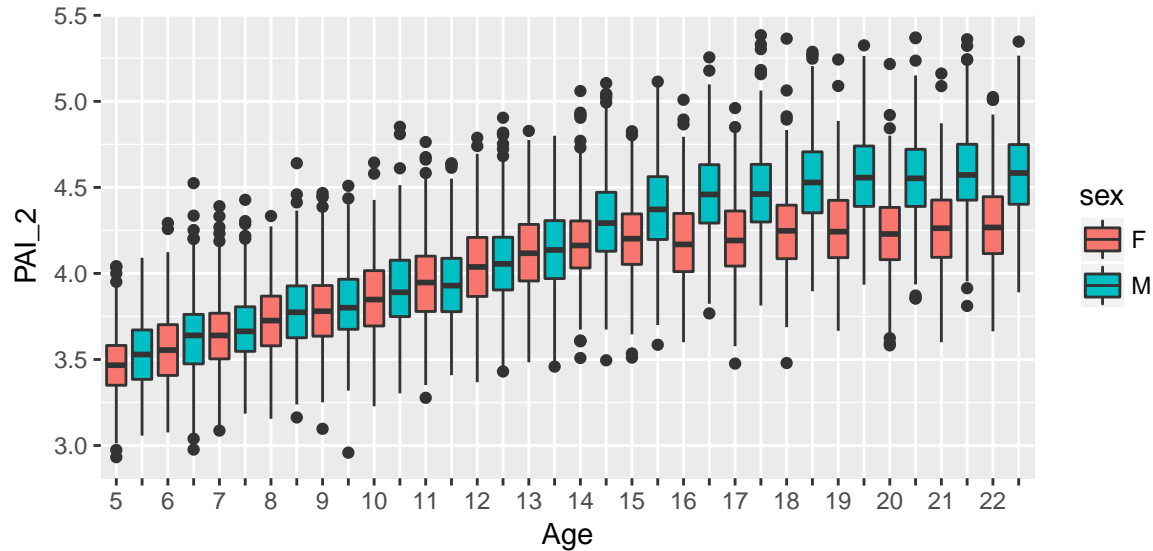

# Distributions of PAI\_30 by Sex and Age

ages from 5 years to 22 years old

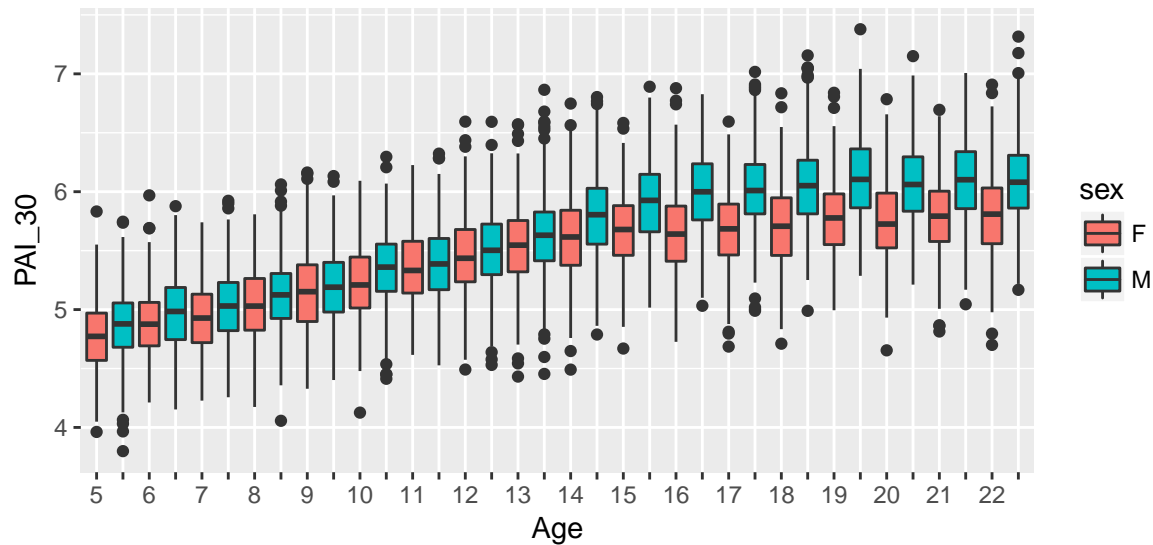

# Distributions of PAI\_31 by Sex and Age

ages from 5 years to 22 years old

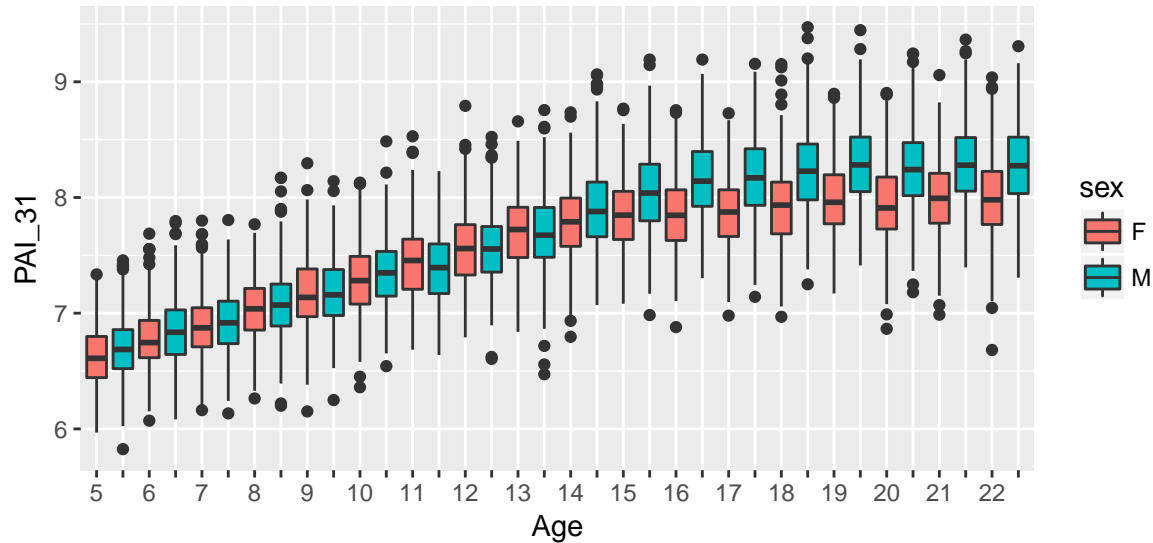

# Distributions of PAI\_32 by Sex and Age

ages from 5 years to 22 years old

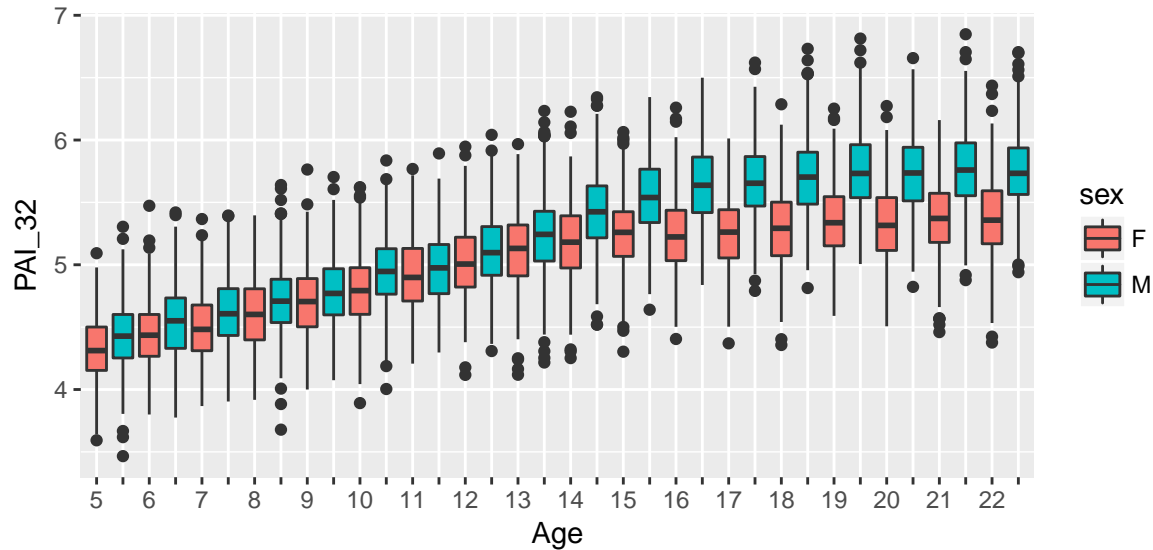

# Distributions of PAI\_33 by Sex and Age

ages from 5 years to 22 years old

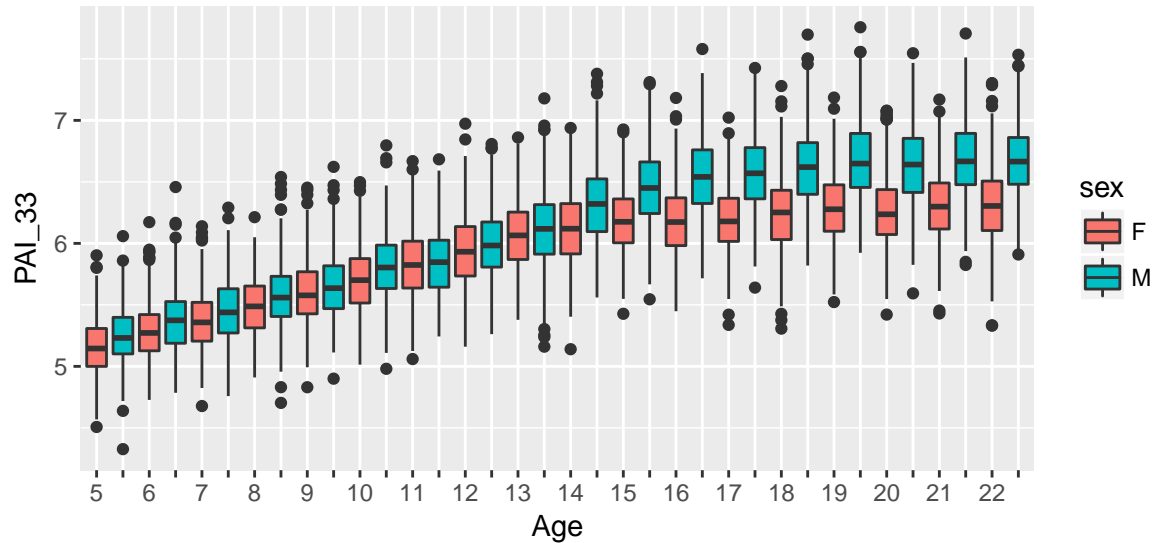

# Distributions of PAI\_34 by Sex and Age

ages from 5 years to 22 years old

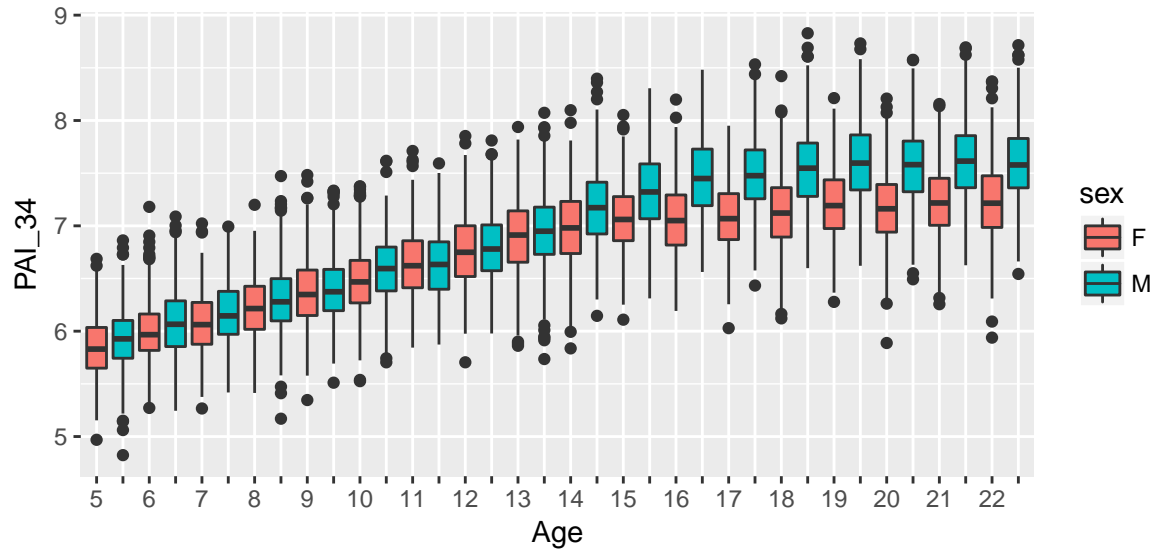

# Distributions of PAI\_35 by Sex and Age

ages from 5 years to 22 years old

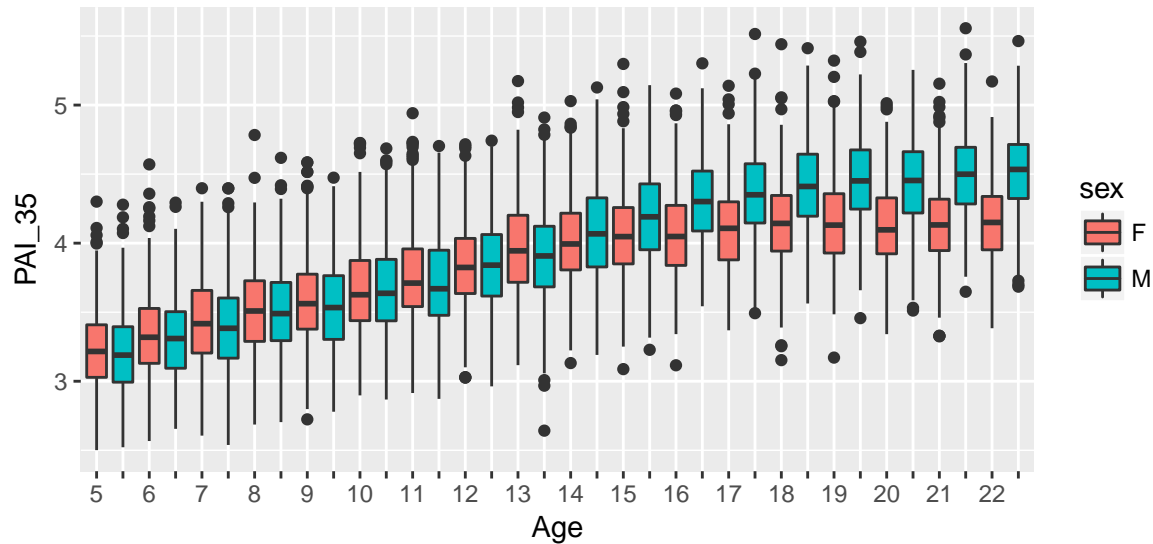

# Distributions of PAI\_36 by Sex and Age

ages from 5 years to 22 years old

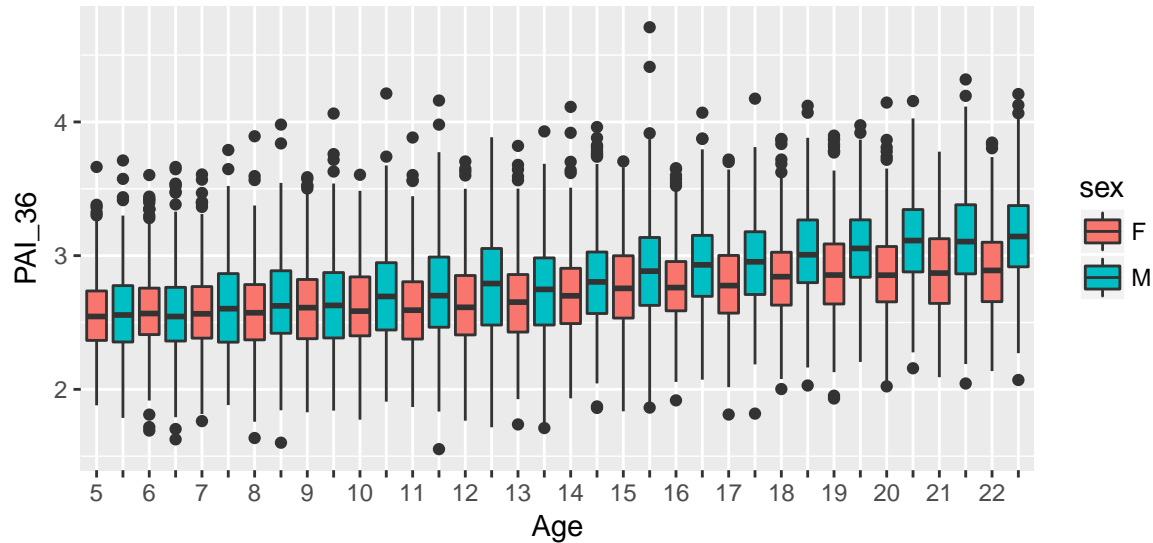

# Distributions of PAI\_37 by Sex and Age

ages from 5 years to 22 years old

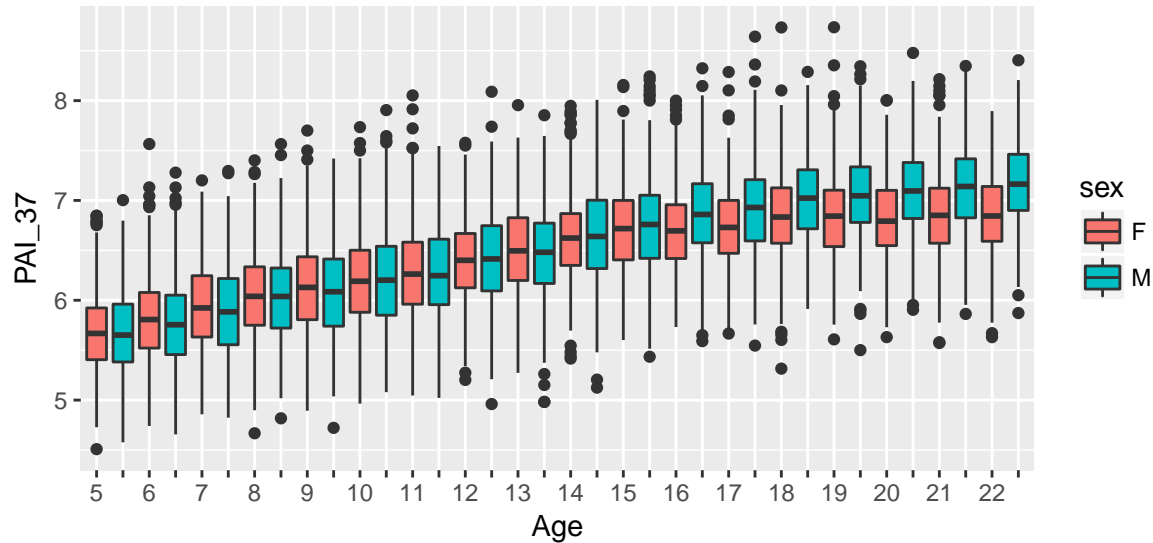

# Distributions of PAI\_38 by Sex and Age

ages from 5 years to 22 years old

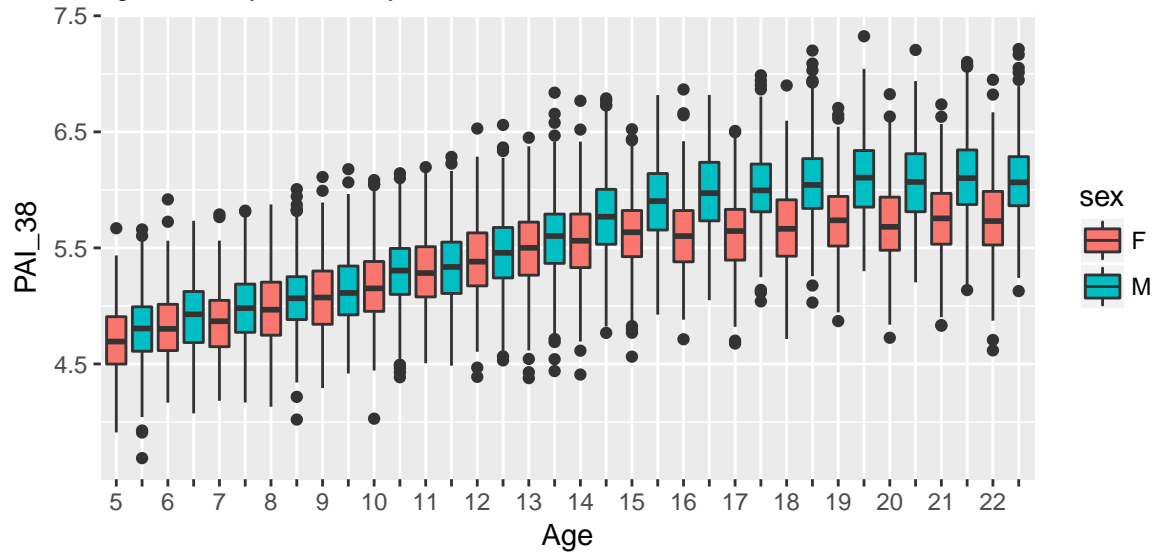

ages from 5 years to 22 years old

ages from 5 years to 22 years old

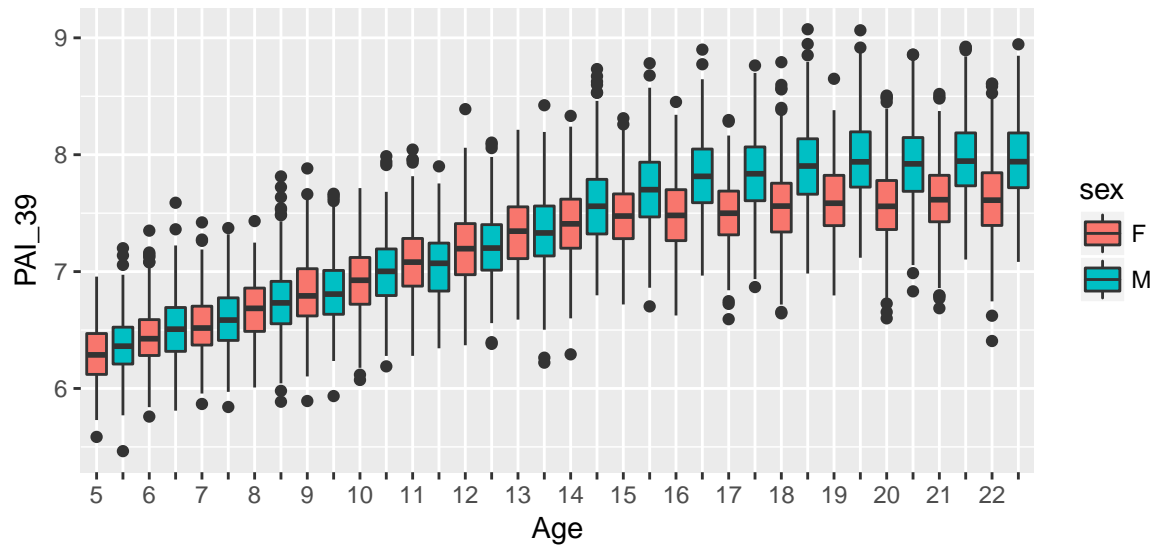

# Distributions of PAI\_3 by Sex and Age

ages from 5 years to 22 years old

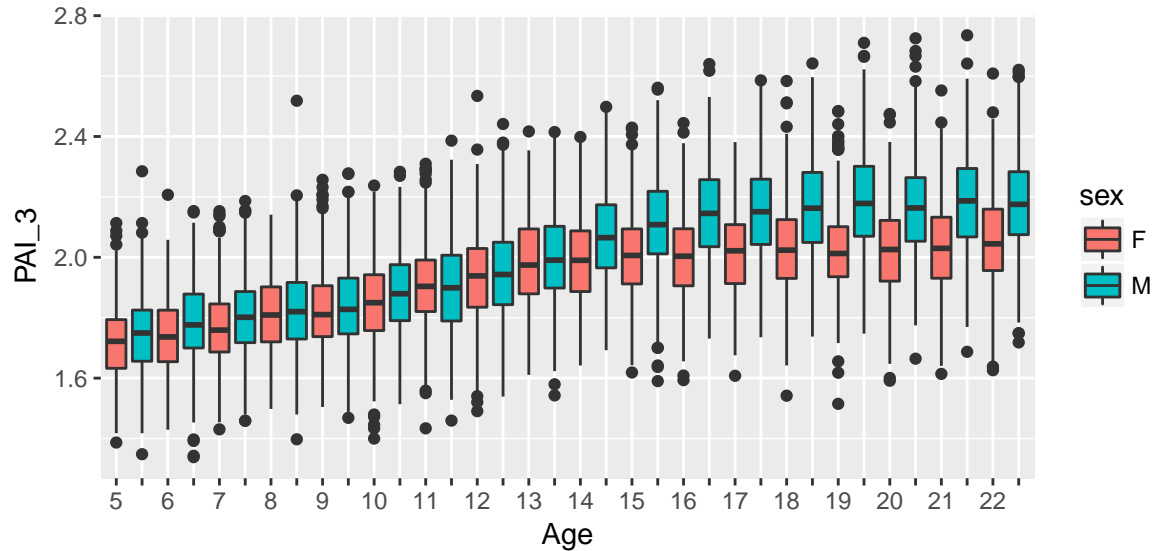

# Distributions of PAI\_40 by Sex and Age

ages from 5 years to 22 years old

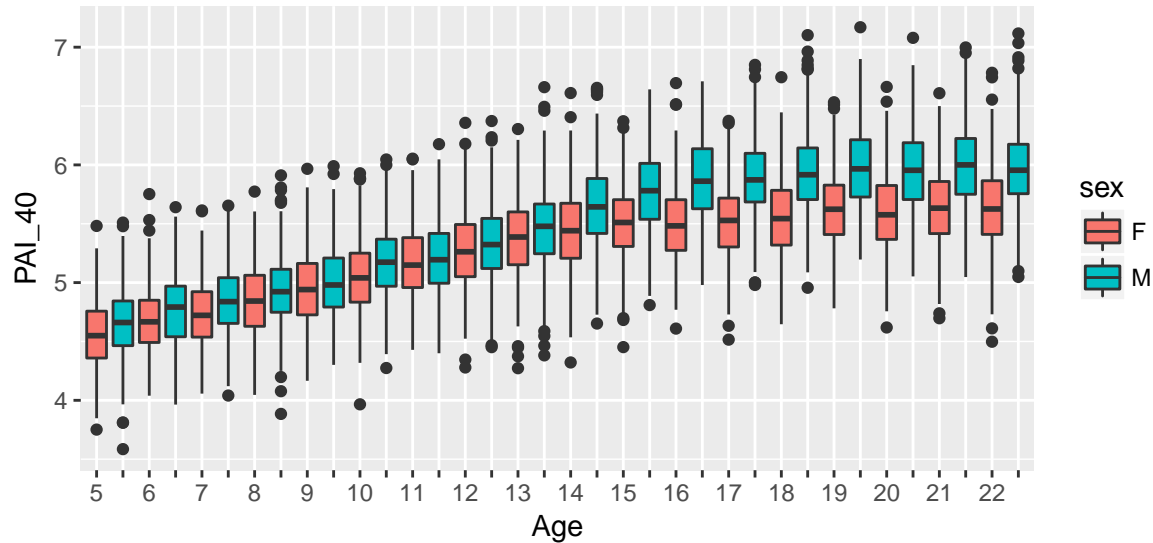

# Distributions of PAI\_41 by Sex and Age

ages from 5 years to 22 years old

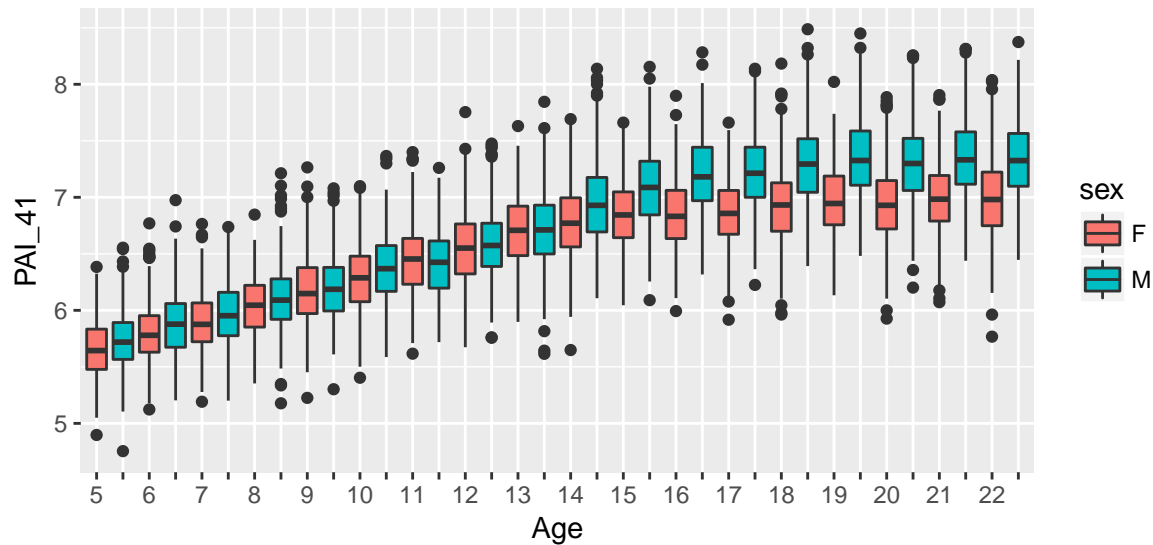

# Distributions of PAI\_42 by Sex and Age

ages from 5 years to 22 years old

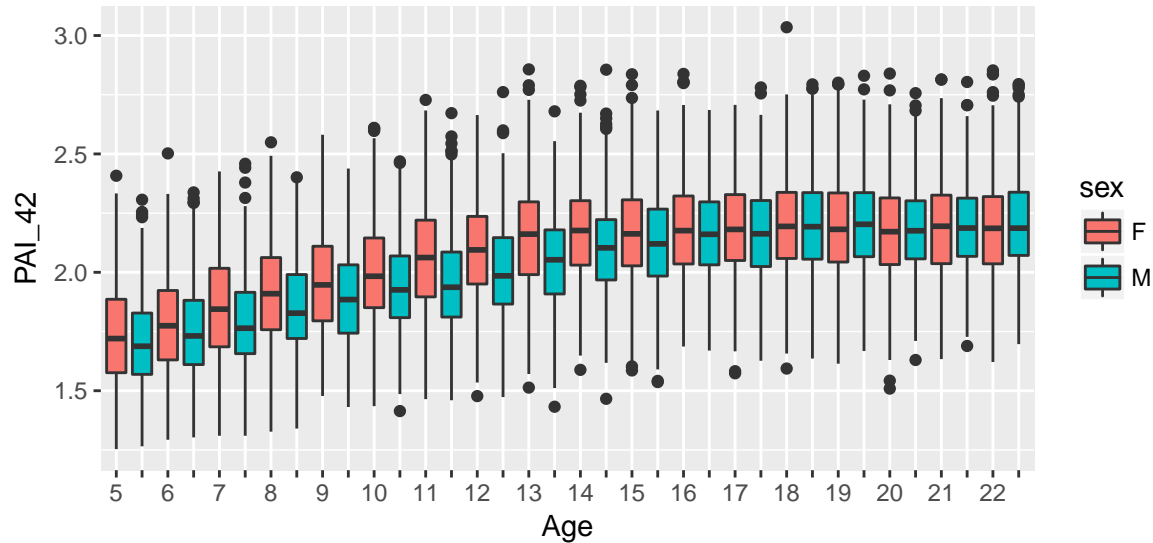

# Distributions of PAI\_43 by Sex and Age

ages from 5 years to 22 years old

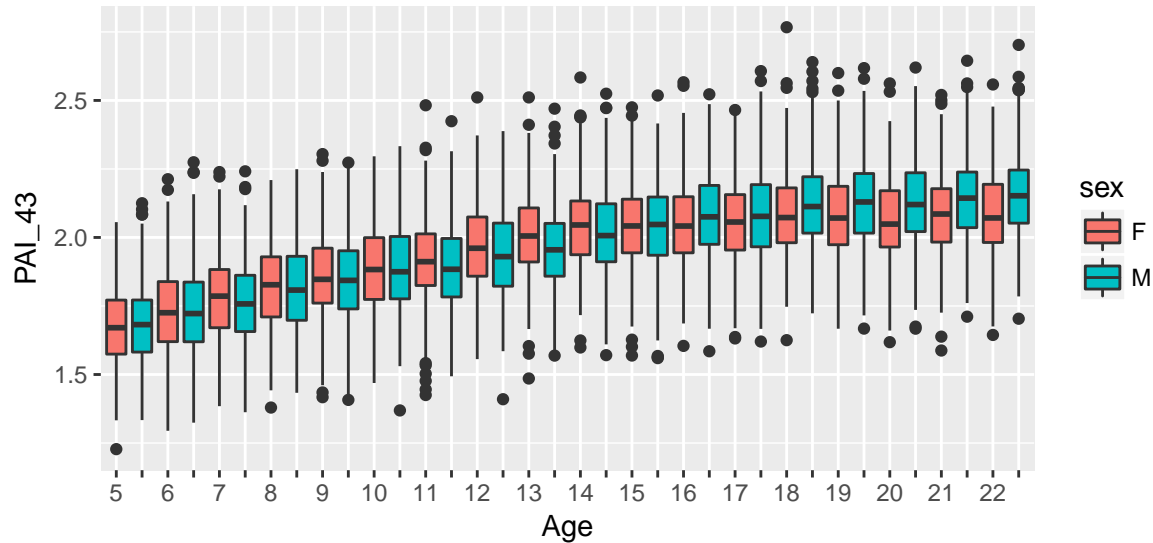

# Distributions of PAI\_44 by Sex and Age

ages from 5 years to 22 years old

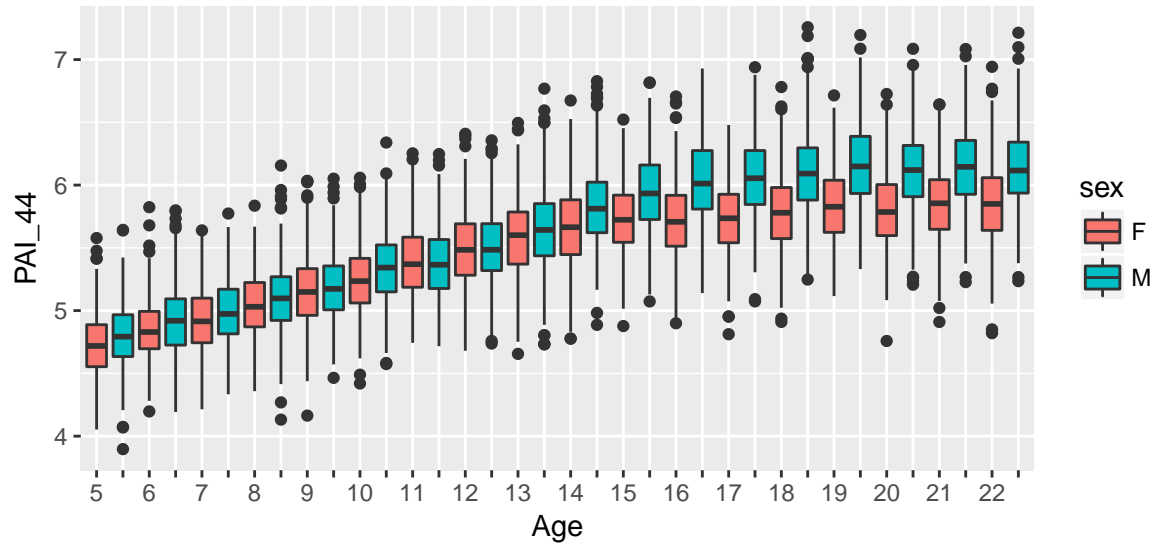

# Distributions of PAI\_45 by Sex and Age

ages from 5 years to 22 years old

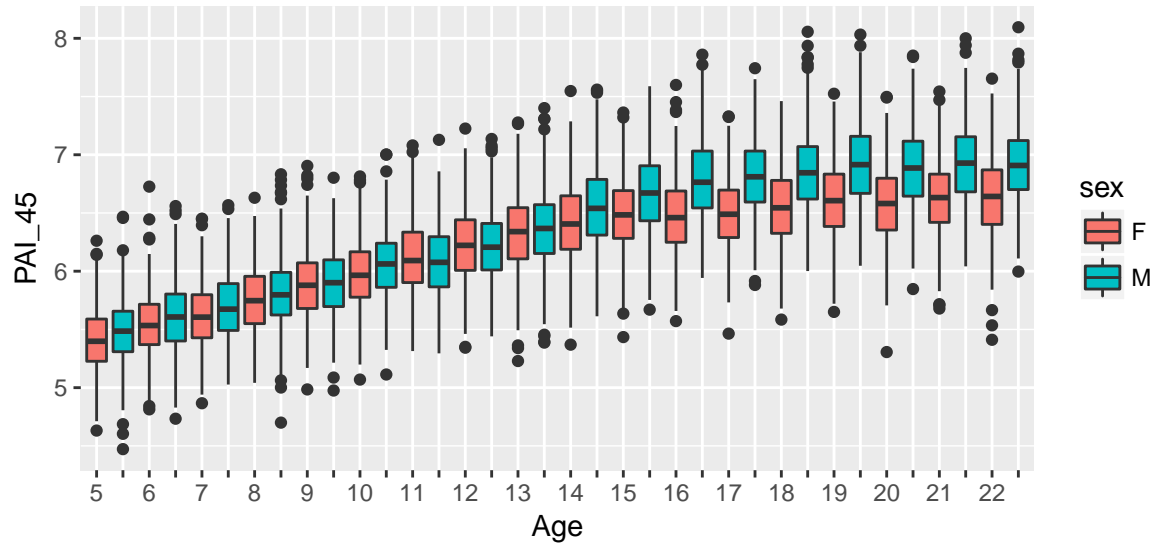

# Distributions of PAI\_46 by Sex and Age

ages from 5 years to 22 years old

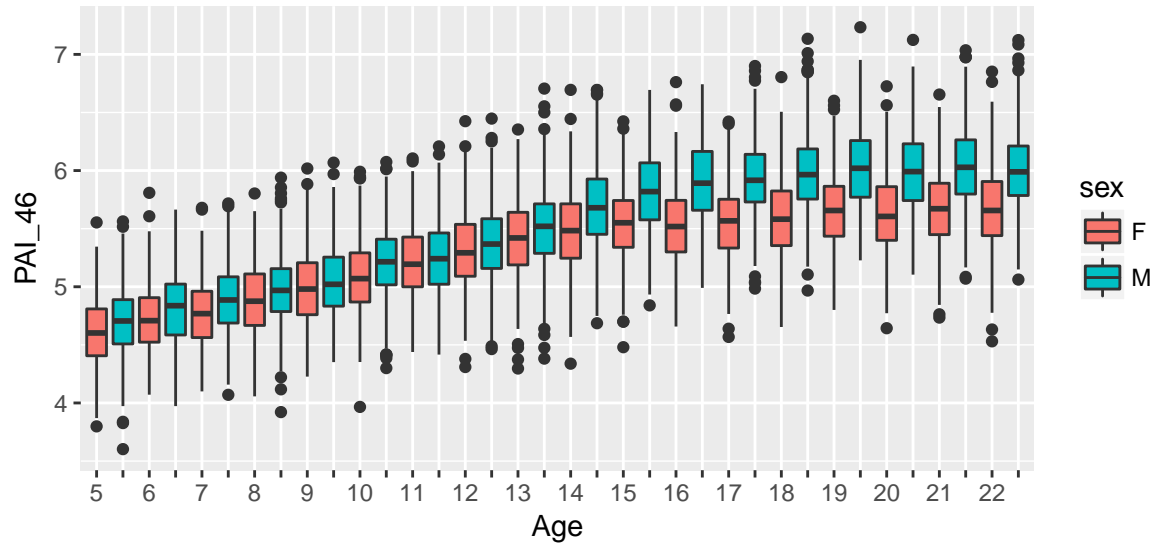

# Distributions of PAI\_47 by Sex and Age

ages from 5 years to 22 years old

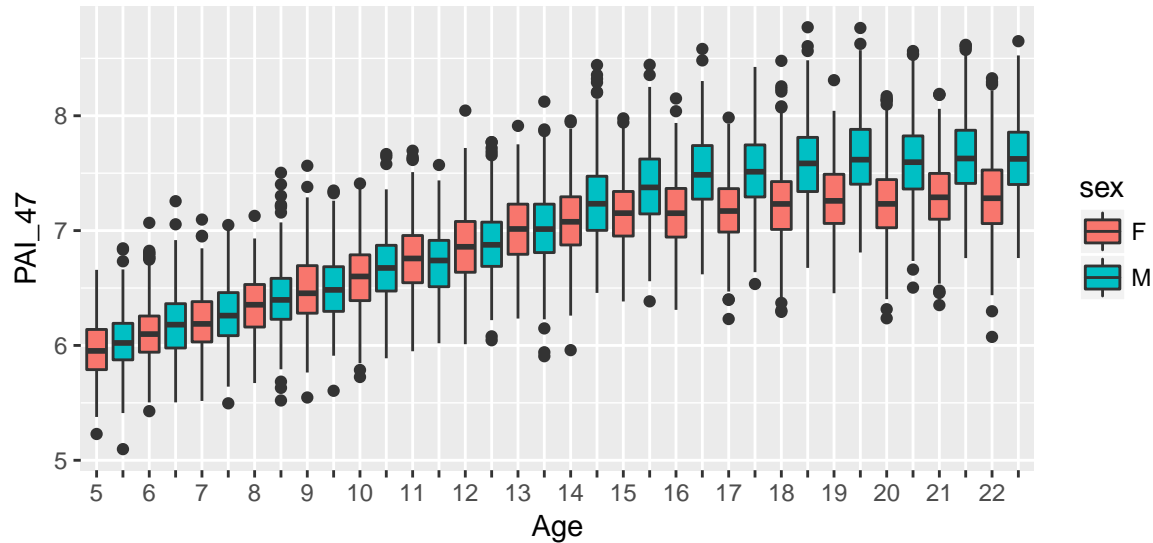

# Distributions of PAI\_48 by Sex and Age

ages from 5 years to 22 years old

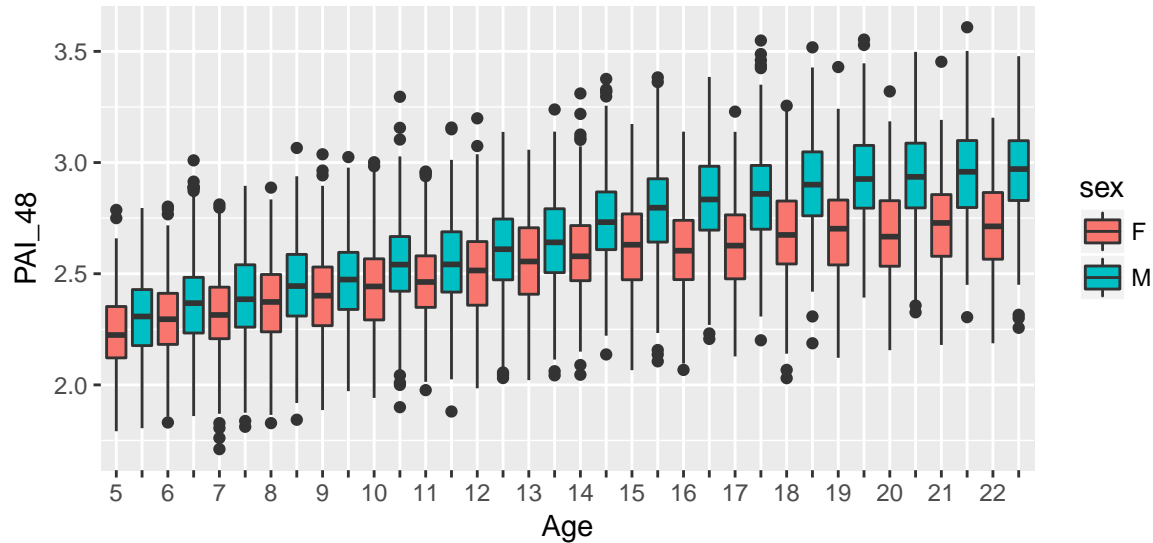

## Distributions of PAI\_49 by Sex and Age

ages from 5 years to 22 years old

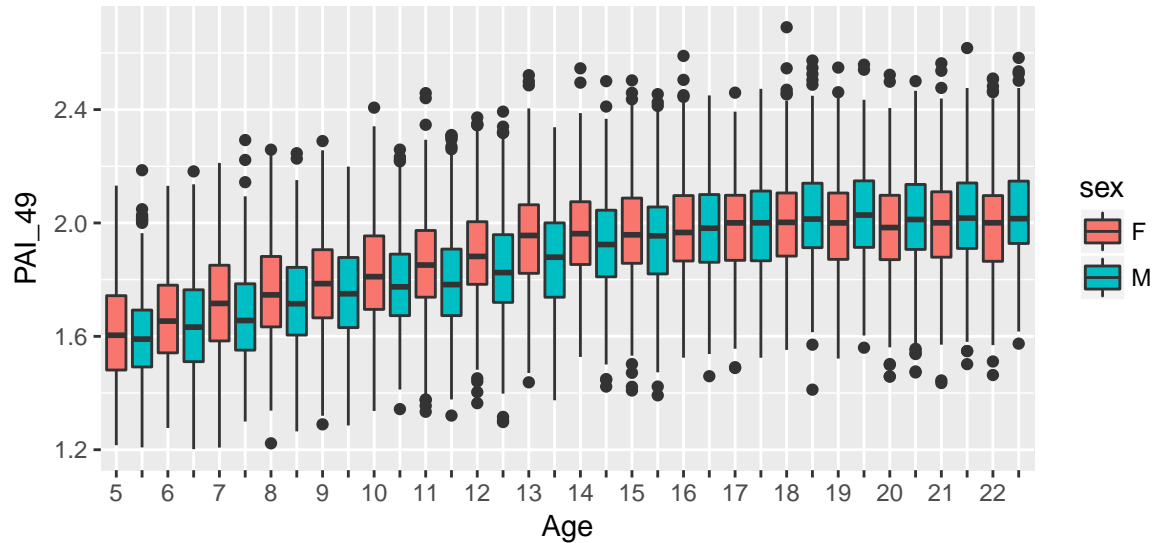

# Distributions of PAI\_4 by Sex and Age

ages from 5 years to 22 years old

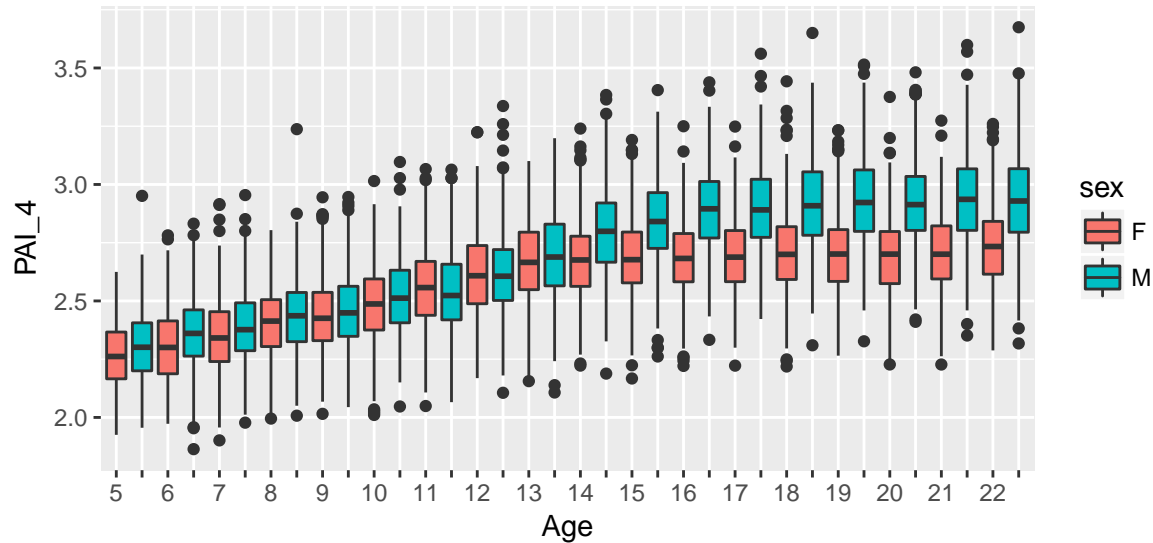

# Distributions of PAI\_50 by Sex and Age

ages from 5 years to 22 years old

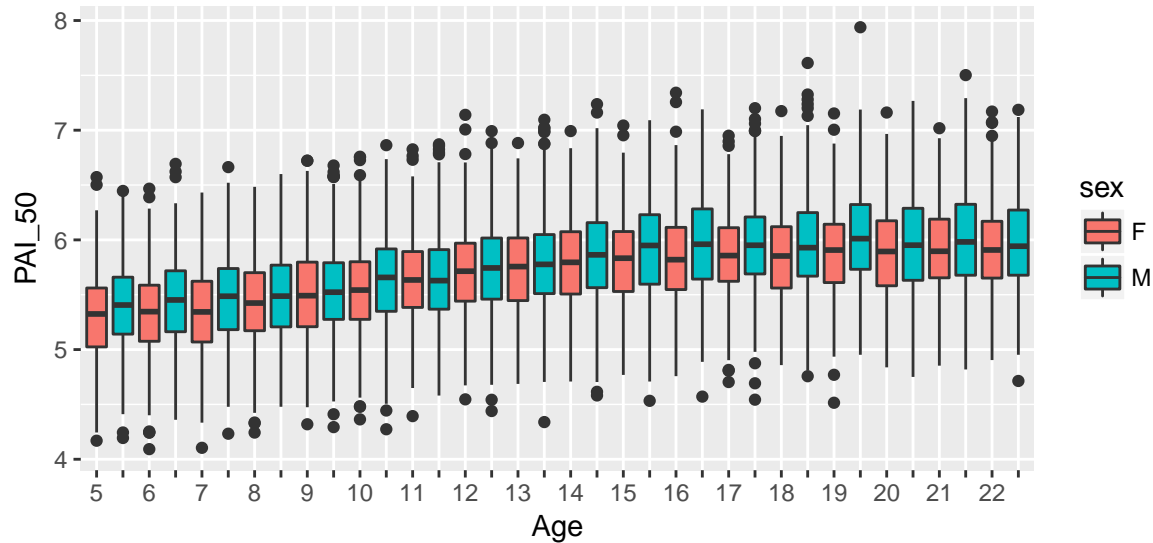

# Distributions of PAI\_51 by Sex and Age

ages from 5 years to 22 years old

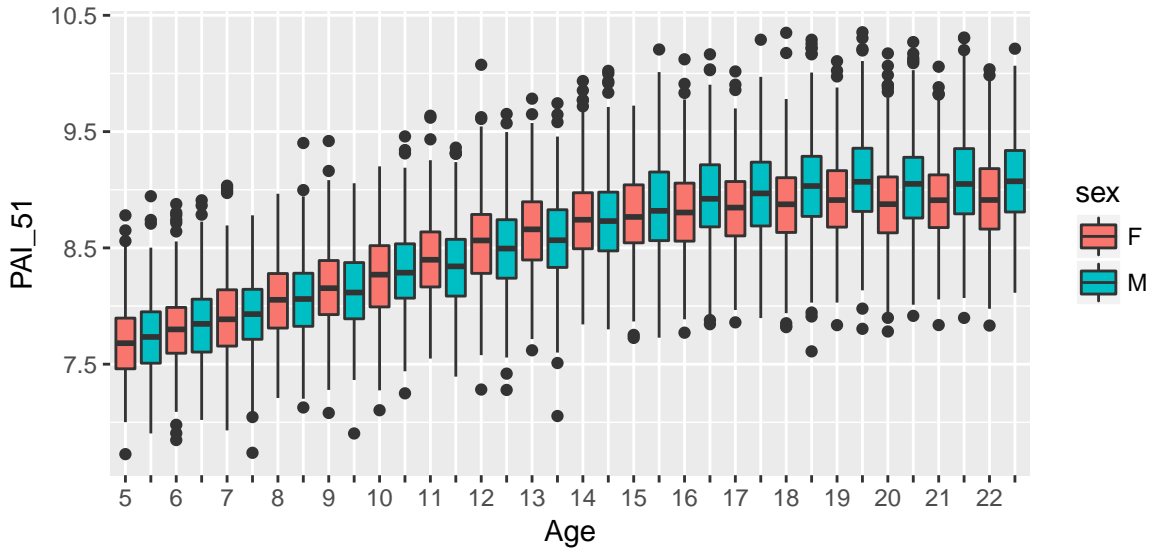

# Distributions of PAI\_52 by Sex and Age

ages from 5 years to 22 years old

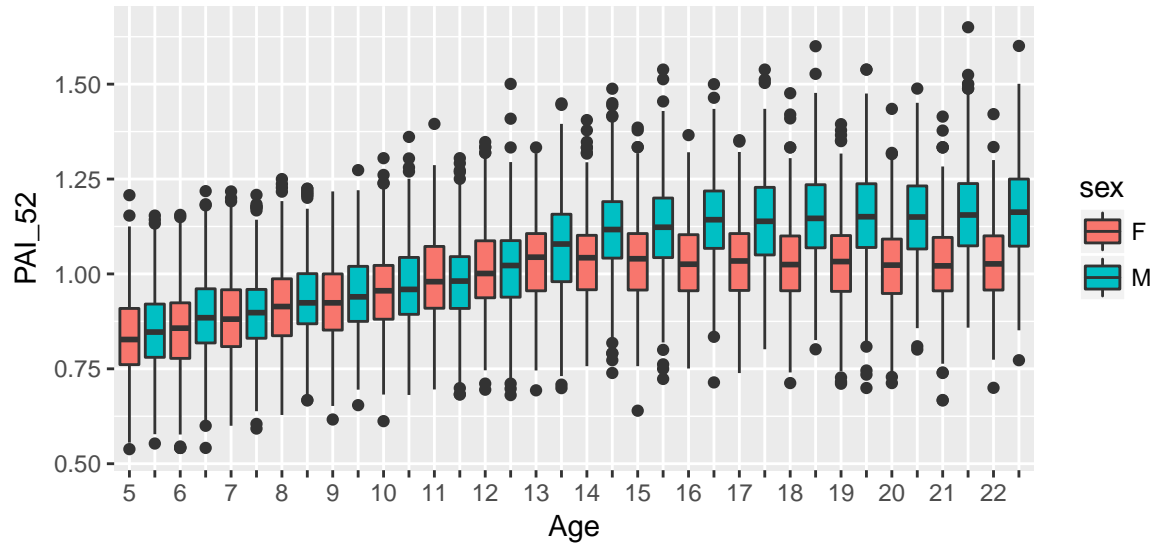

# Distributions of PAI\_53 by Sex and Age

ages from 5 years to 22 years old

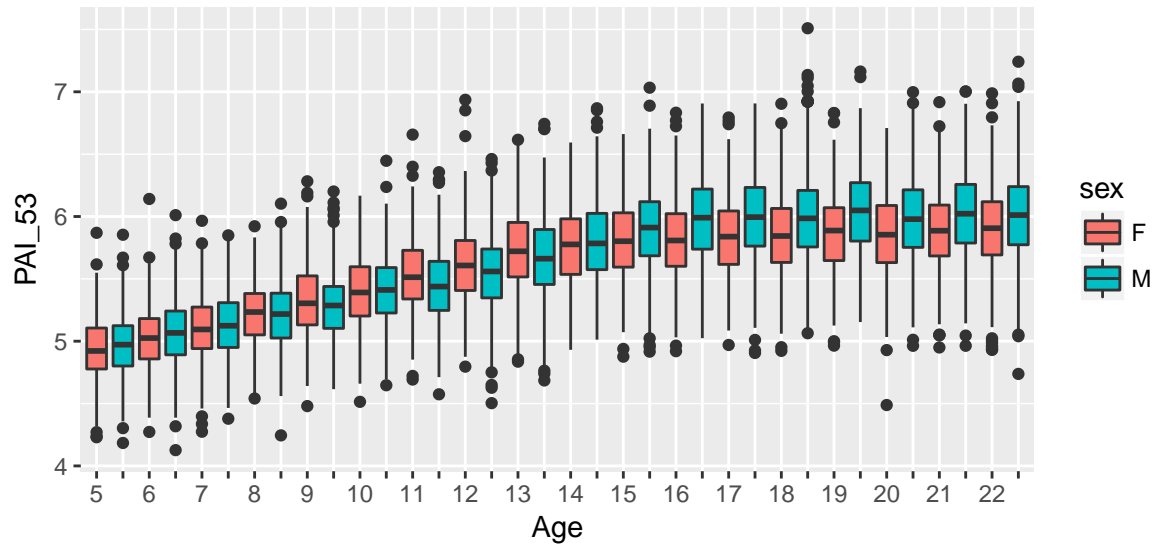

# Distributions of PAI\_54 by Sex and Age

ages from 5 years to 22 years old

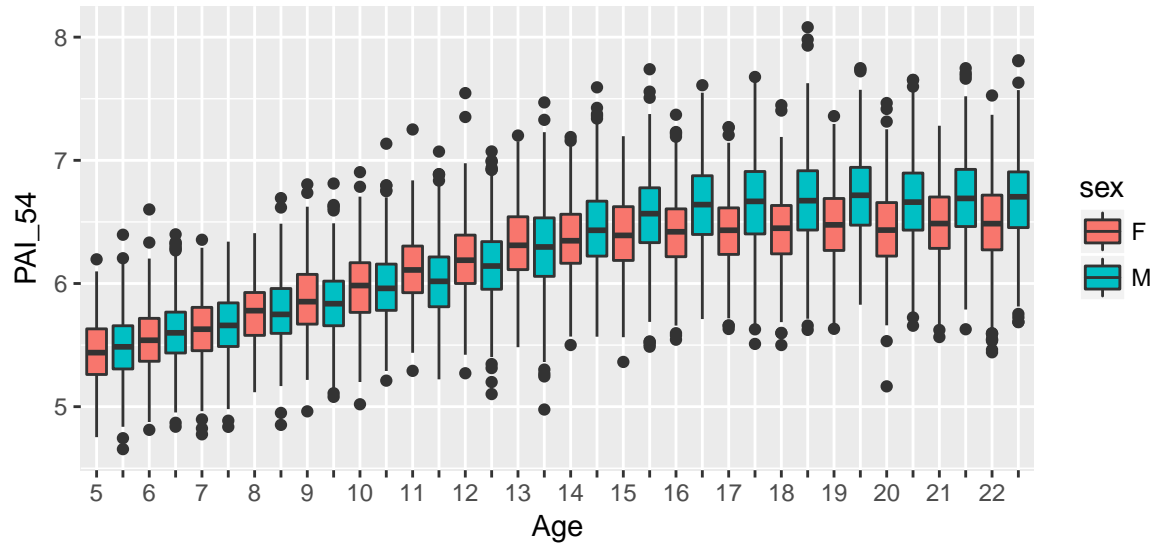

# Distributions of PAI\_55 by Sex and Age

ages from 5 years to 22 years old

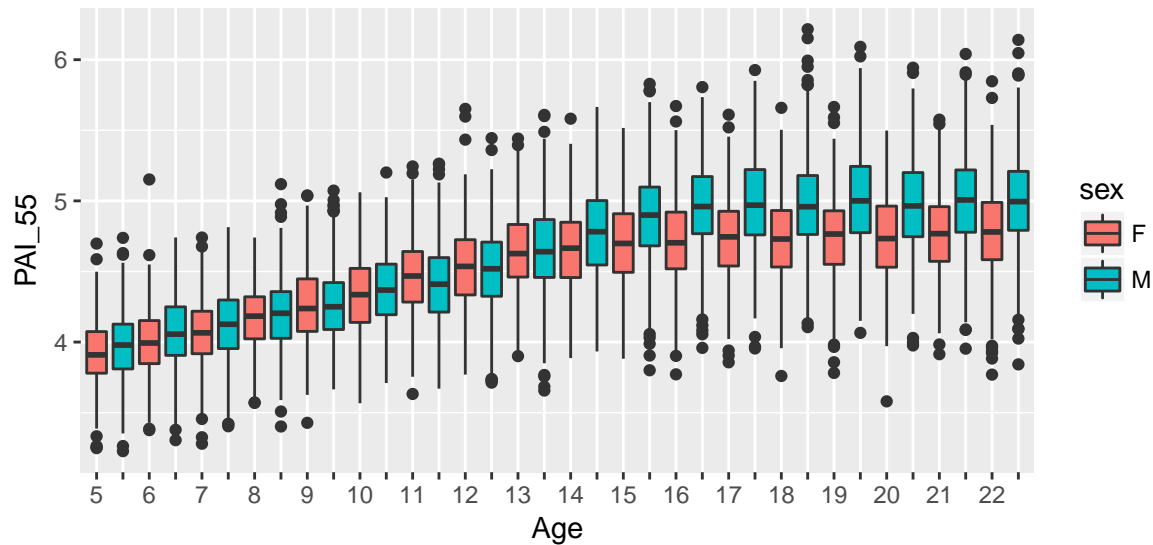

# Distributions of PAI\_56 by Sex and Age

ages from 5 years to 22 years old

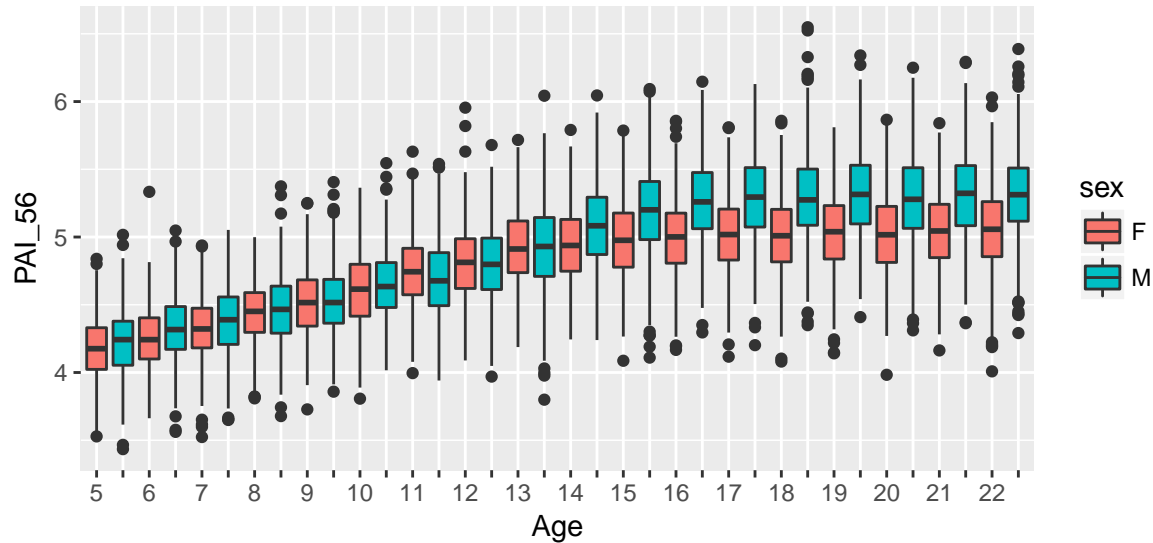

# Distributions of PAI\_57 by Sex and Age

ages from 5 years to 22 years old

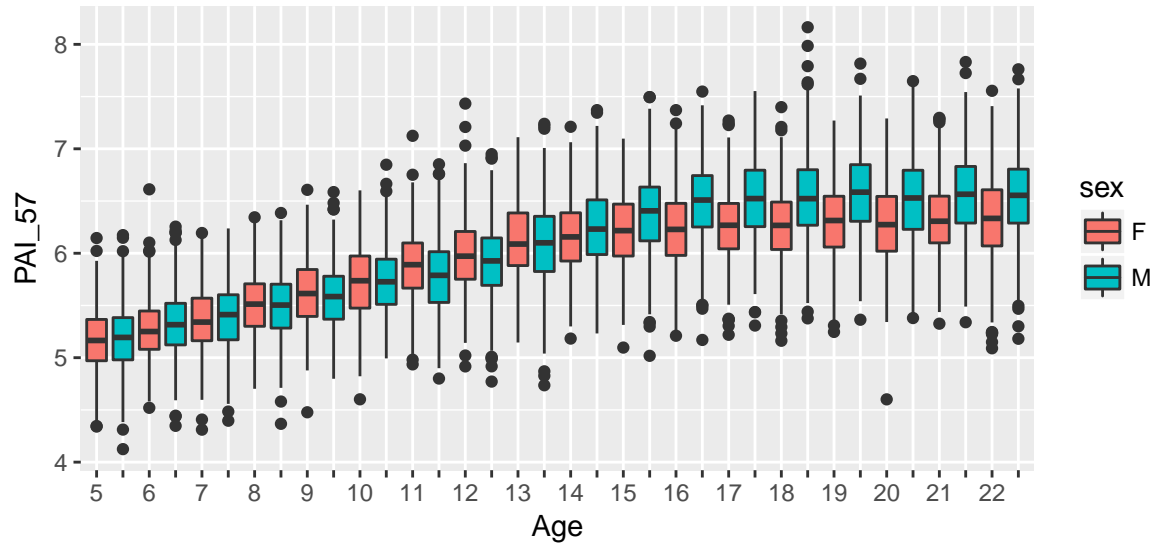

# Distributions of PAI\_58 by Sex and Age

ages from 5 years to 22 years old

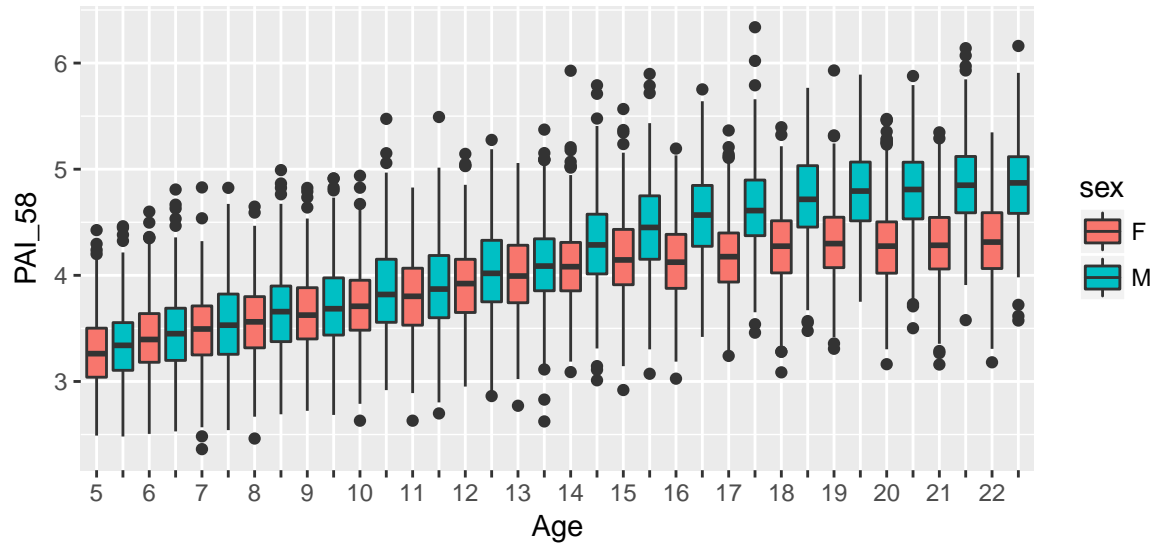

# Distributions of PAI\_59 by Sex and Age

ages from 5 years to 22 years old

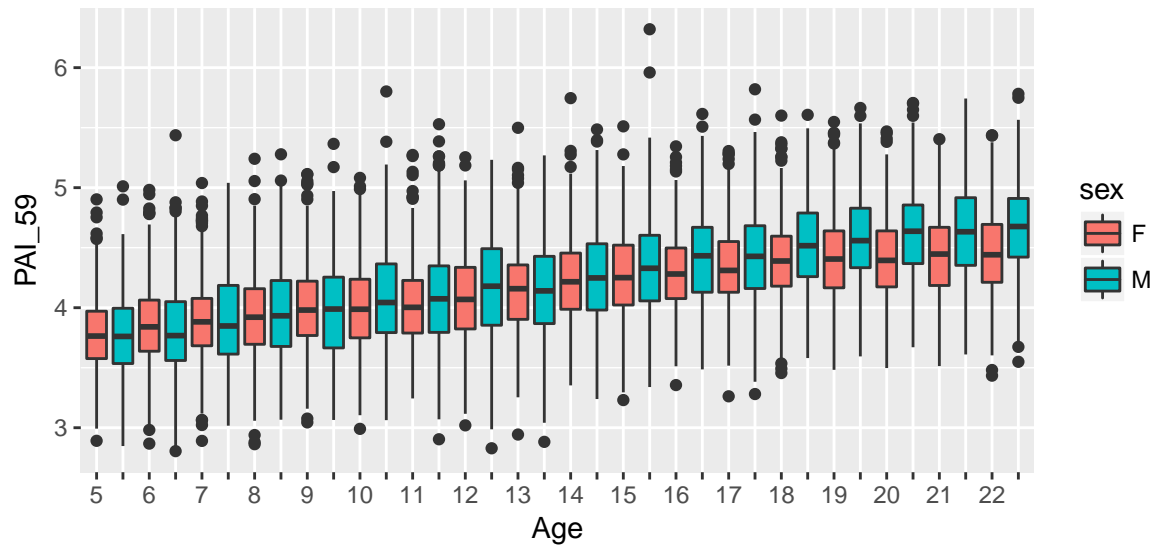

# Distributions of PAI\_5 by Sex and Age

ages from 5 years to 22 years old

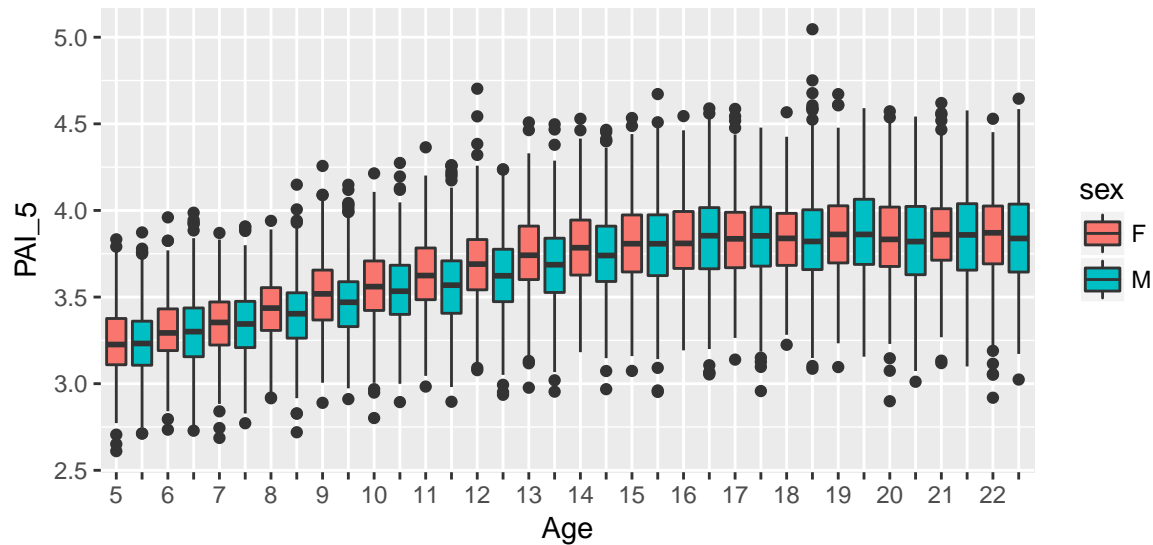

# Distributions of PAI\_60 by Sex and Age

ages from 5 years to 22 years old

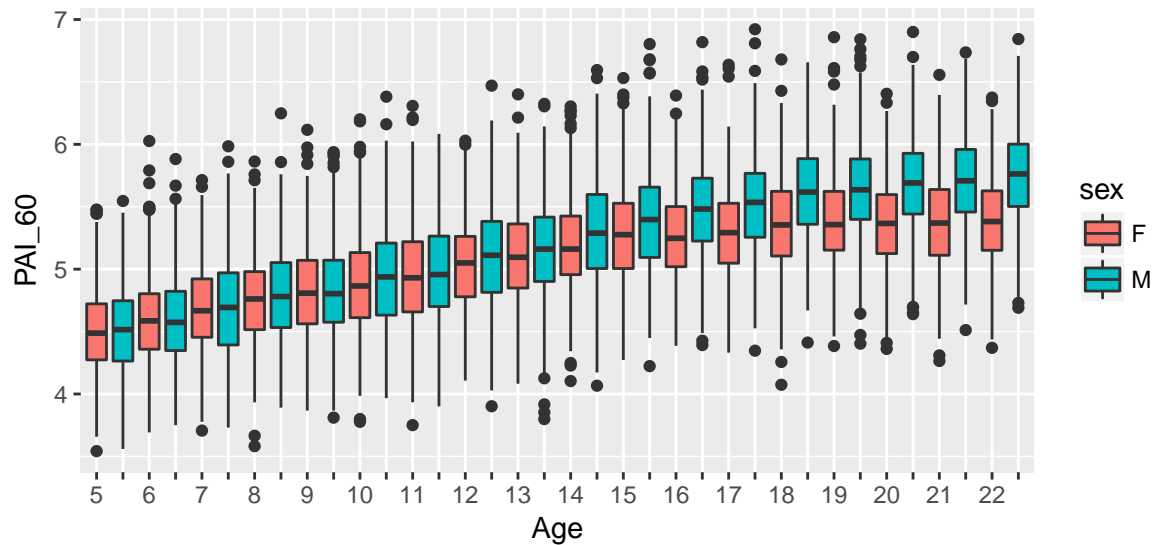

# Distributions of PAI\_61 by Sex and Age

ages from 5 years to 22 years old

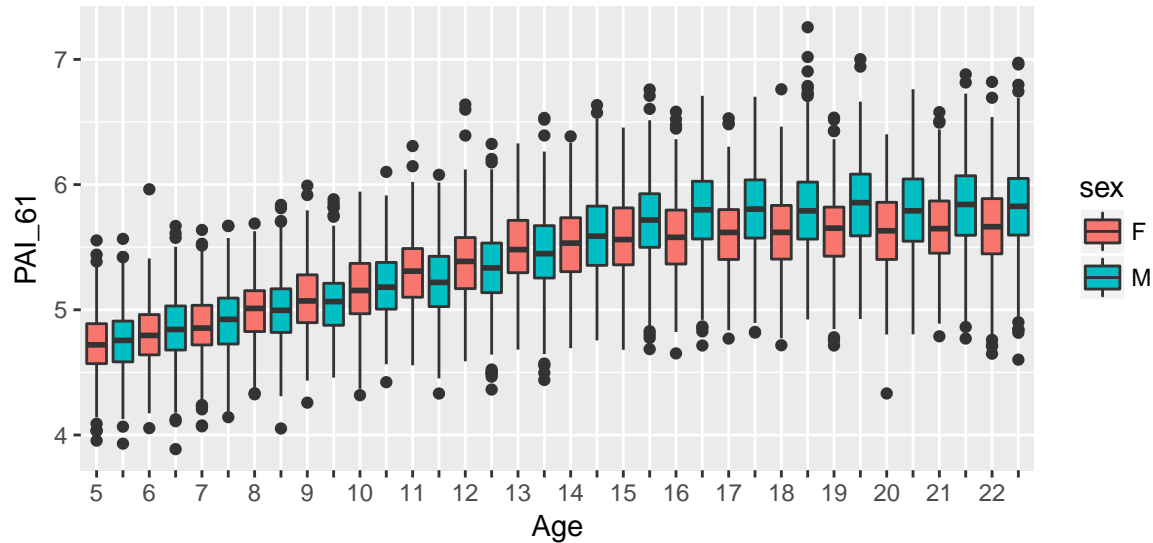

# Distributions of PAI\_62 by Sex and Age

ages from 5 years to 22 years old

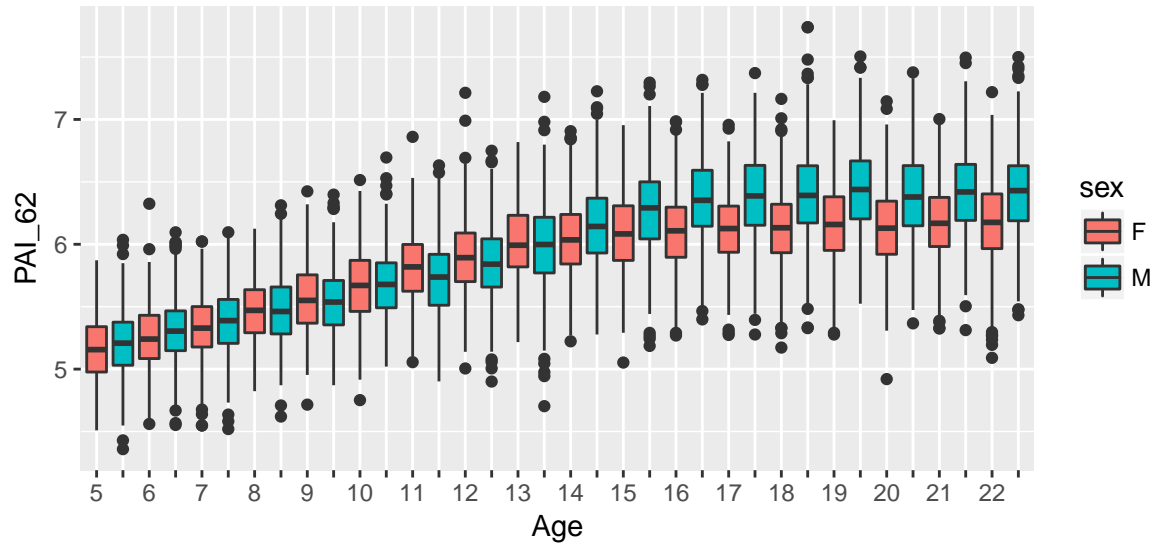

# Distributions of PAI\_63 by Sex and Age

ages from 5 years to 22 years old

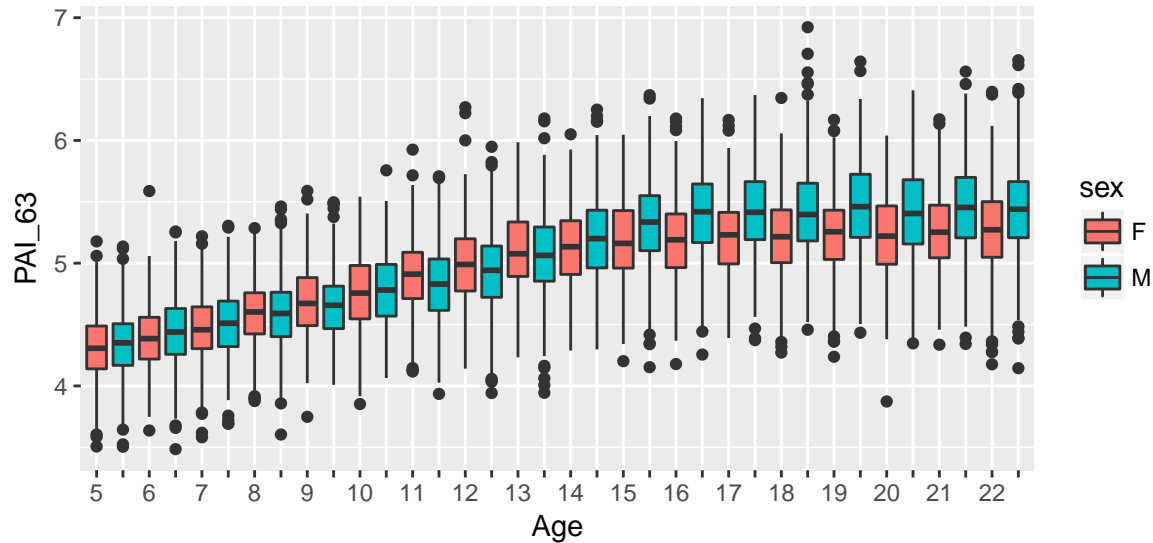

# Distributions of PAI\_64 by Sex and Age

ages from 5 years to 22 years old

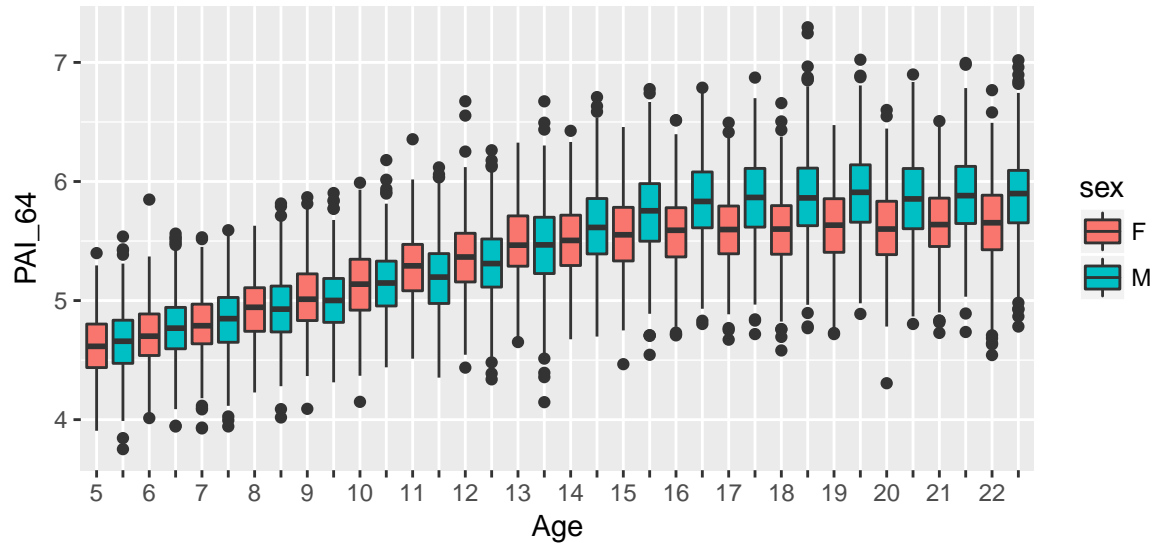

# Distributions of PAI\_65 by Sex and Age

ages from 5 years to 22 years old

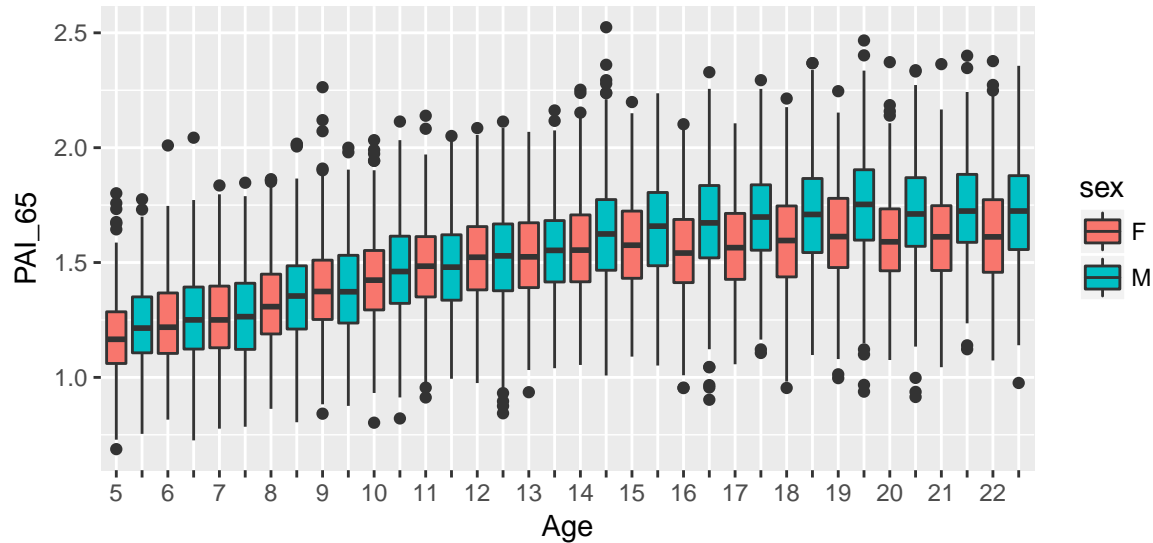

# Distributions of PAI\_66 by Sex and Age

ages from 5 years to 22 years old

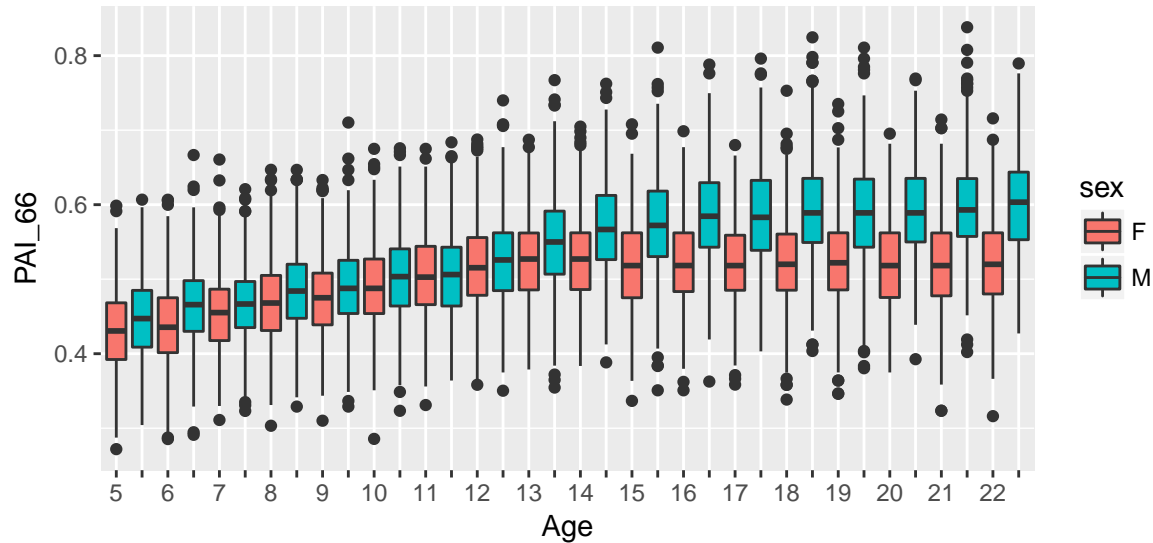

# Distributions of PAI\_67 by Sex and Age

ages from 5 years to 22 years old

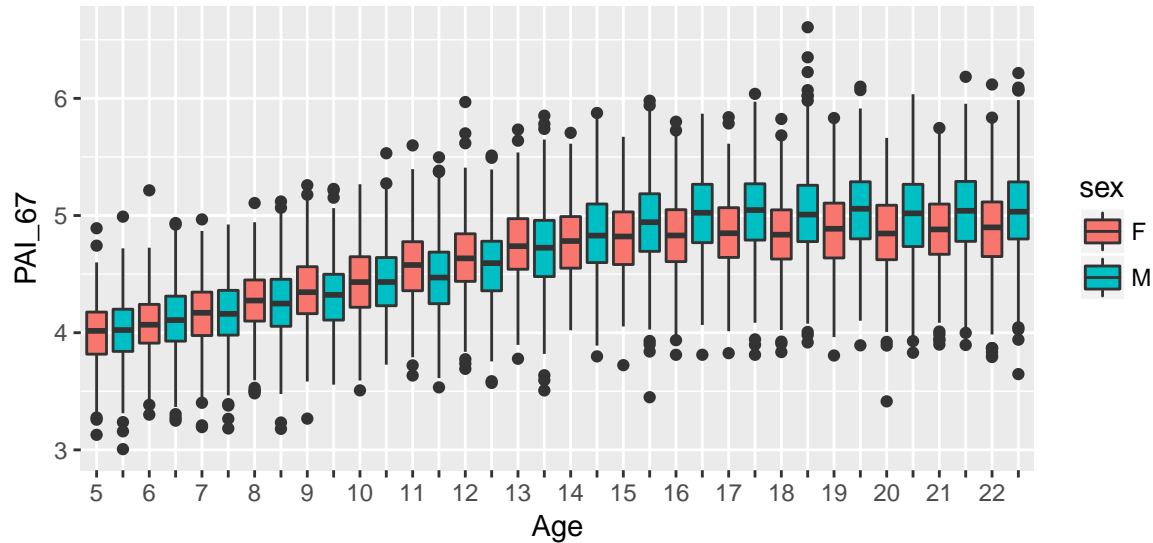

# Distributions of PAI\_68 by Sex and Age

ages from 5 years to 22 years old

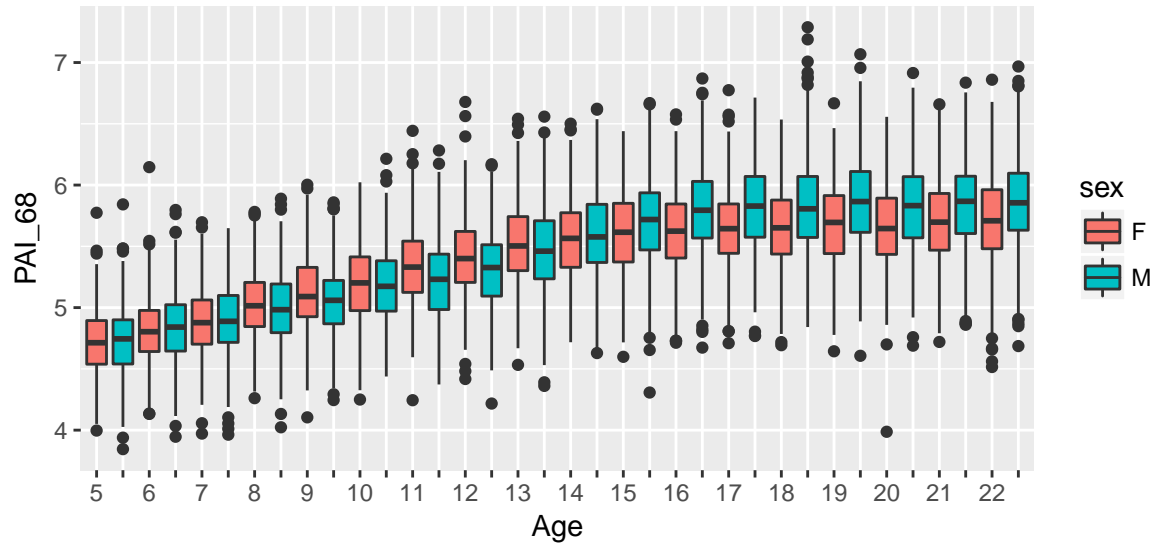

# Distributions of PAI\_69 by Sex and Age

ages from 5 years to 22 years old

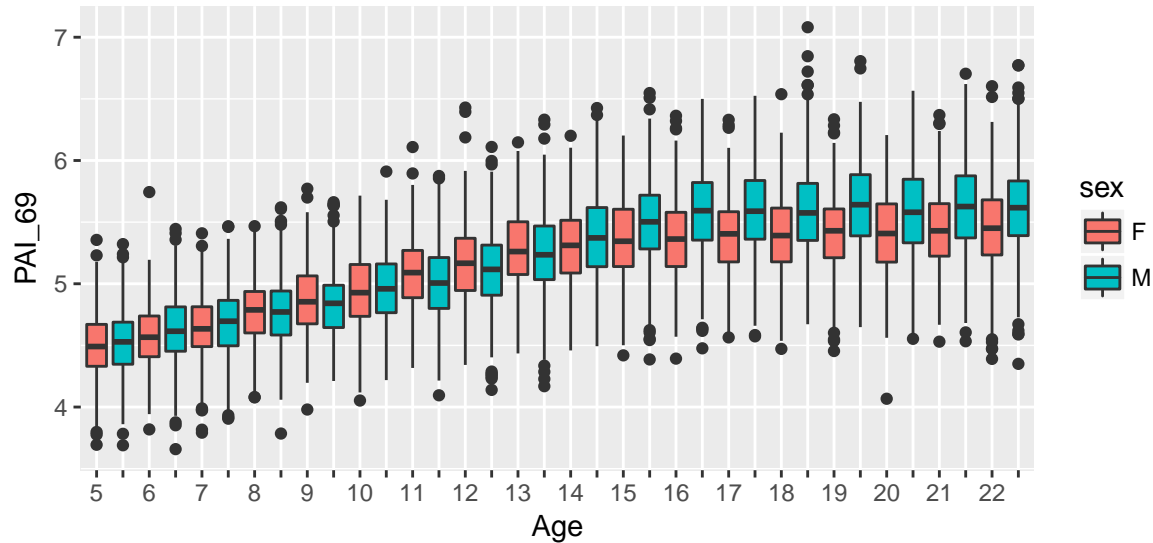

# Distributions of PAI\_6 by Sex and Age

ages from 5 years to 22 years old

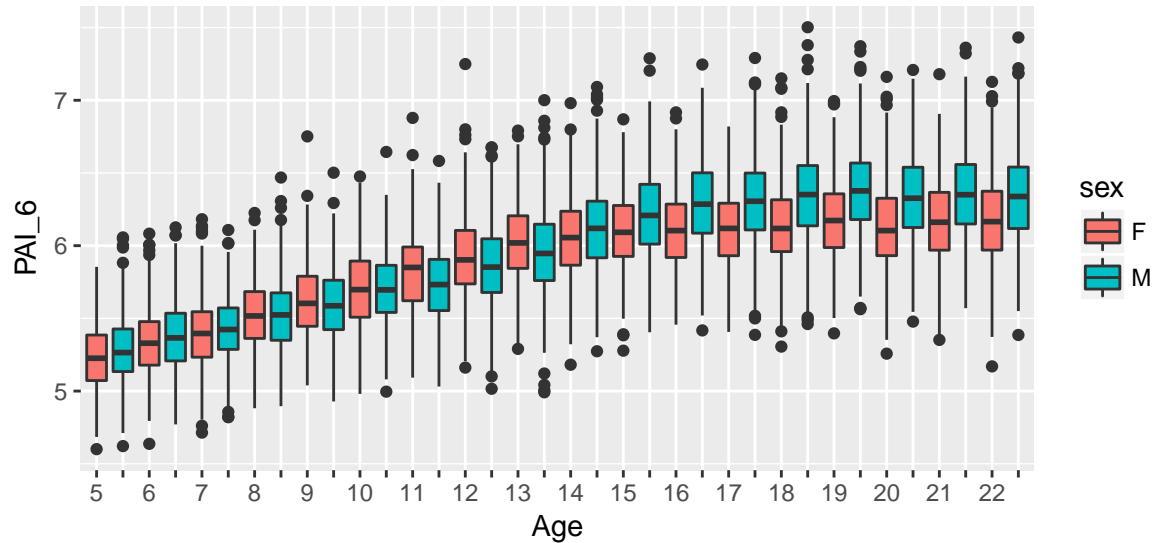

# Distributions of PAI\_70 by Sex and Age

ages from 5 years to 22 years old

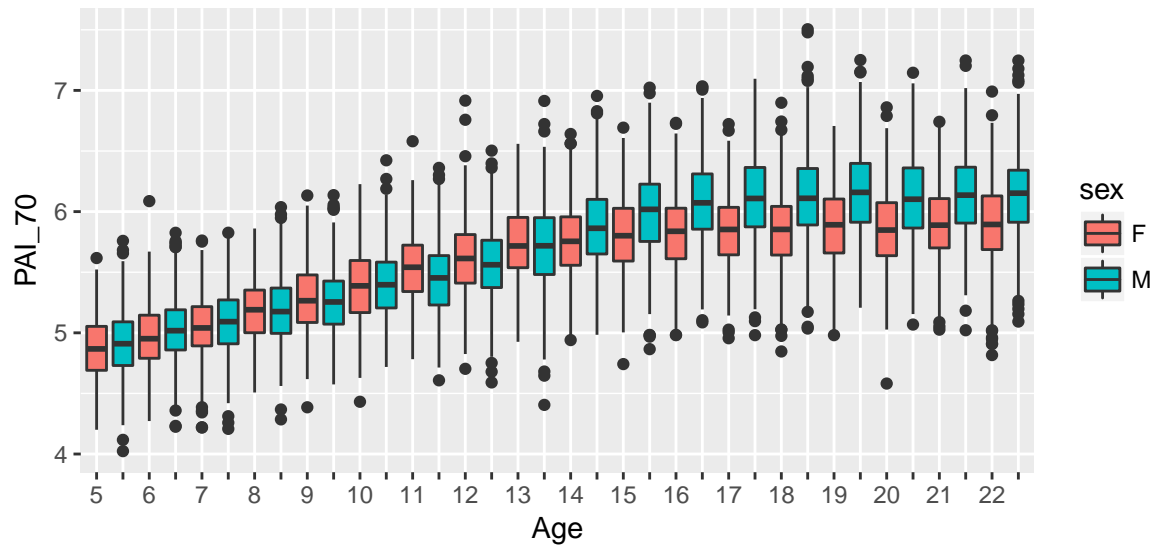

# Distributions of PAI\_71 by Sex and Age

ages from 5 years to 22 years old

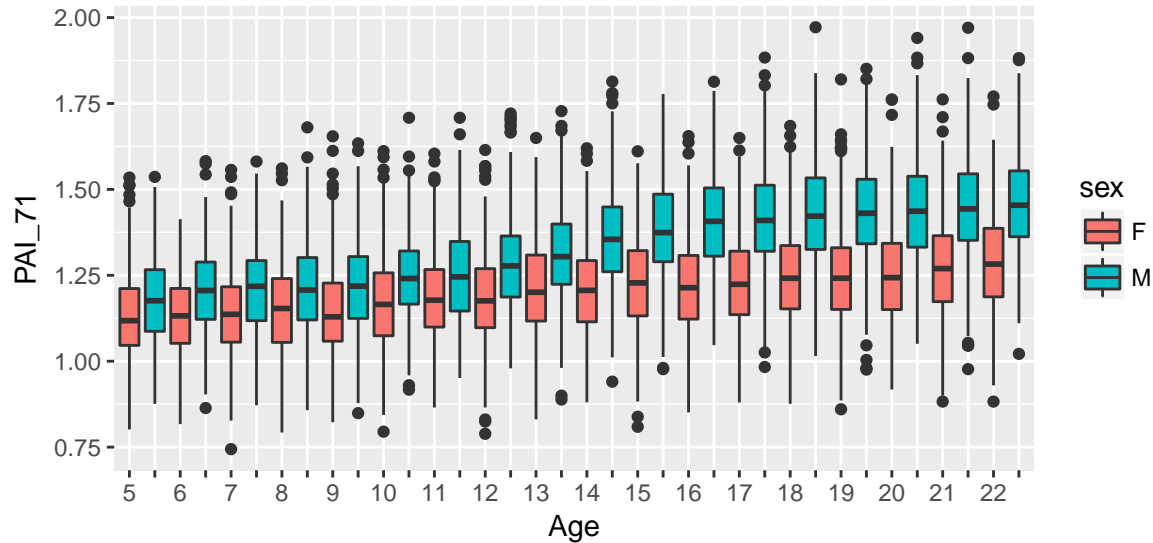

# Distributions of PAI\_72 by Sex and Age

ages from 5 years to 22 years old

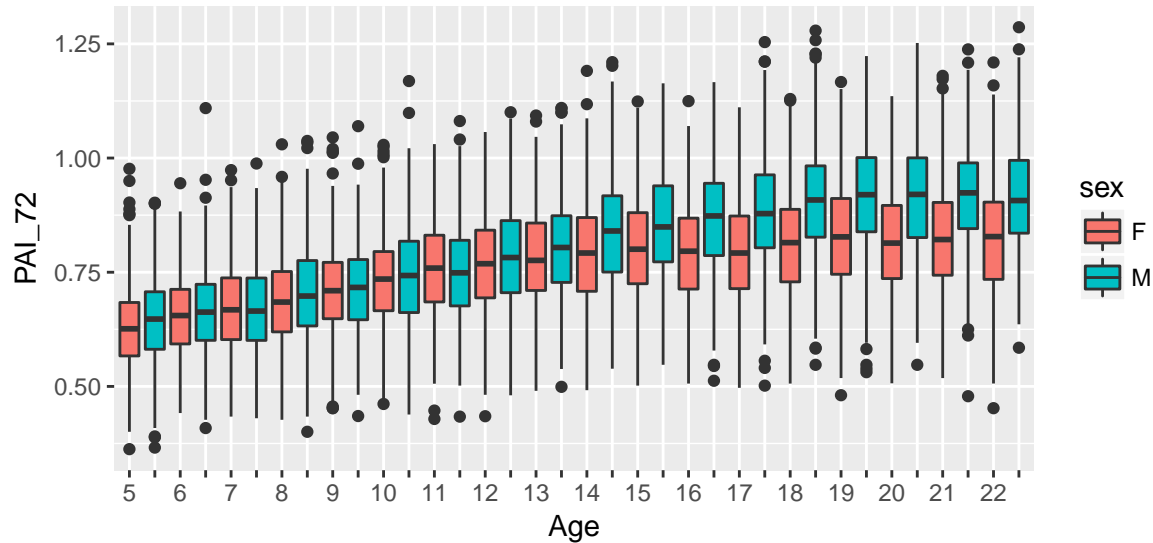

# Distributions of PAI\_73 by Sex and Age

ages from 5 years to 22 years old

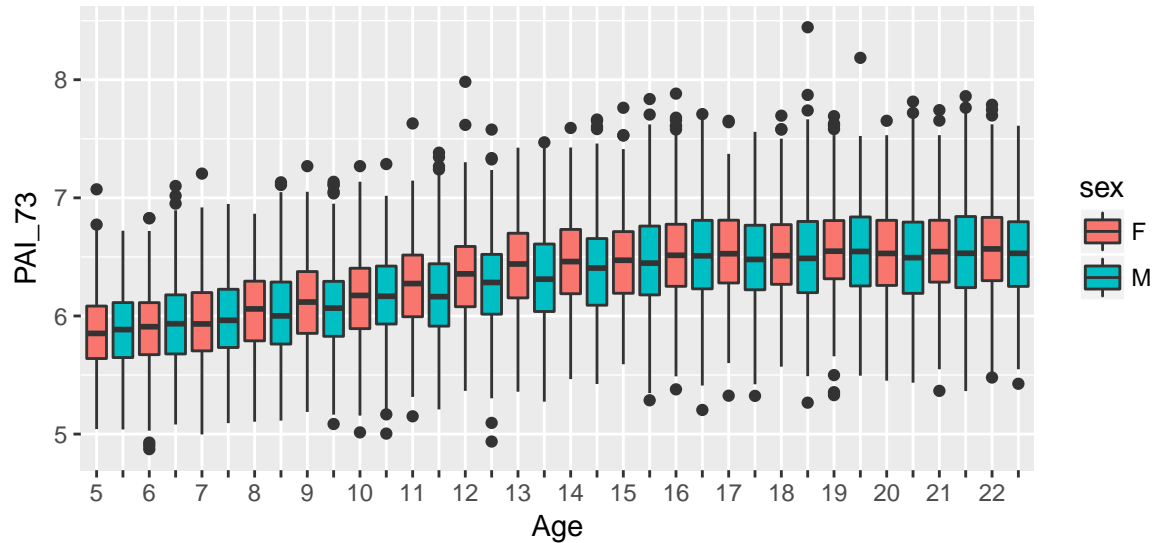

# Distributions of PAI\_74 by Sex and Age

ages from 5 years to 22 years old

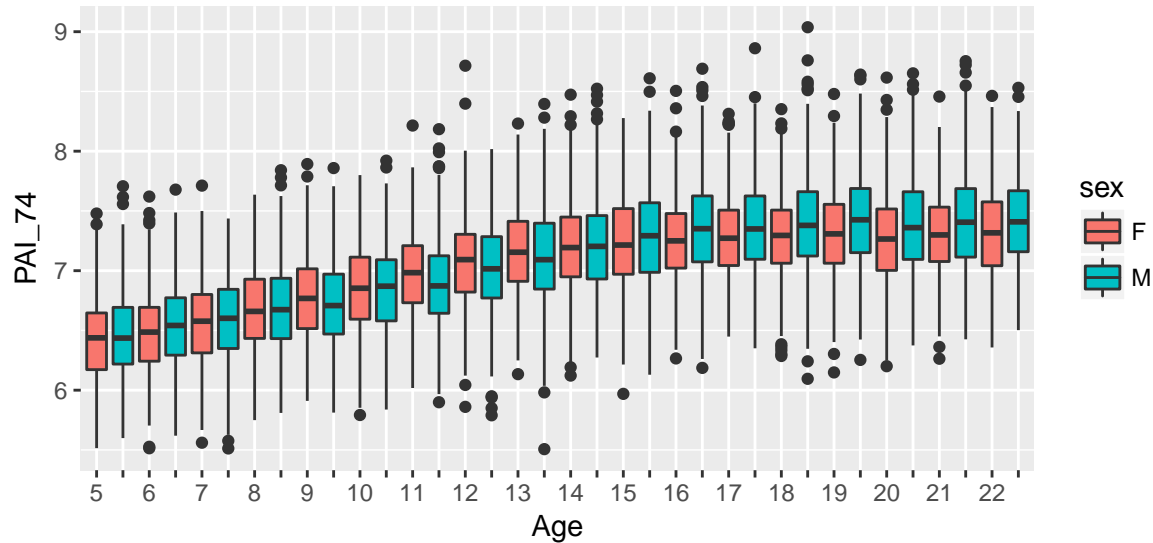

# Distributions of PAI\_75 by Sex and Age

ages from 5 years to 22 years old

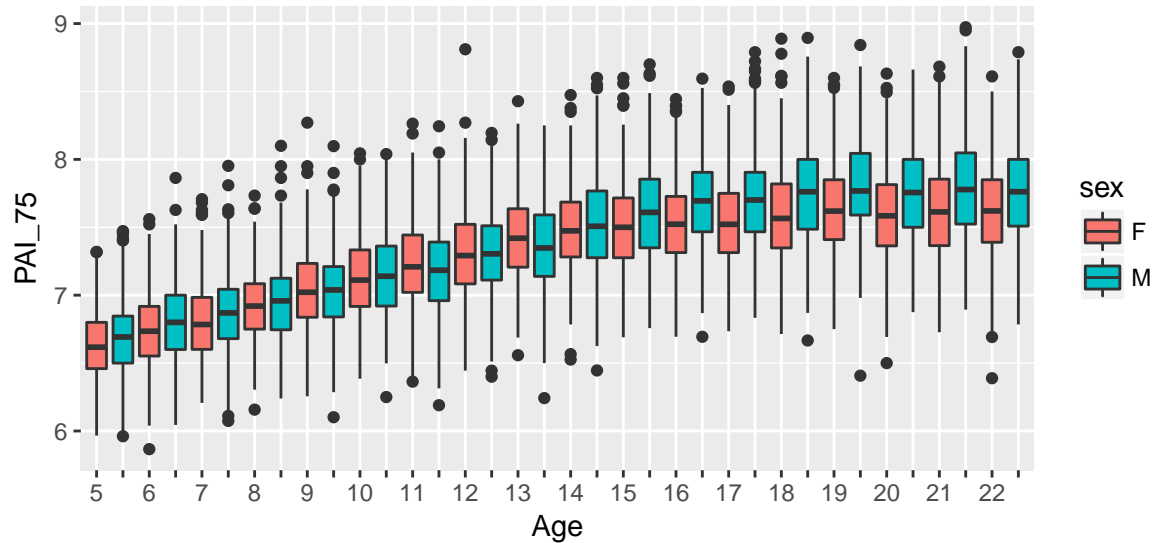

# Distributions of PAI\_76 by Sex and Age

ages from 5 years to 22 years old

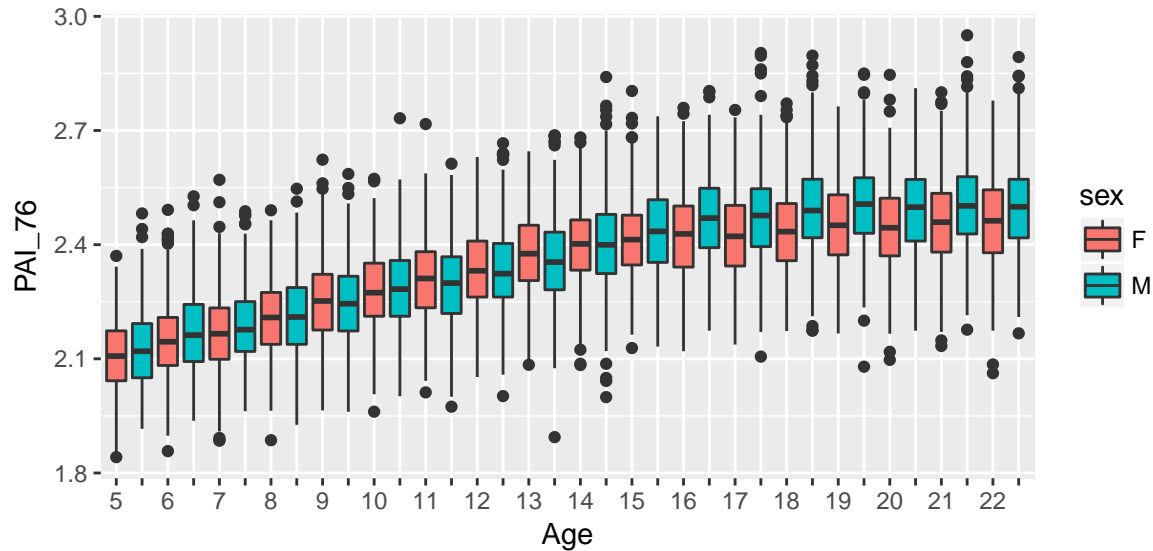

# Distributions of PAI\_77 by Sex and Age

ages from 5 years to 22 years old

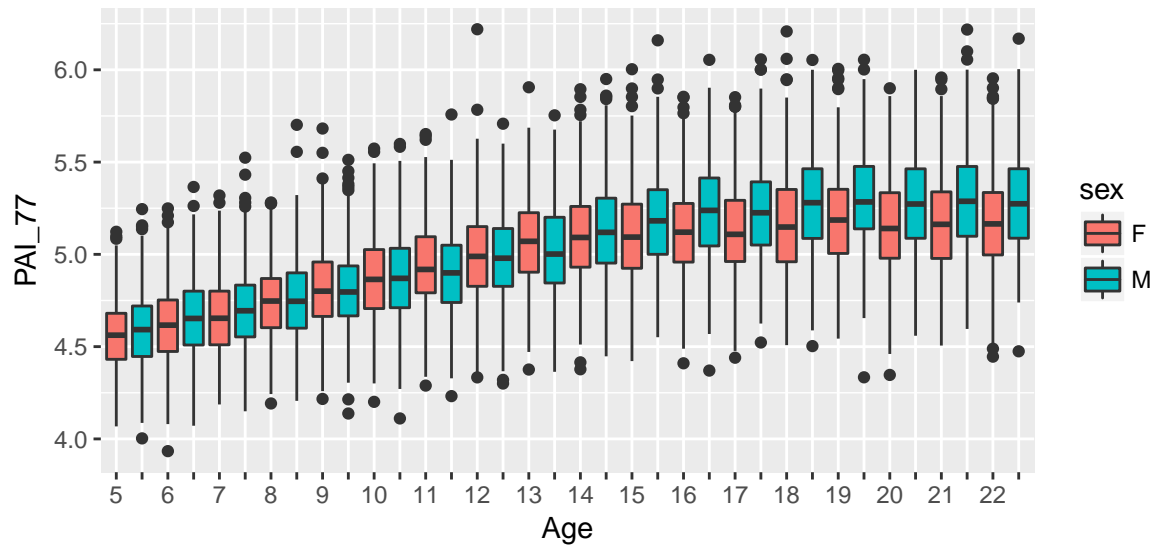

# Distributions of PAI\_78 by Sex and Age

ages from 5 years to 22 years old

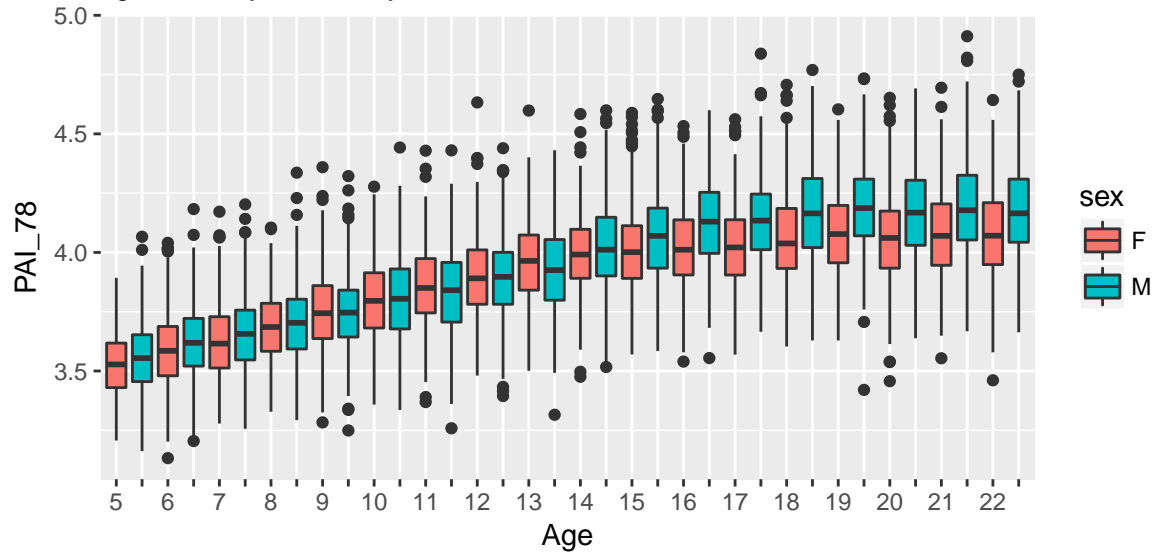

# Distributions of PAI\_79 by Sex and Age

ages from 5 years to 22 years old

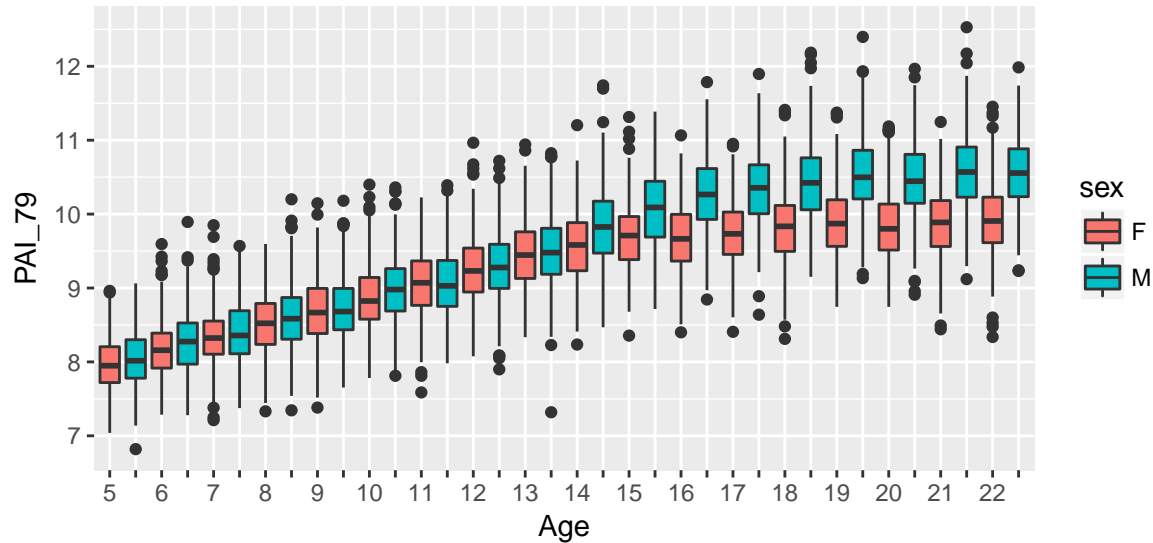

# Distributions of PAI\_7 by Sex and Age

ages from 5 years to 22 years old

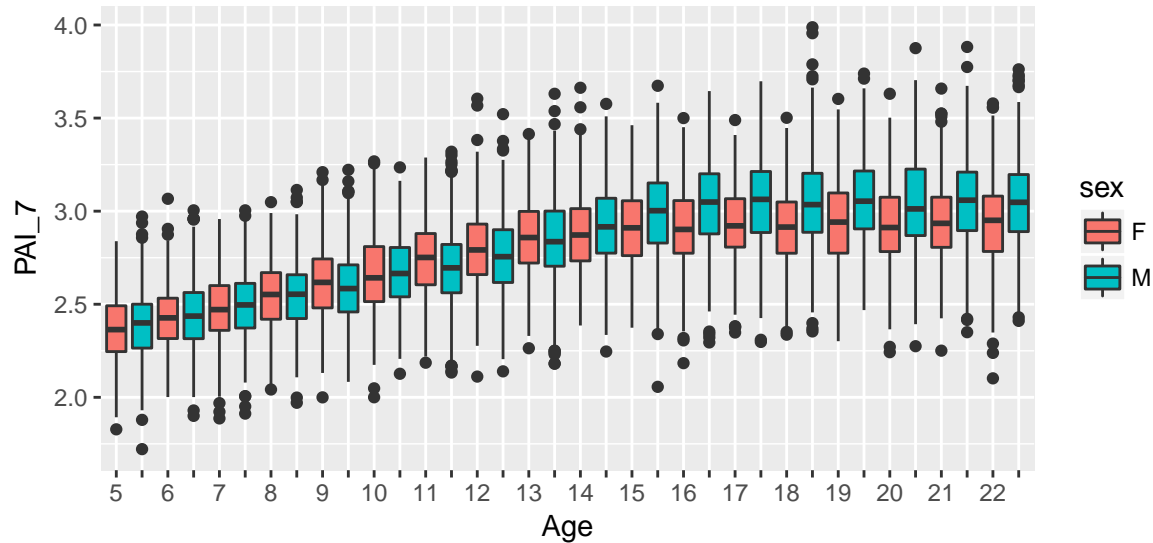

# Distributions of PAI\_80 by Sex and Age

ages from 5 years to 22 years old

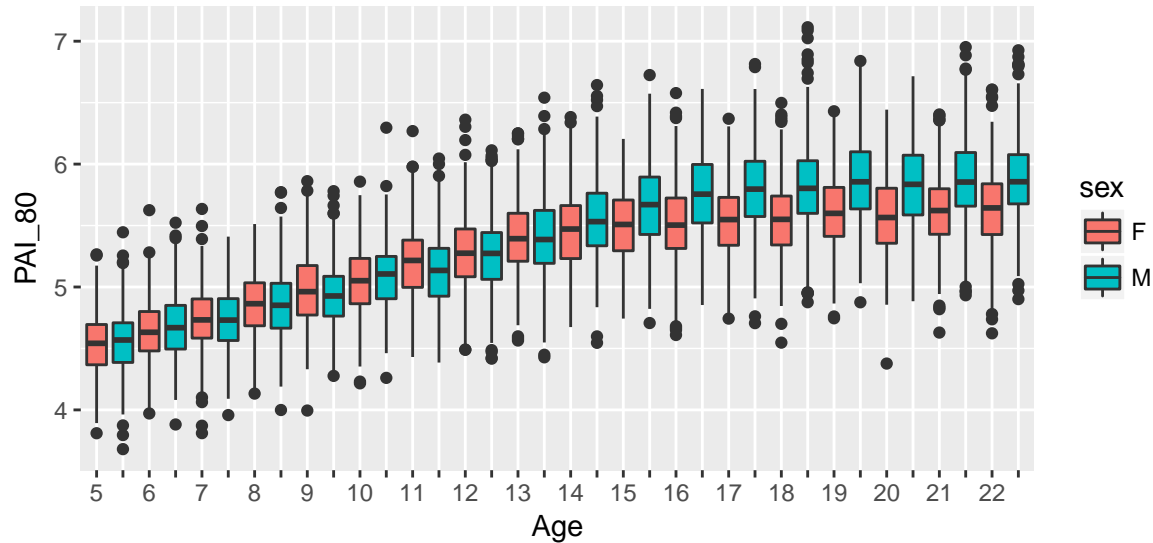

# Distributions of PAI\_81 by Sex and Age

ages from 5 years to 22 years old

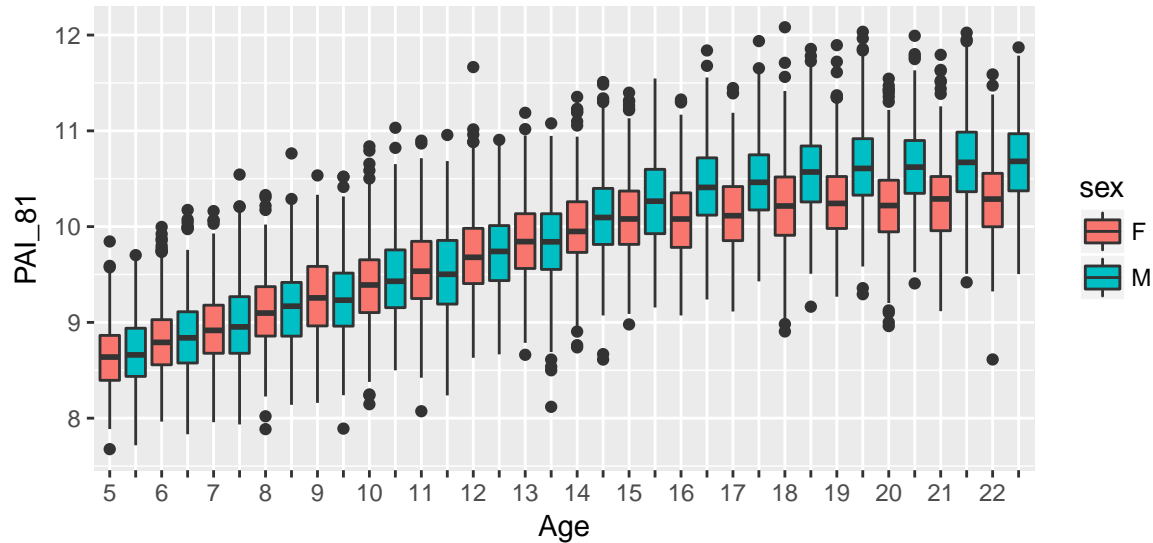

# Distributions of PAI\_82 by Sex and Age

ages from 5 years to 22 years old

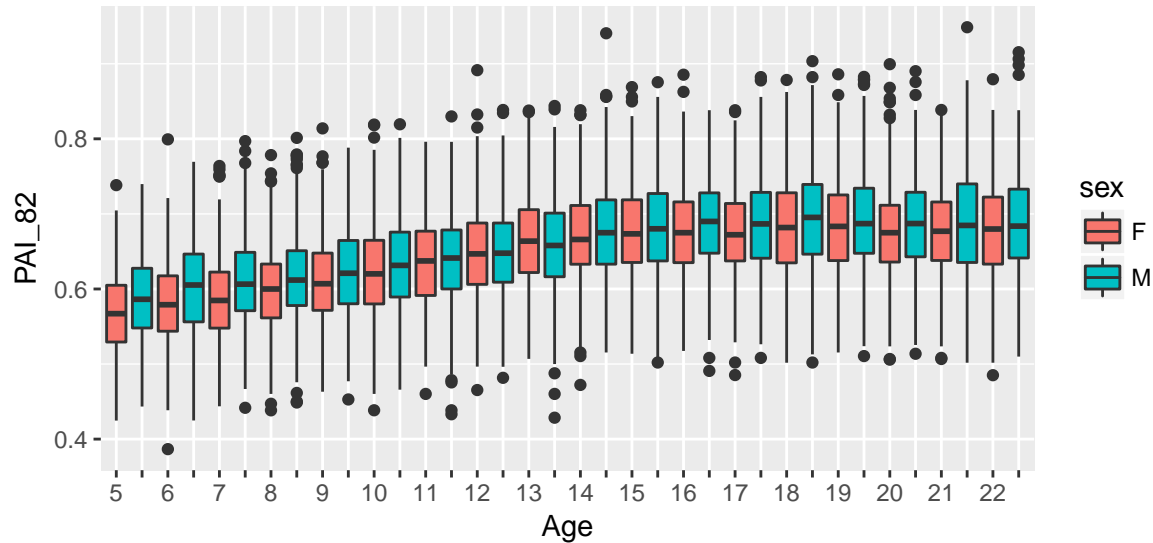

# Distributions of PAI\_83 by Sex and Age

ages from 5 years to 22 years old

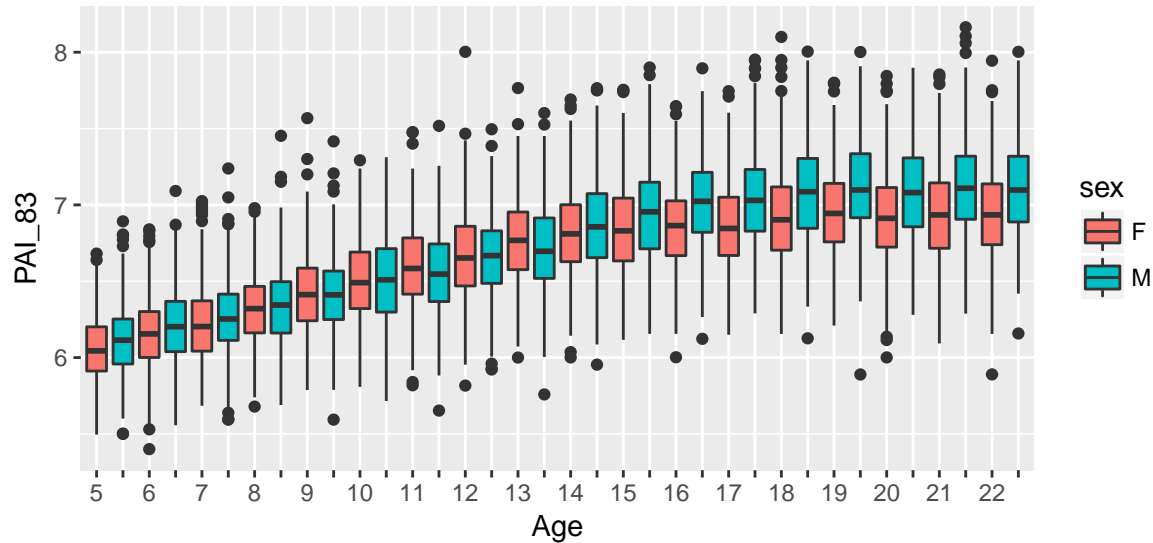

# Distributions of PAI\_84 by Sex and Age

ages from 5 years to 22 years old

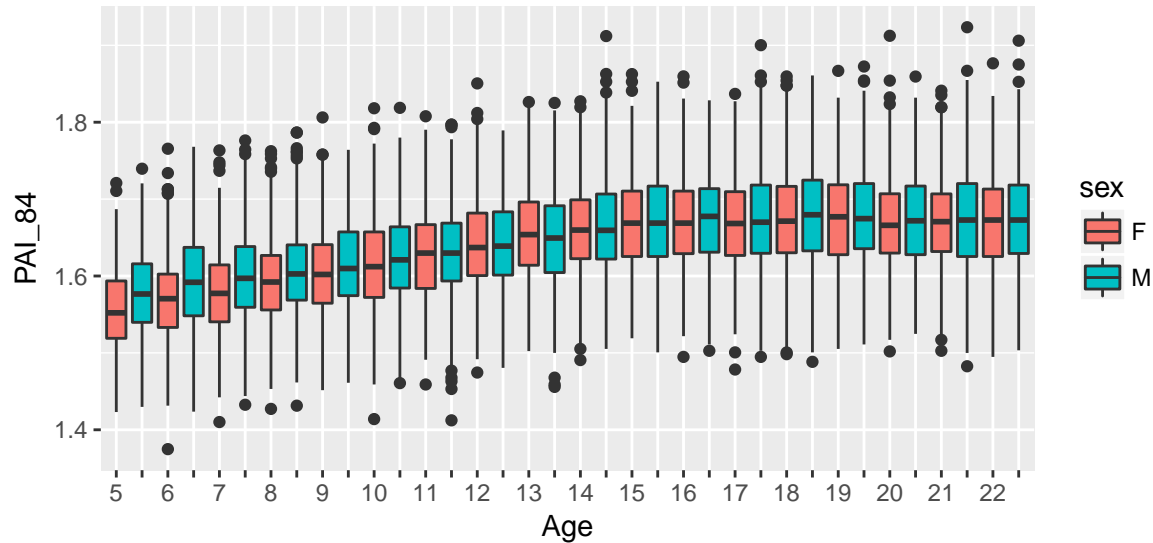

# Distributions of PAI\_85 by Sex and Age

ages from 5 years to 22 years old

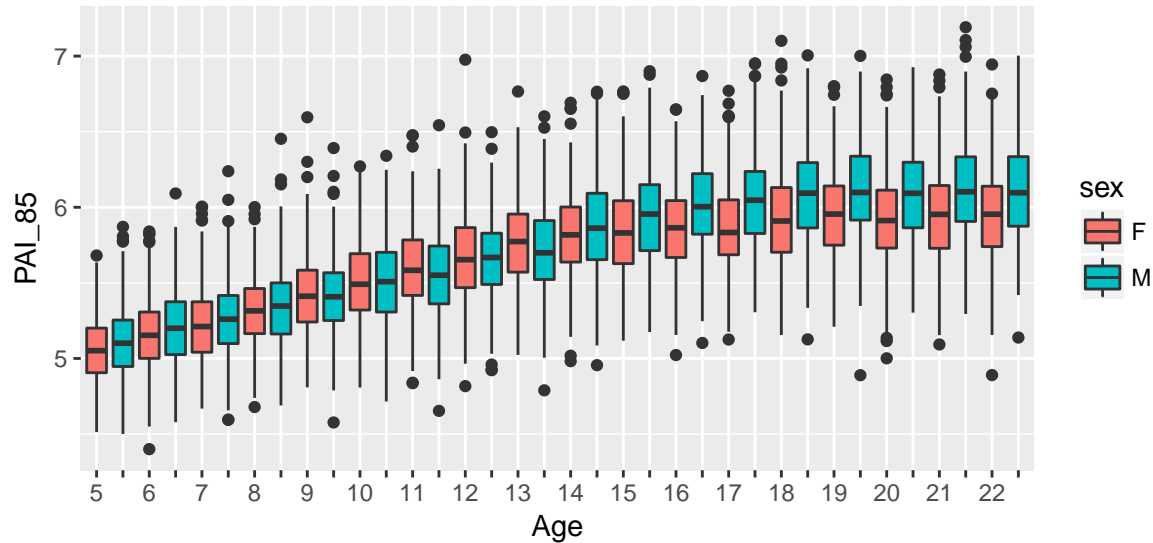

# Distributions of PAI\_86 by Sex and Age

ages from 5 years to 22 years old

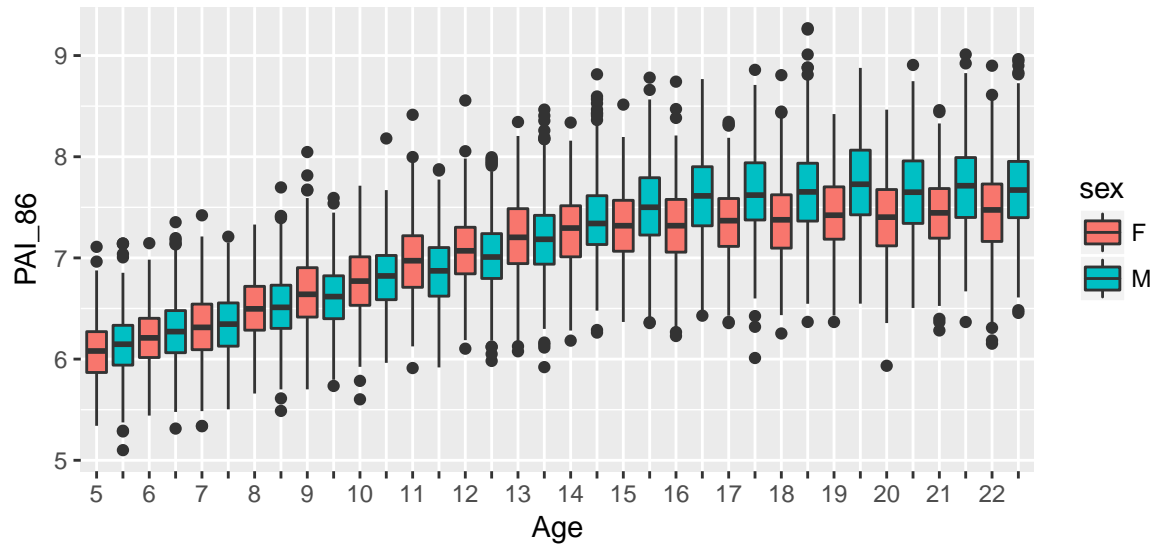

# Distributions of PAI\_87 by Sex and Age

ages from 5 years to 22 years old

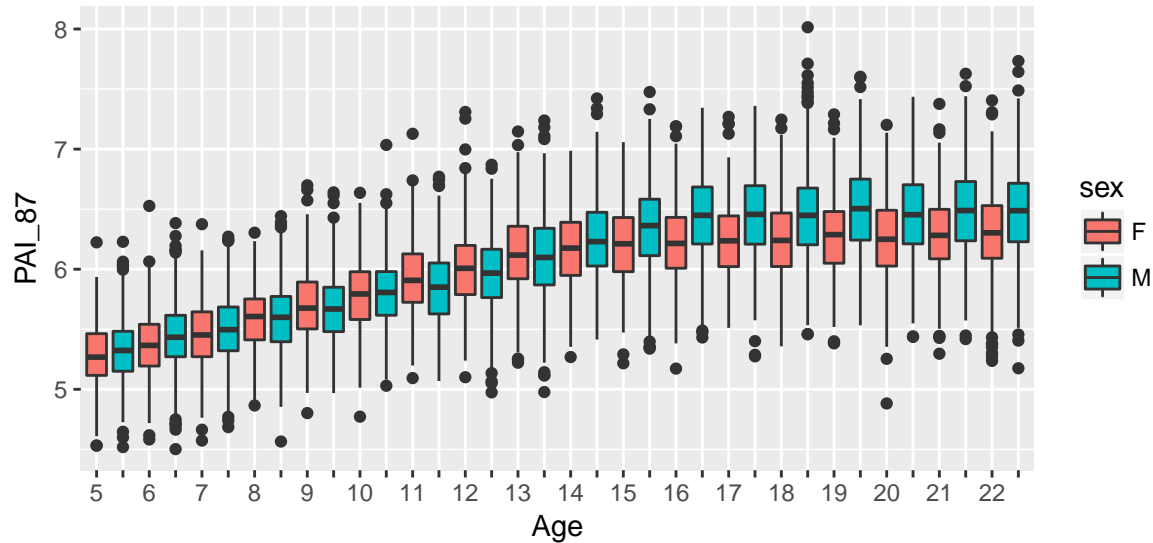

# Distributions of PAI\_88 by Sex and Age

ages from 5 years to 22 years old

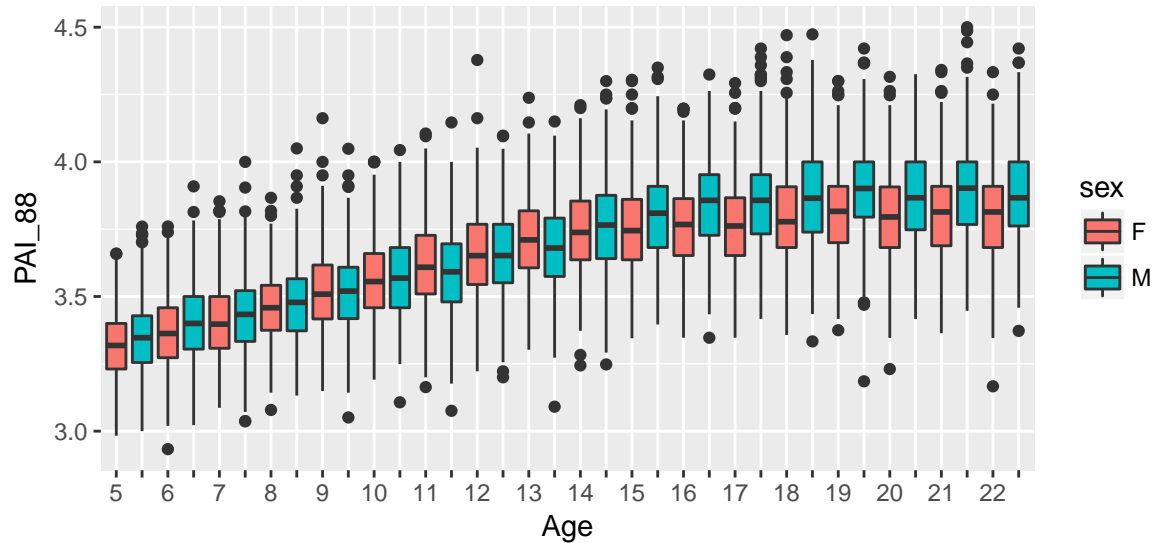

# Distributions of PAI\_89 by Sex and Age

ages from 5 years to 22 years old

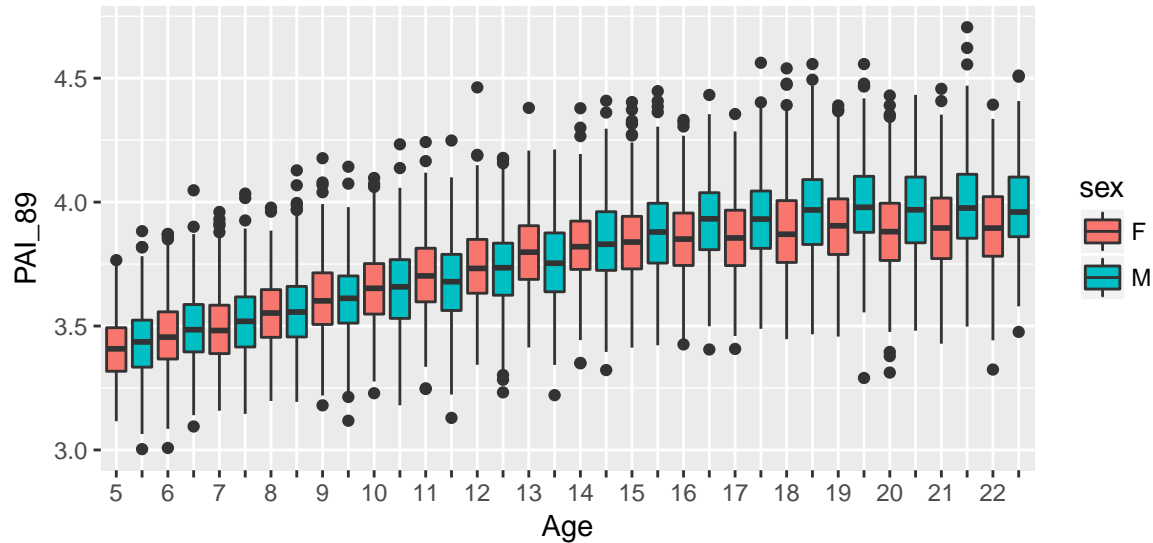

# Distributions of PAI\_8 by Sex and Age

ages from 5 years to 22 years old

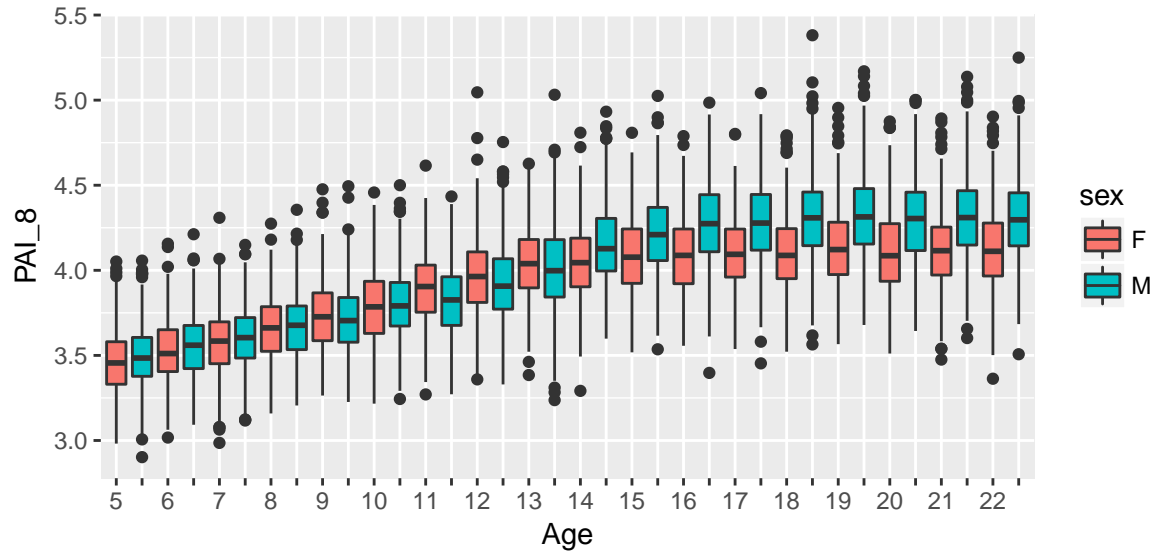

# Distributions of PAI\_90 by Sex and Age

ages from 5 years to 22 years old

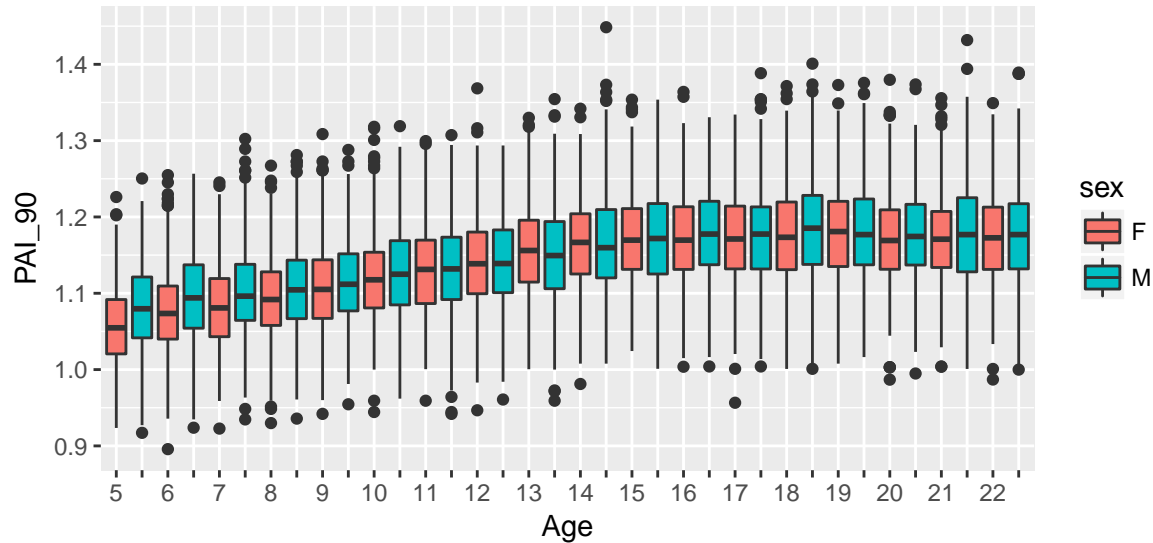

# Distributions of PAI\_91 by Sex and Age

ages from 5 years to 22 years old

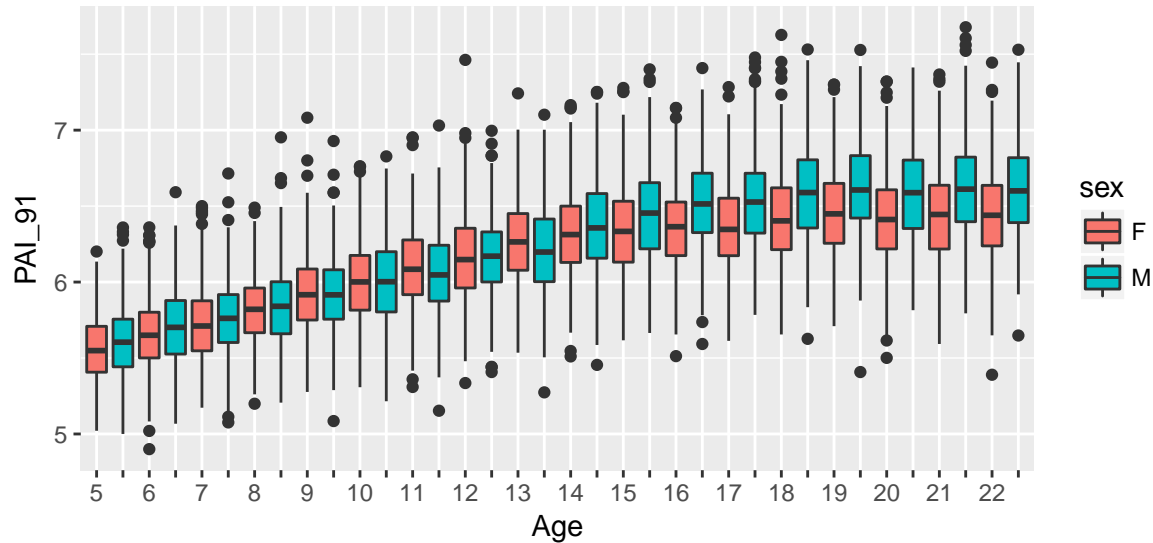

# Distributions of PAI\_92 by Sex and Age

ages from 5 years to 22 years old

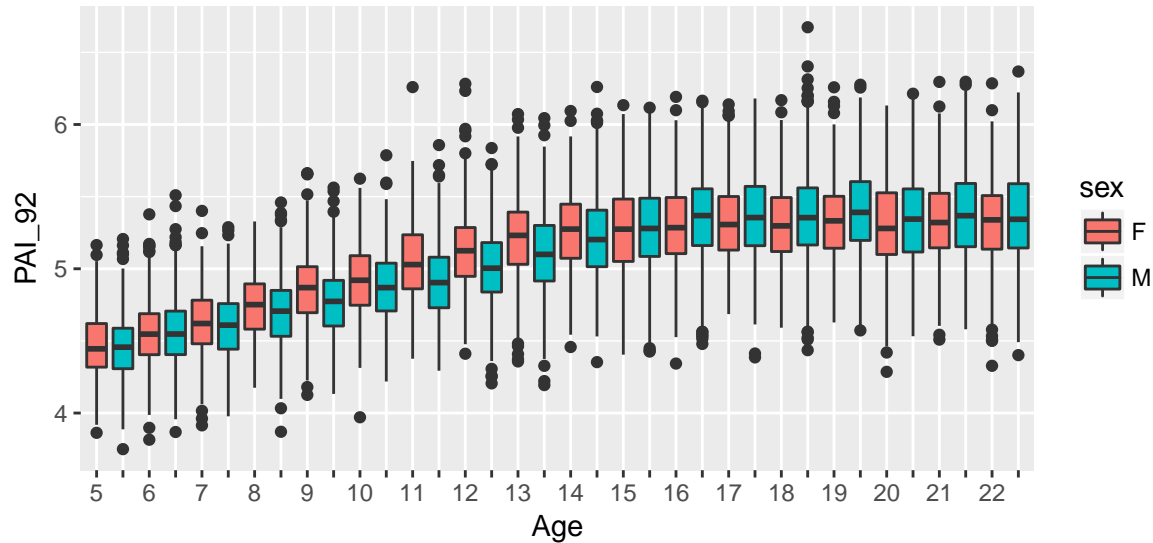

# Distributions of PAI\_93 by Sex and Age

ages from 5 years to 22 years old

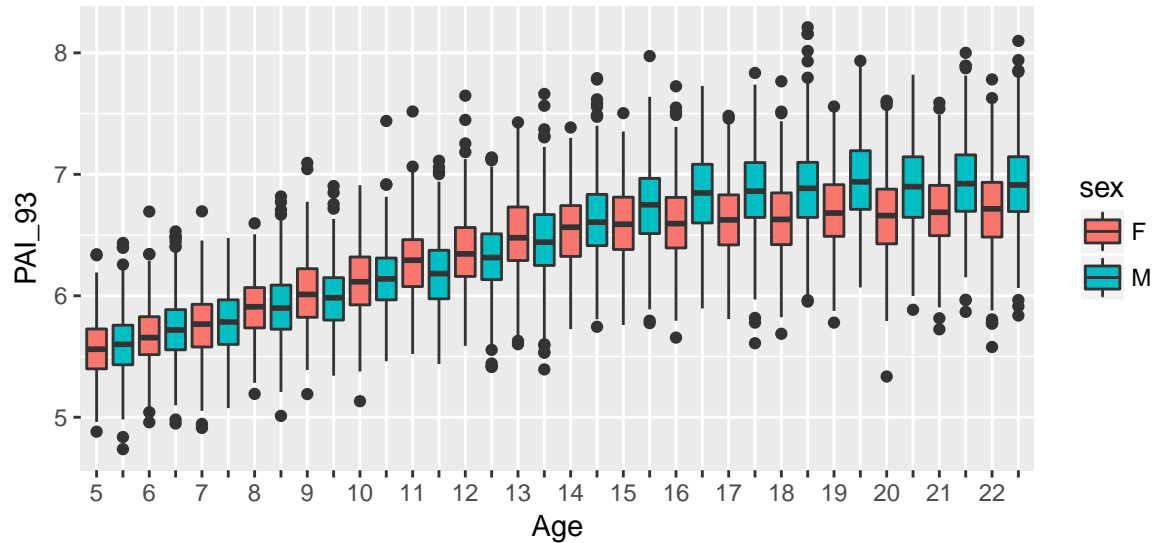

# Distributions of PAI\_94 by Sex and Age

ages from 5 years to 22 years old

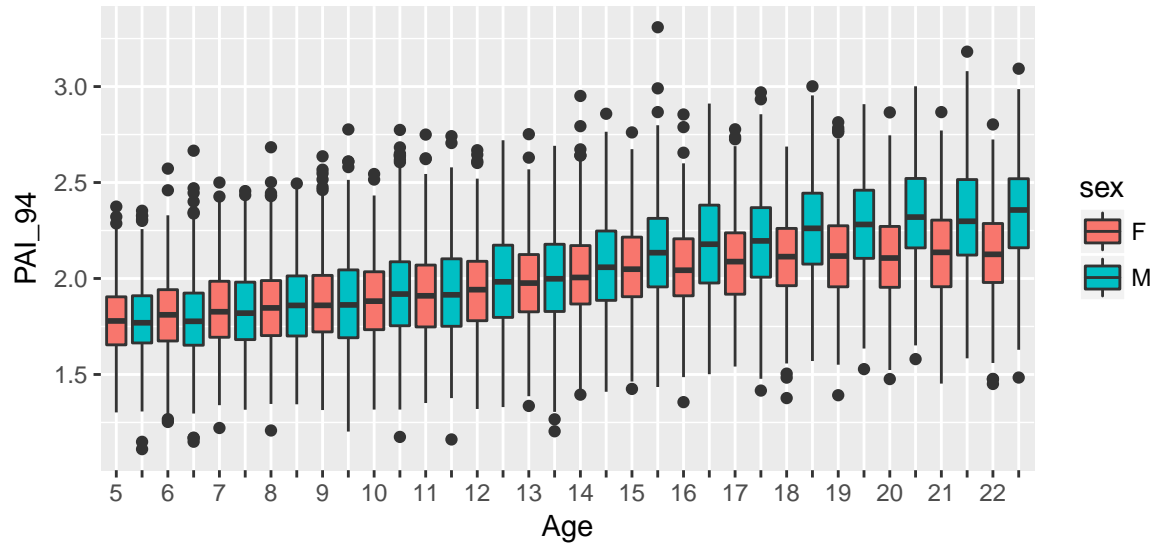

# Distributions of PAI\_95 by Sex and Age

ages from 5 years to 22 years old

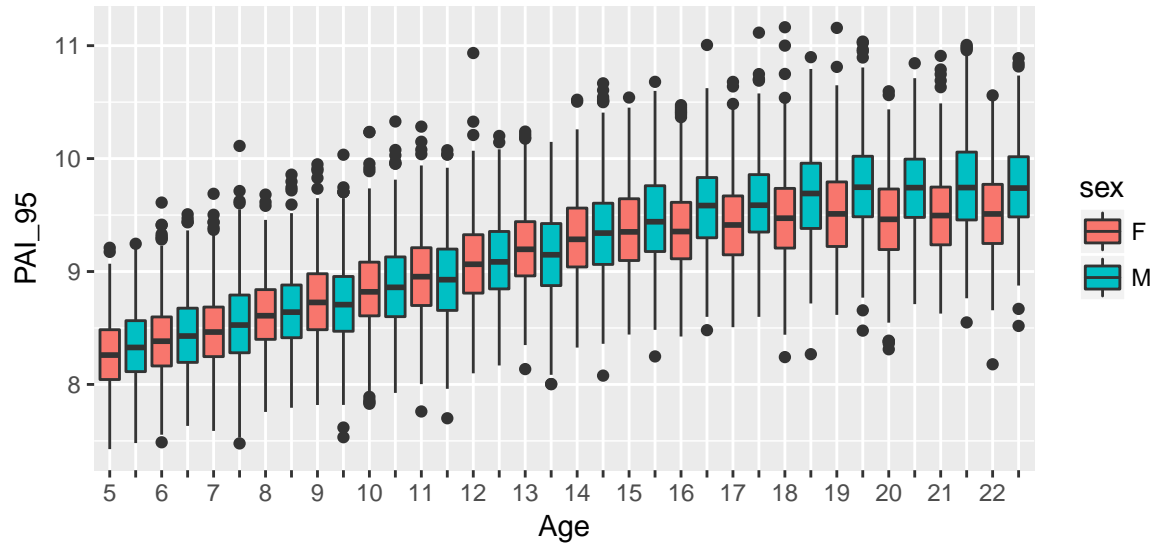

# Distributions of PAI\_96 by Sex and Age

ages from 5 years to 22 years old

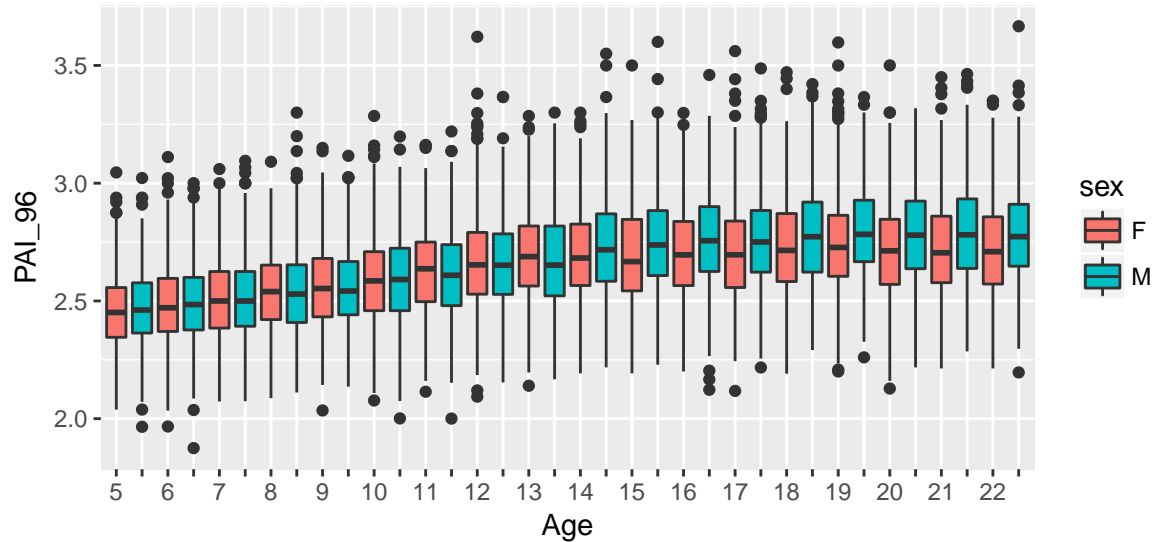

# Distributions of PAI\_97 by Sex and Age

ages from 5 years to 22 years old

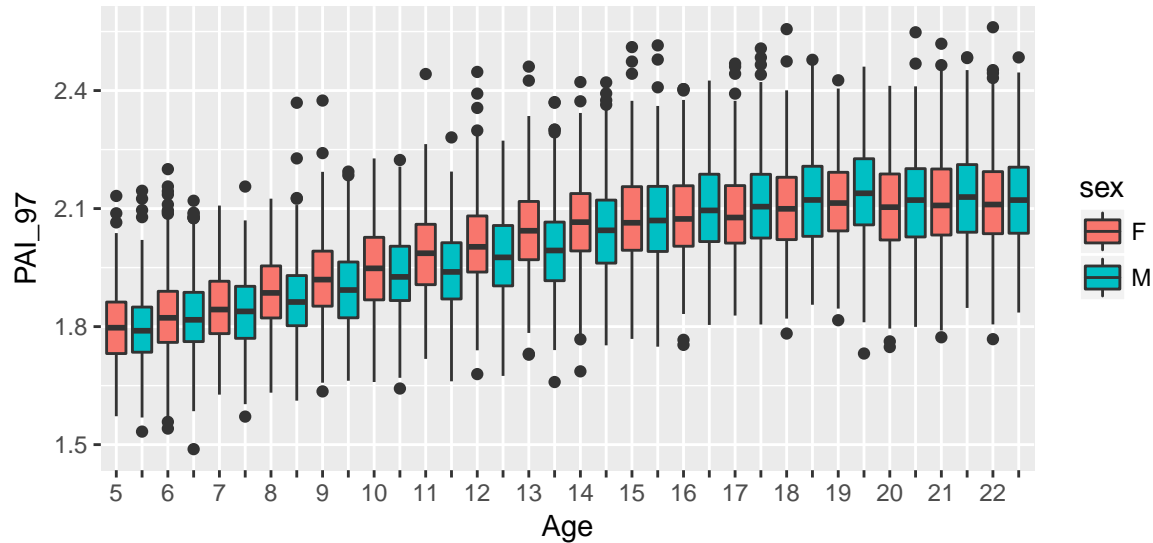

# Distributions of PAI\_98 by Sex and Age

ages from 5 years to 22 years old

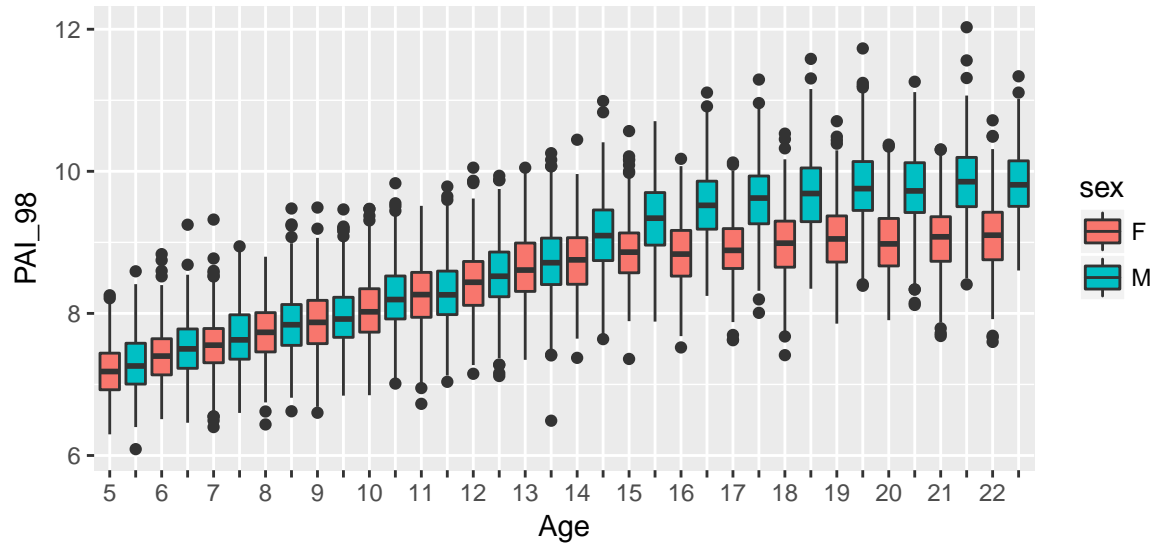

# Distributions of PAI\_99 by Sex and Age

ages from 5 years to 22 years old

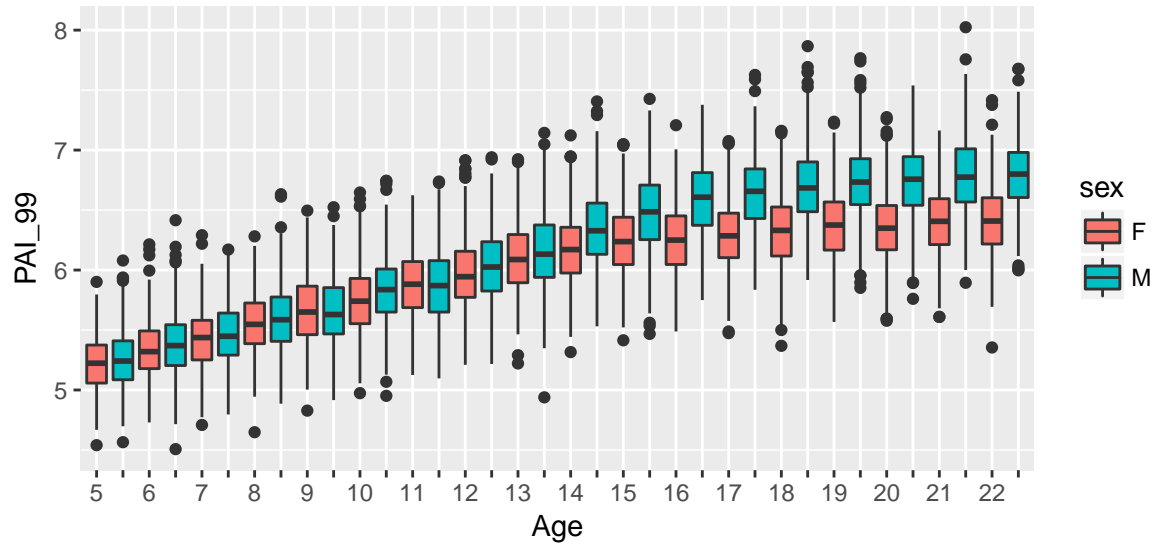

# Distributions of PAI\_9 by Sex and Age

ages from 5 years to 22 years old

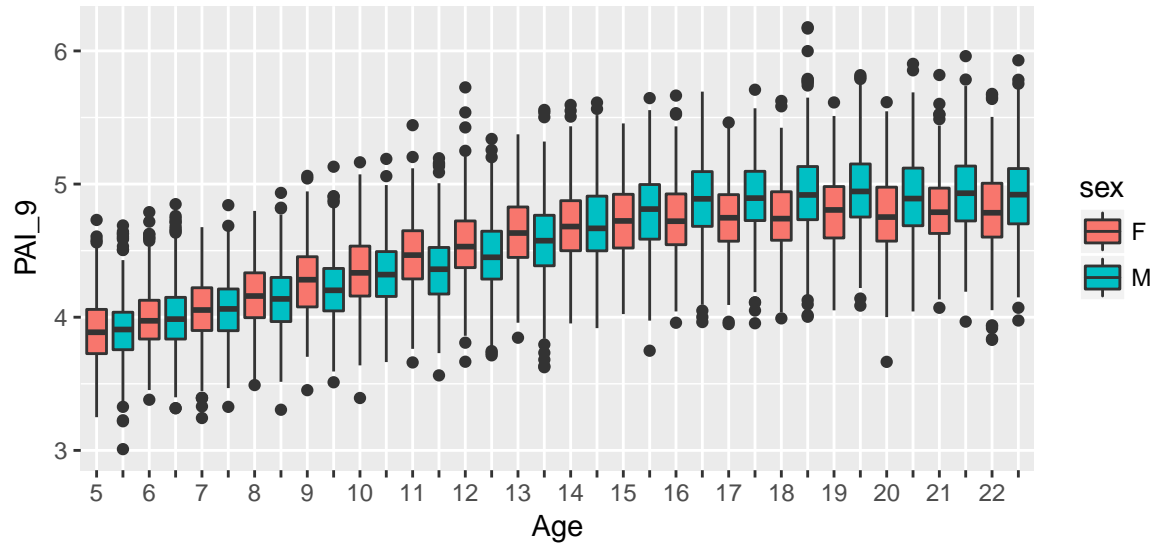

Supplement: Supplementary file 1 [file PAIs_sex_age_boxplots_supplemental.pdf]
